# Supplementary material for: A factorisation-aware Matrix element emulator
Source: arXiv:2107.06625 ancillary file (2021-10-29)

Trajectory 1234

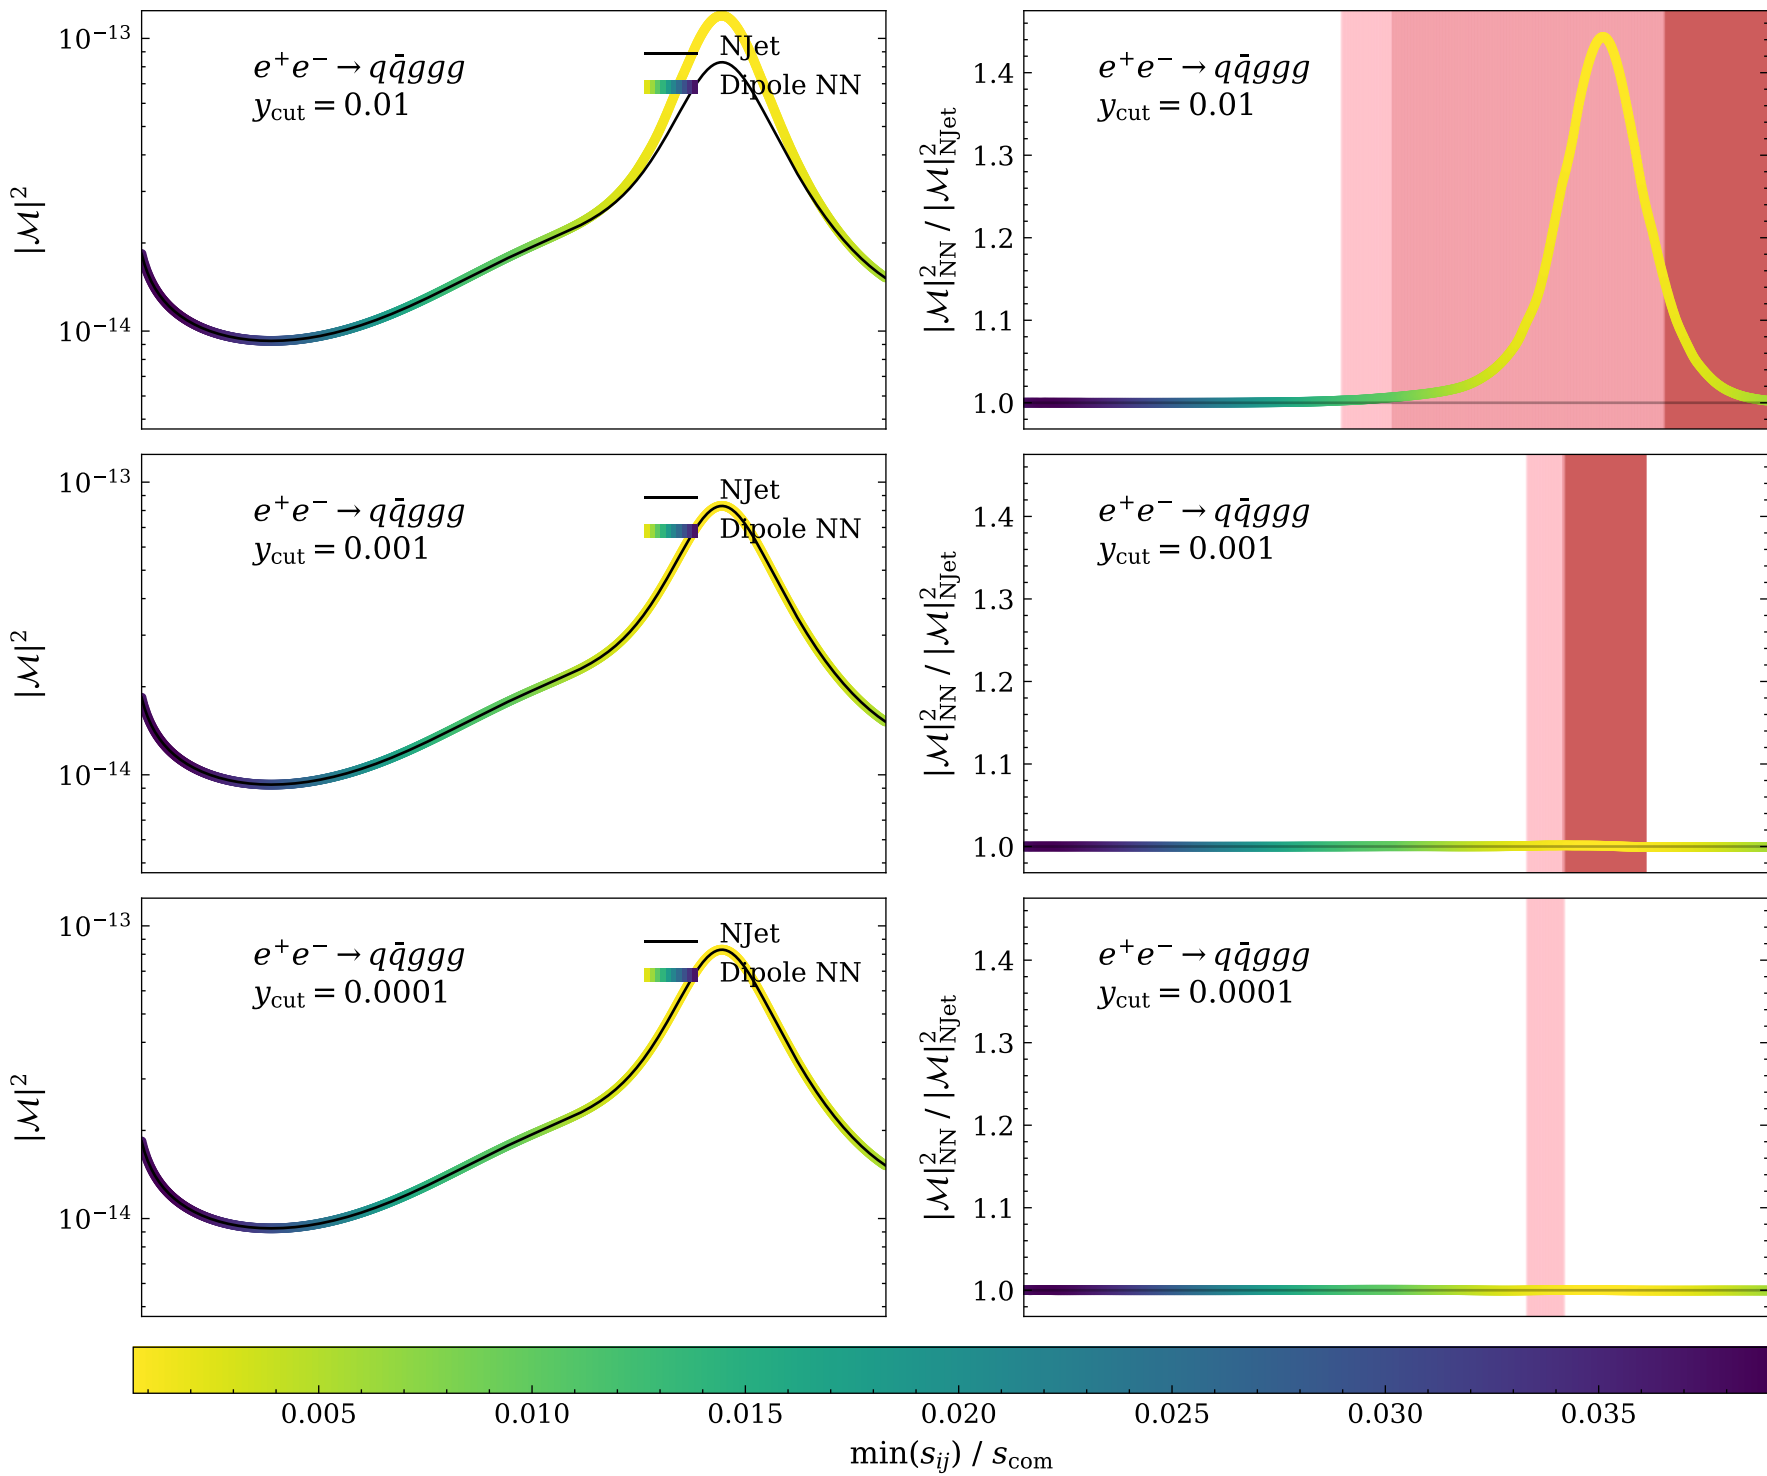

Trajectory 1235

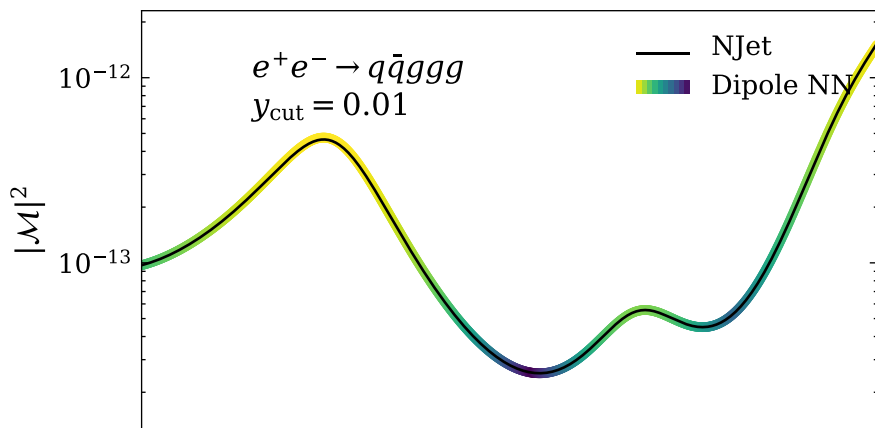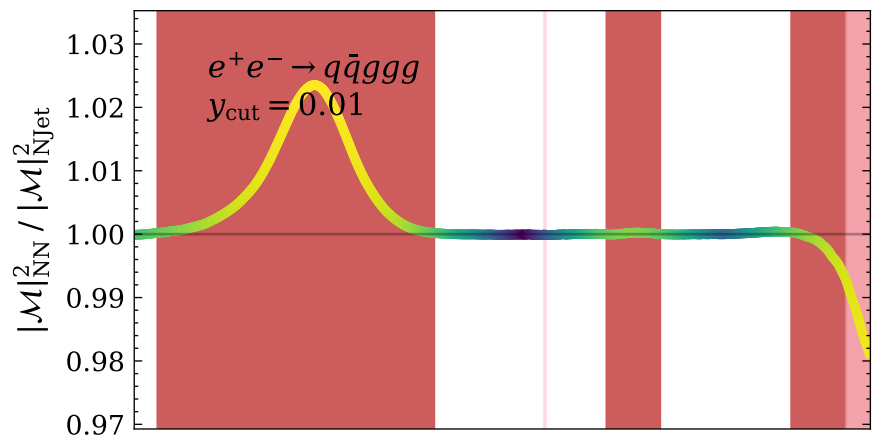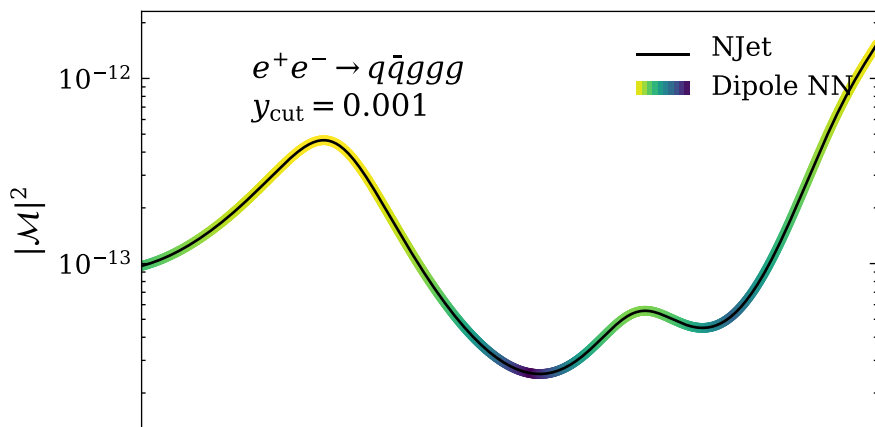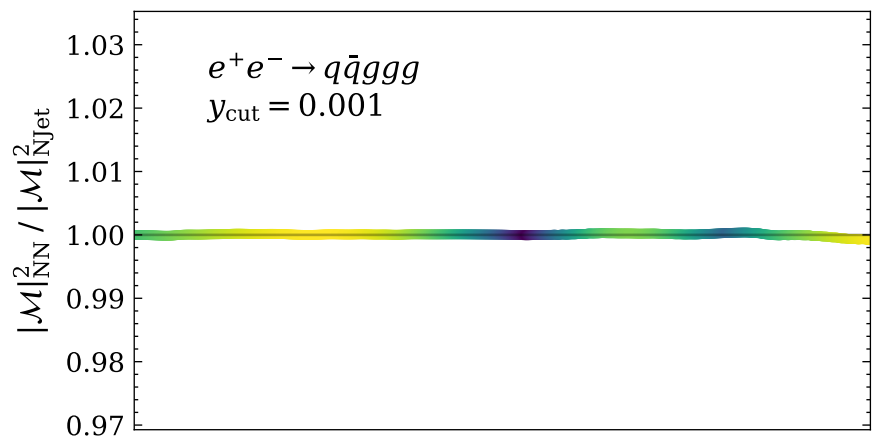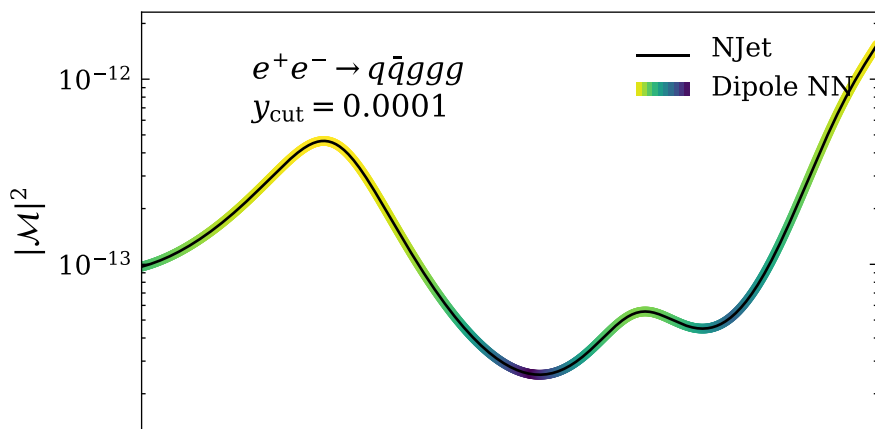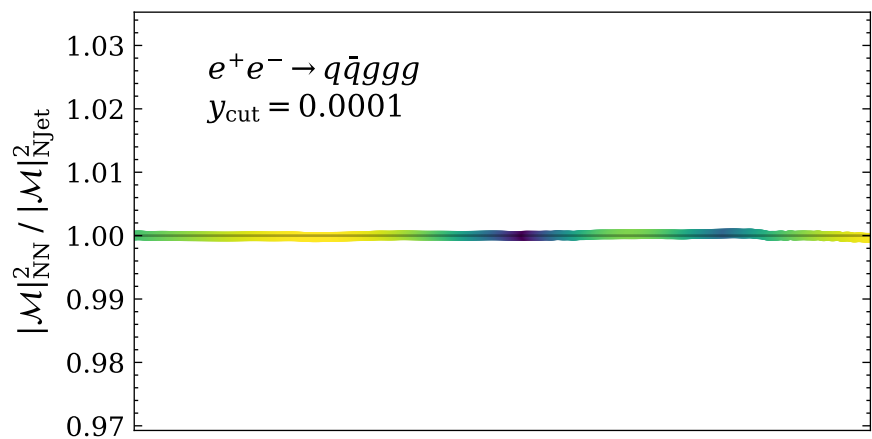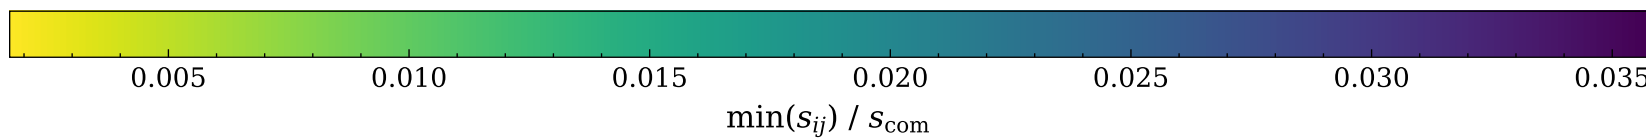

Trajectory 1236

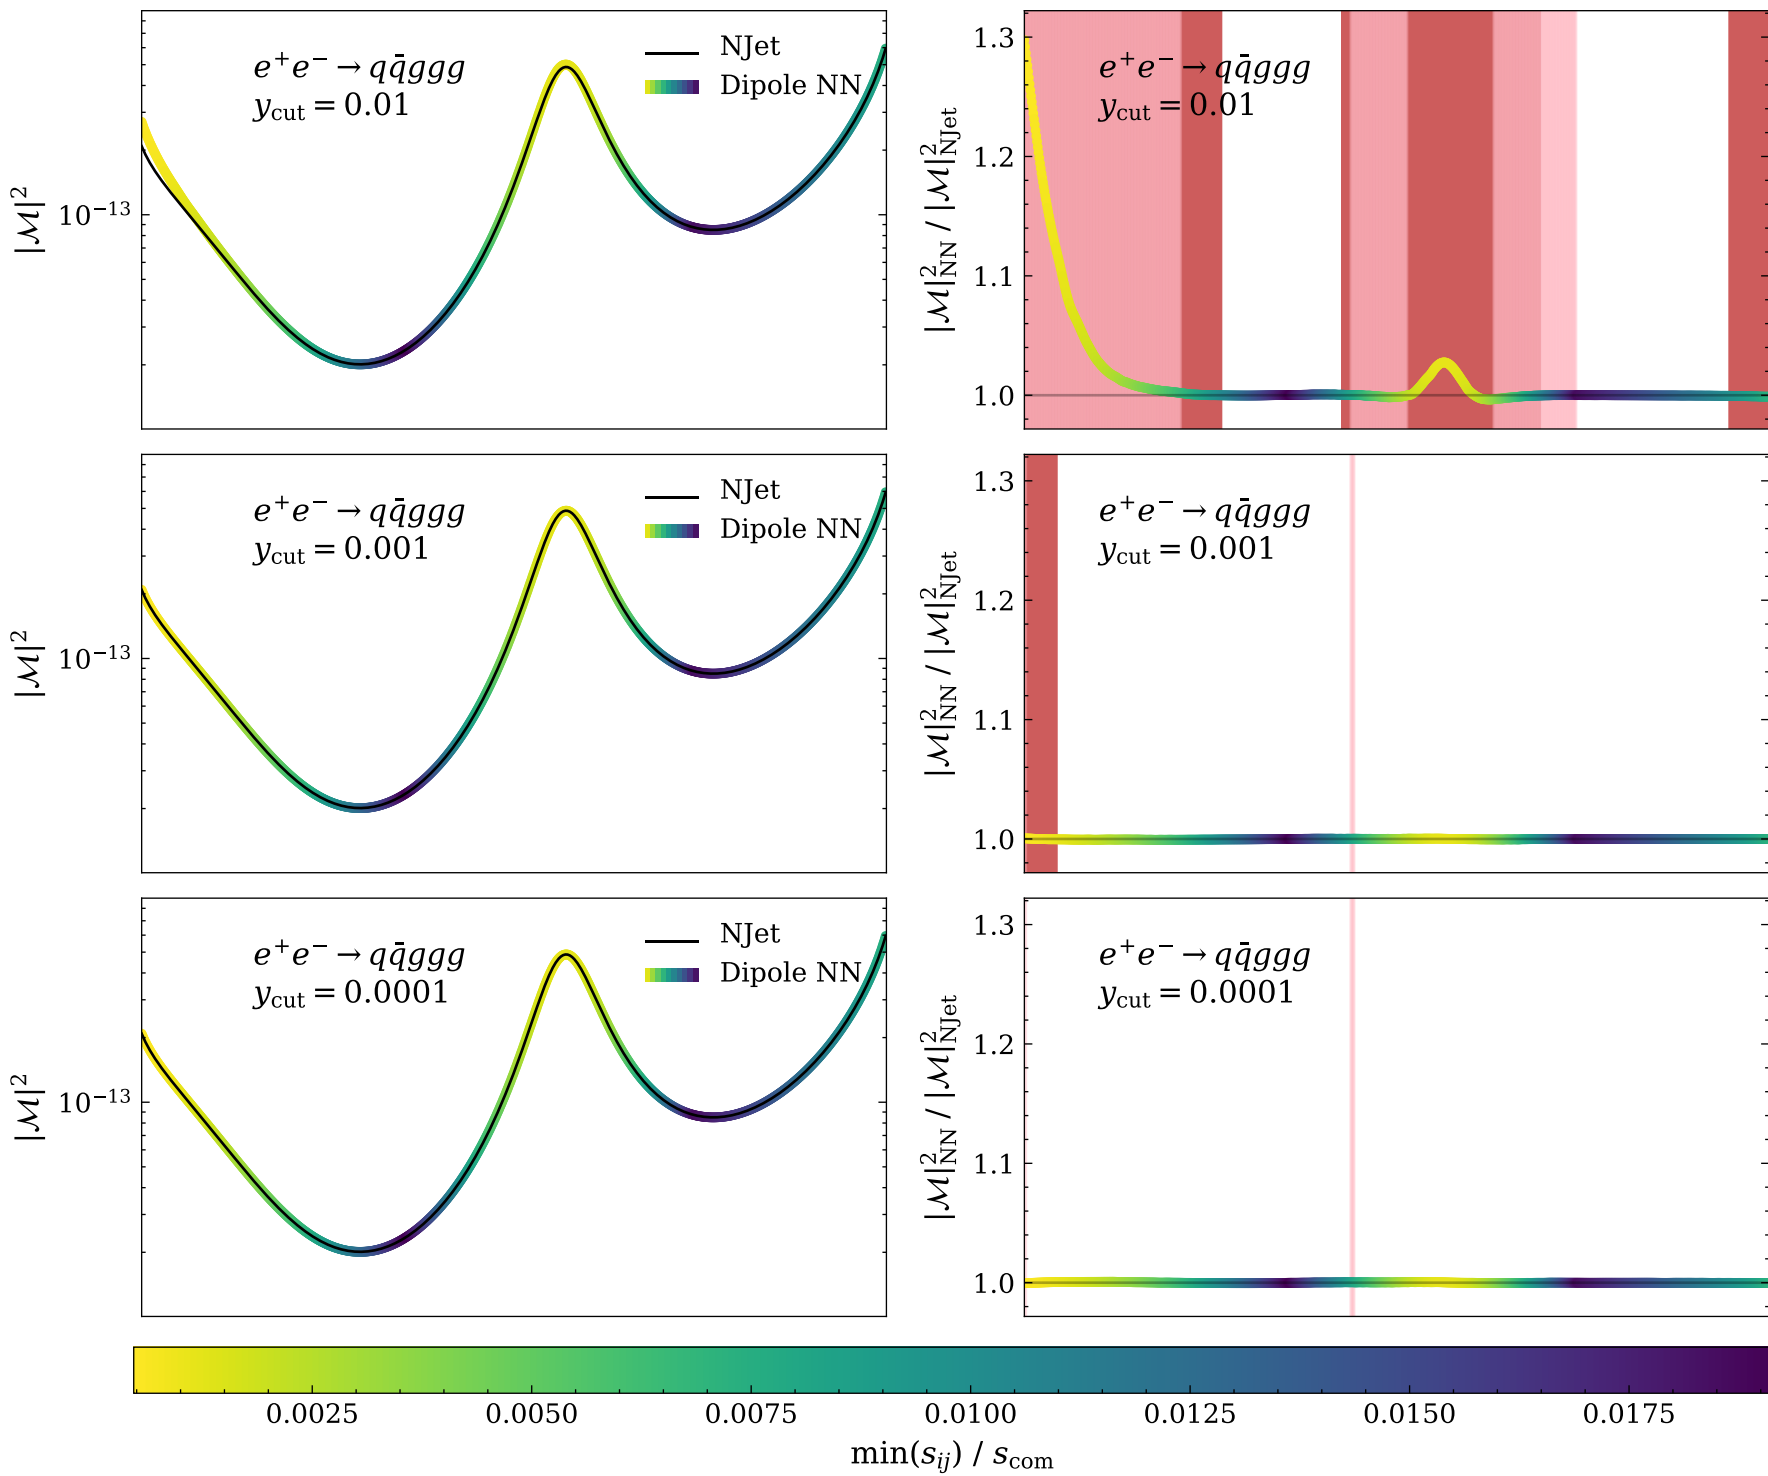

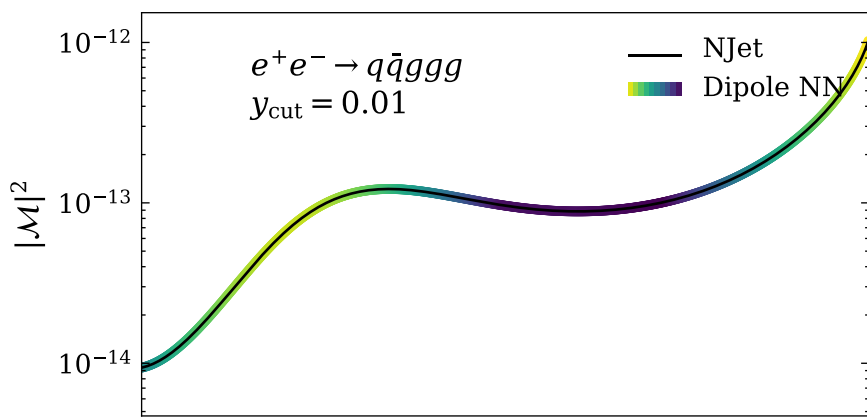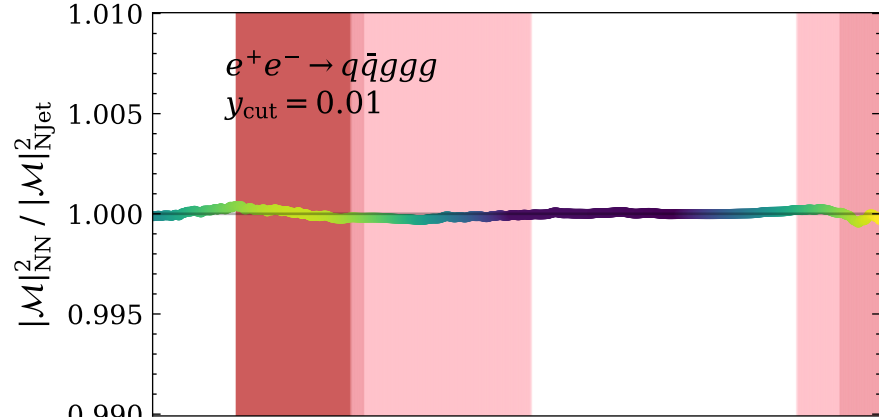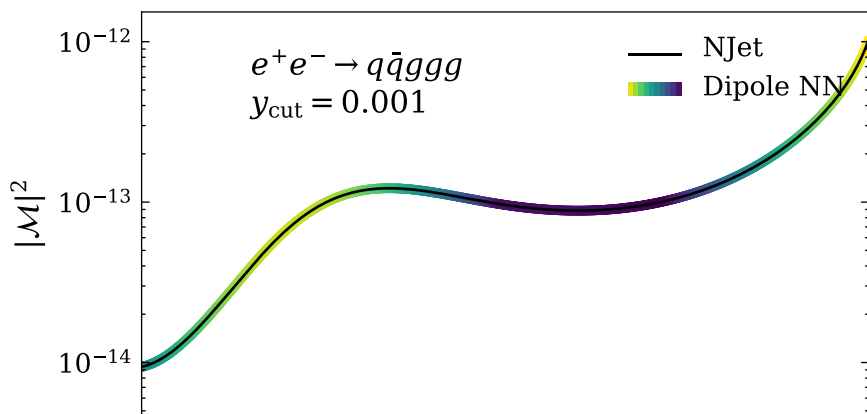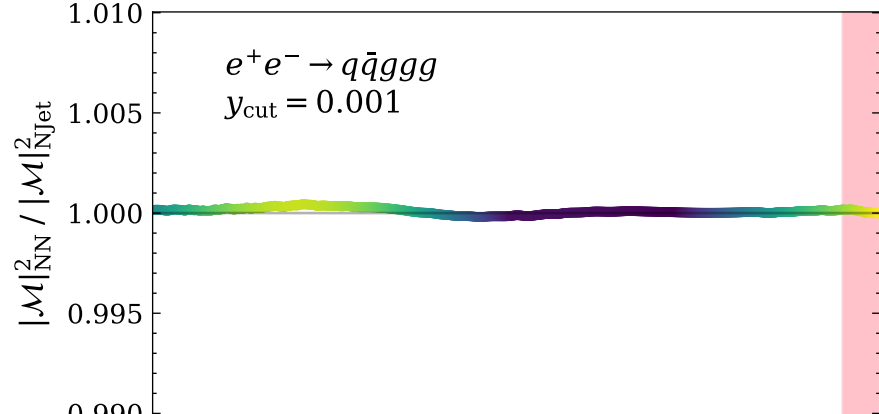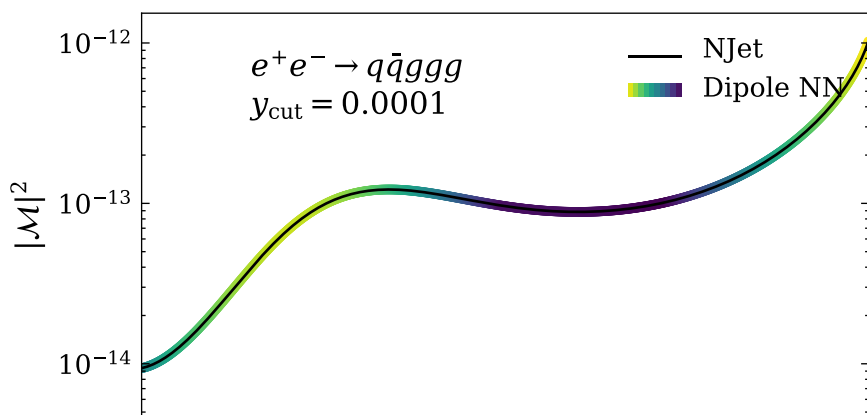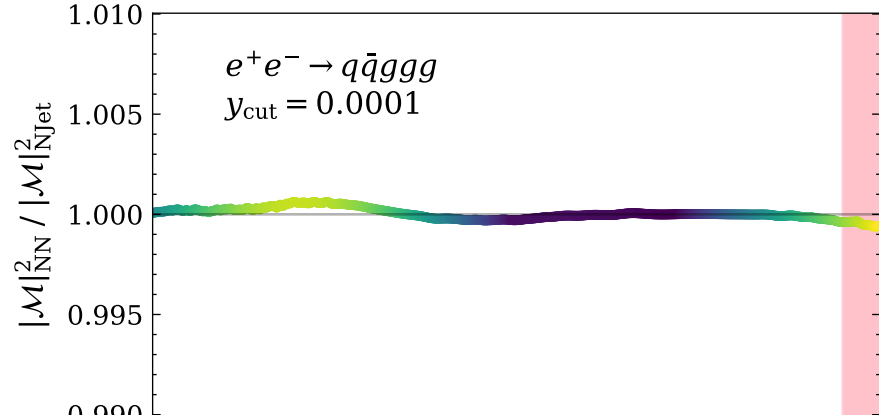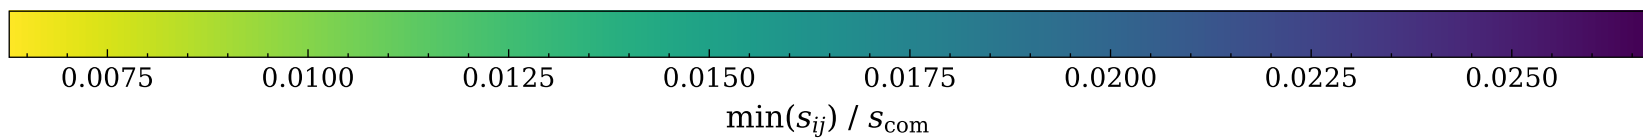

Trajectory 1238

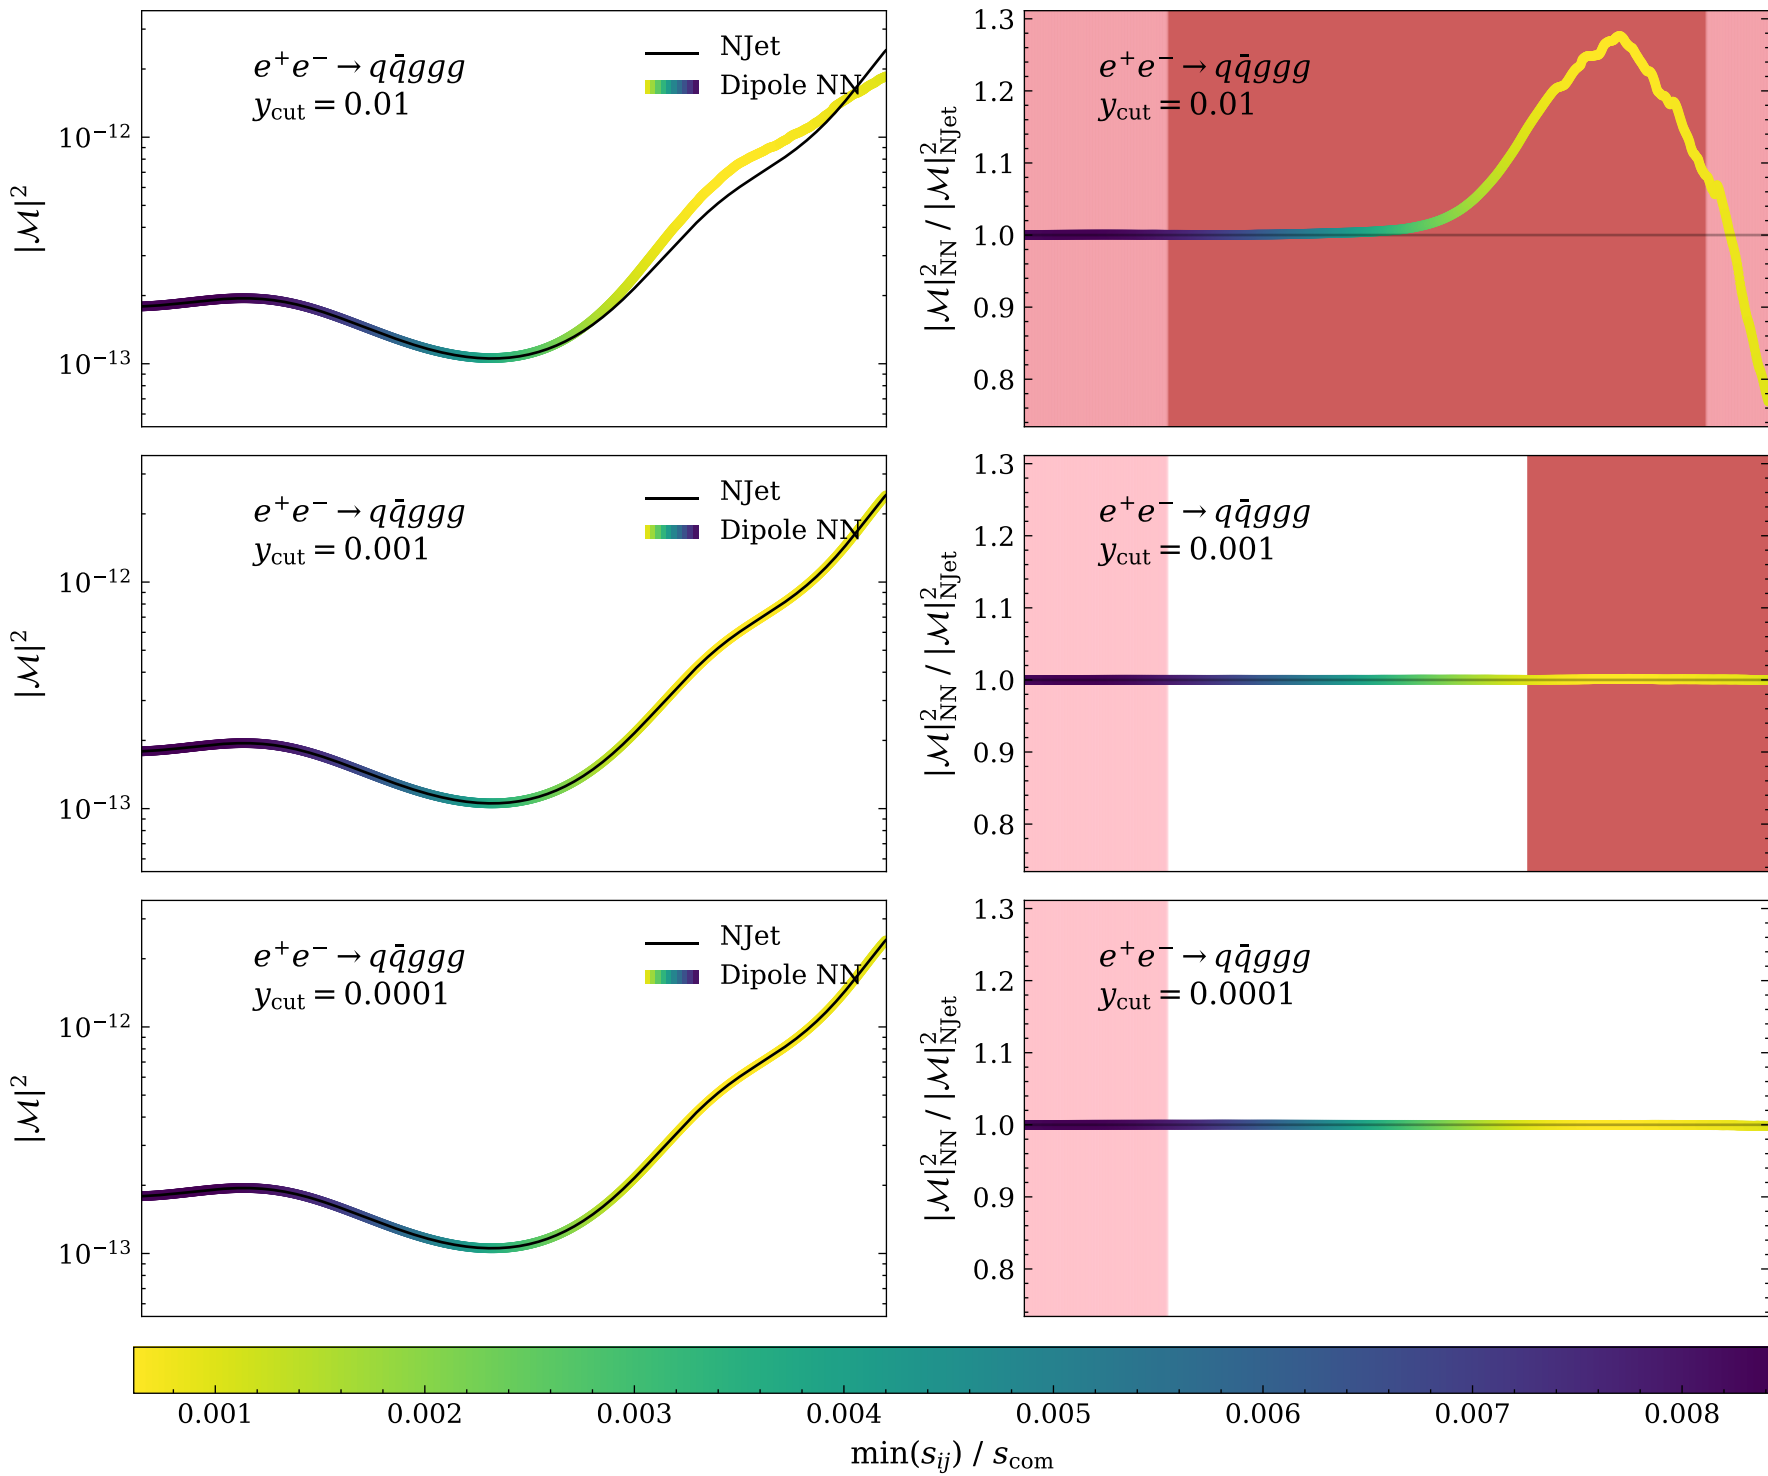

Trajectory 1239

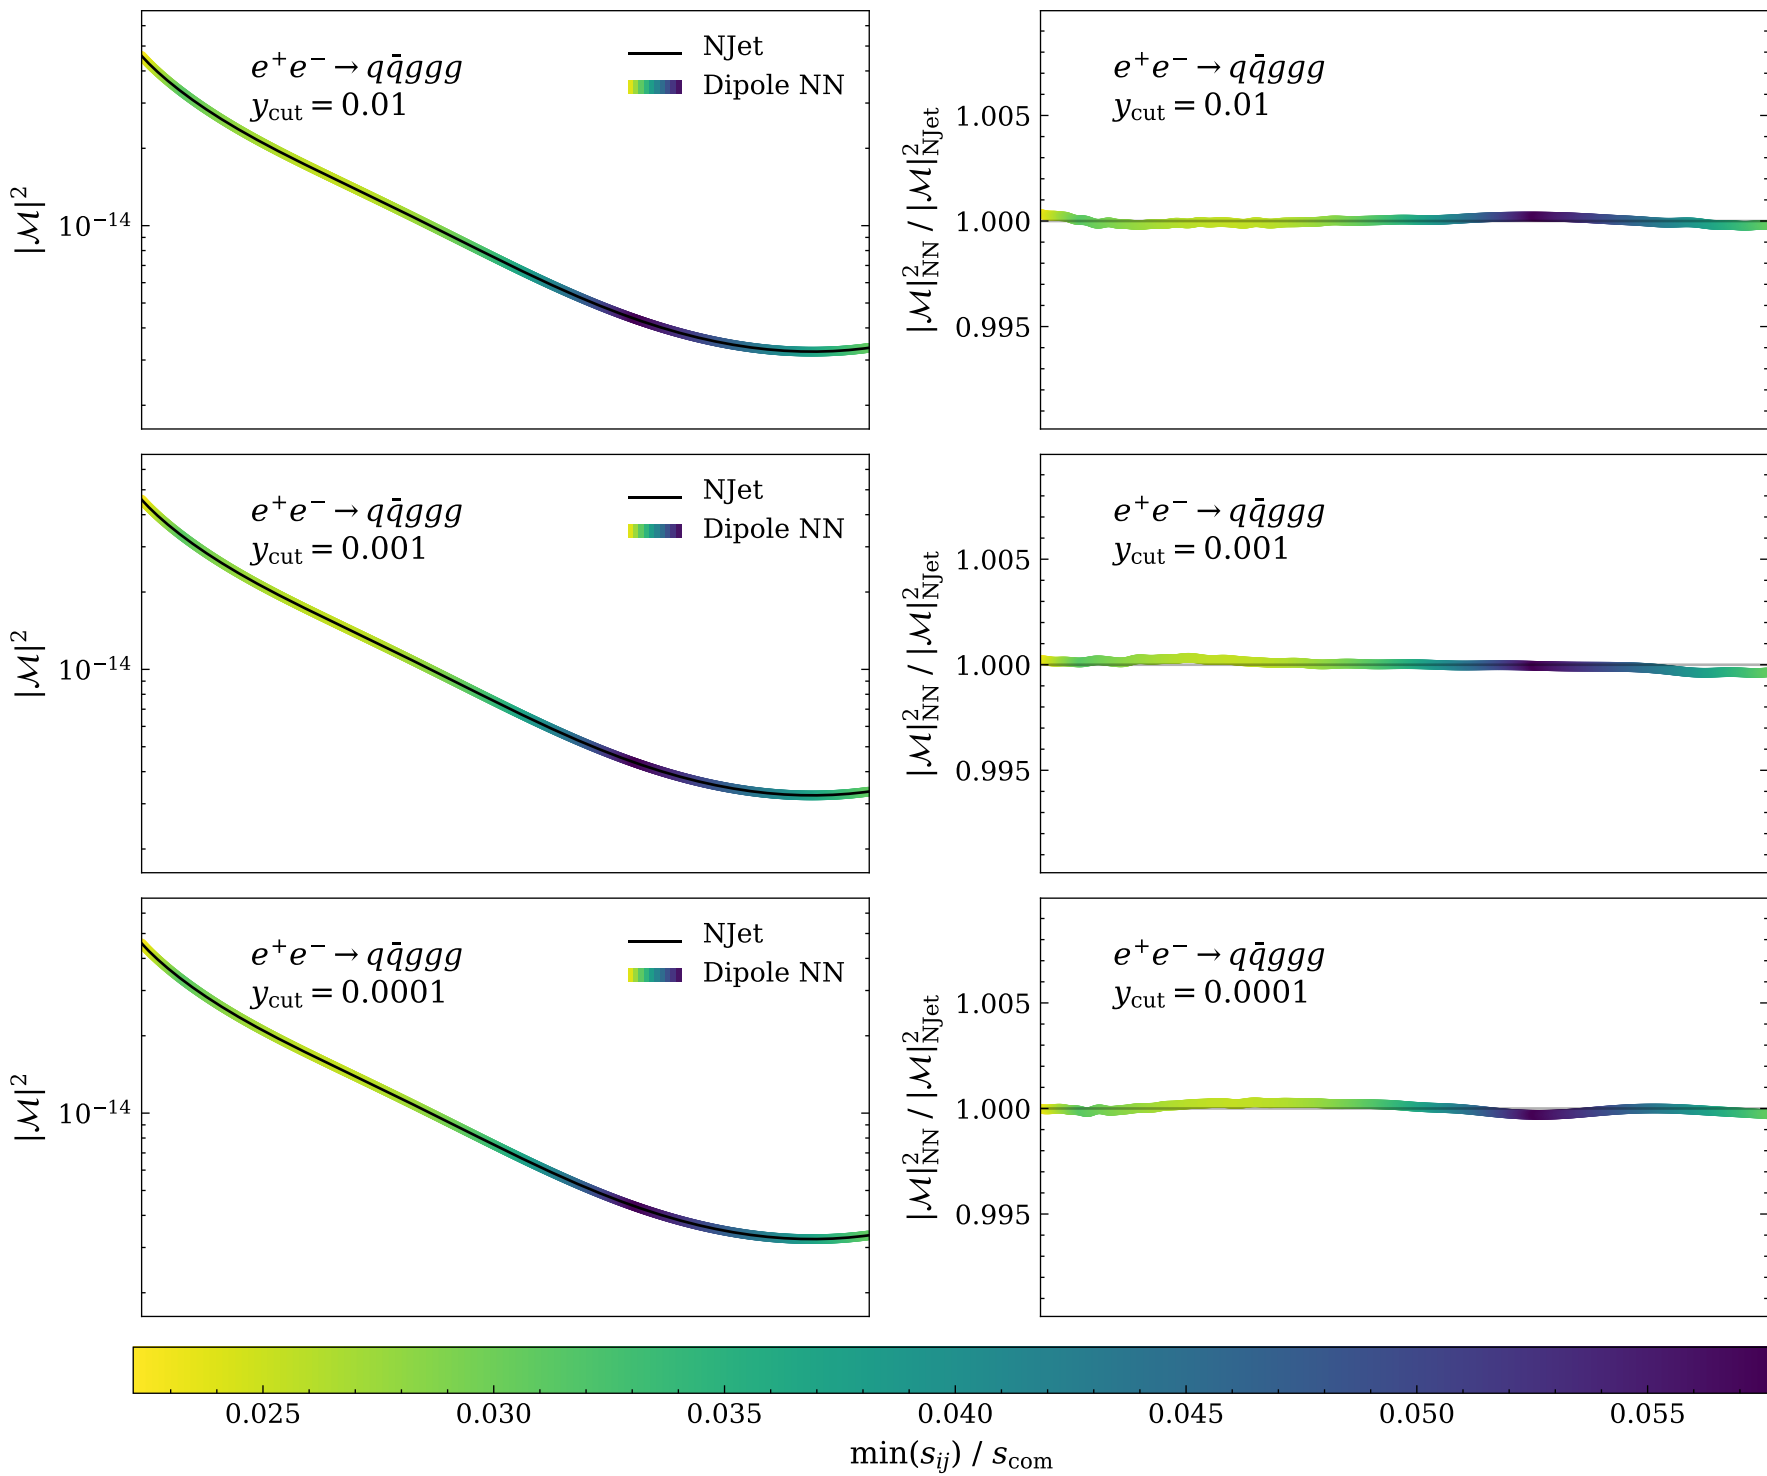

Trajectory 1240

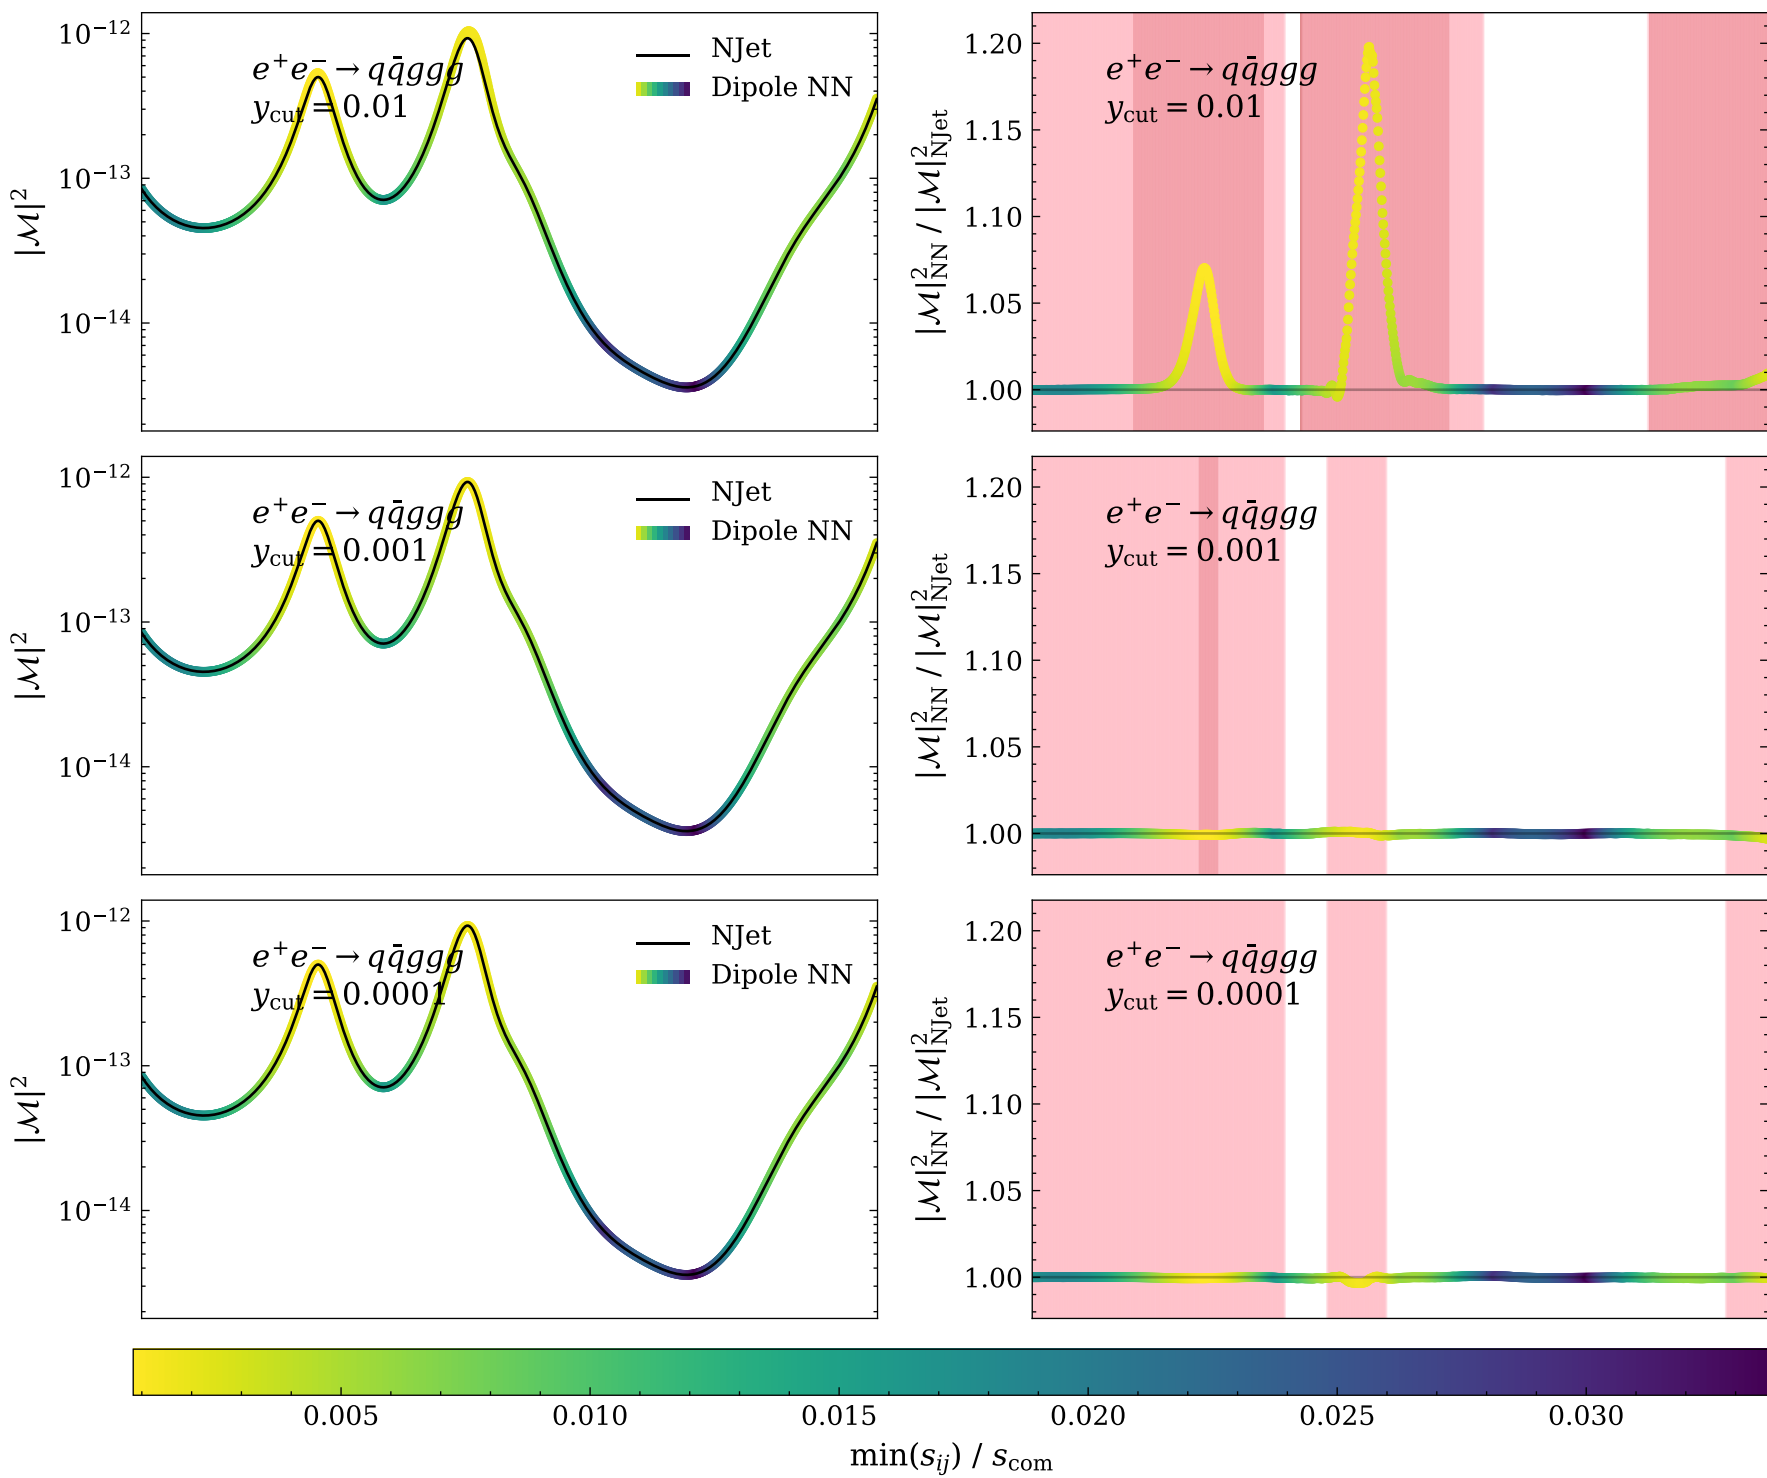

Trajectory 1241

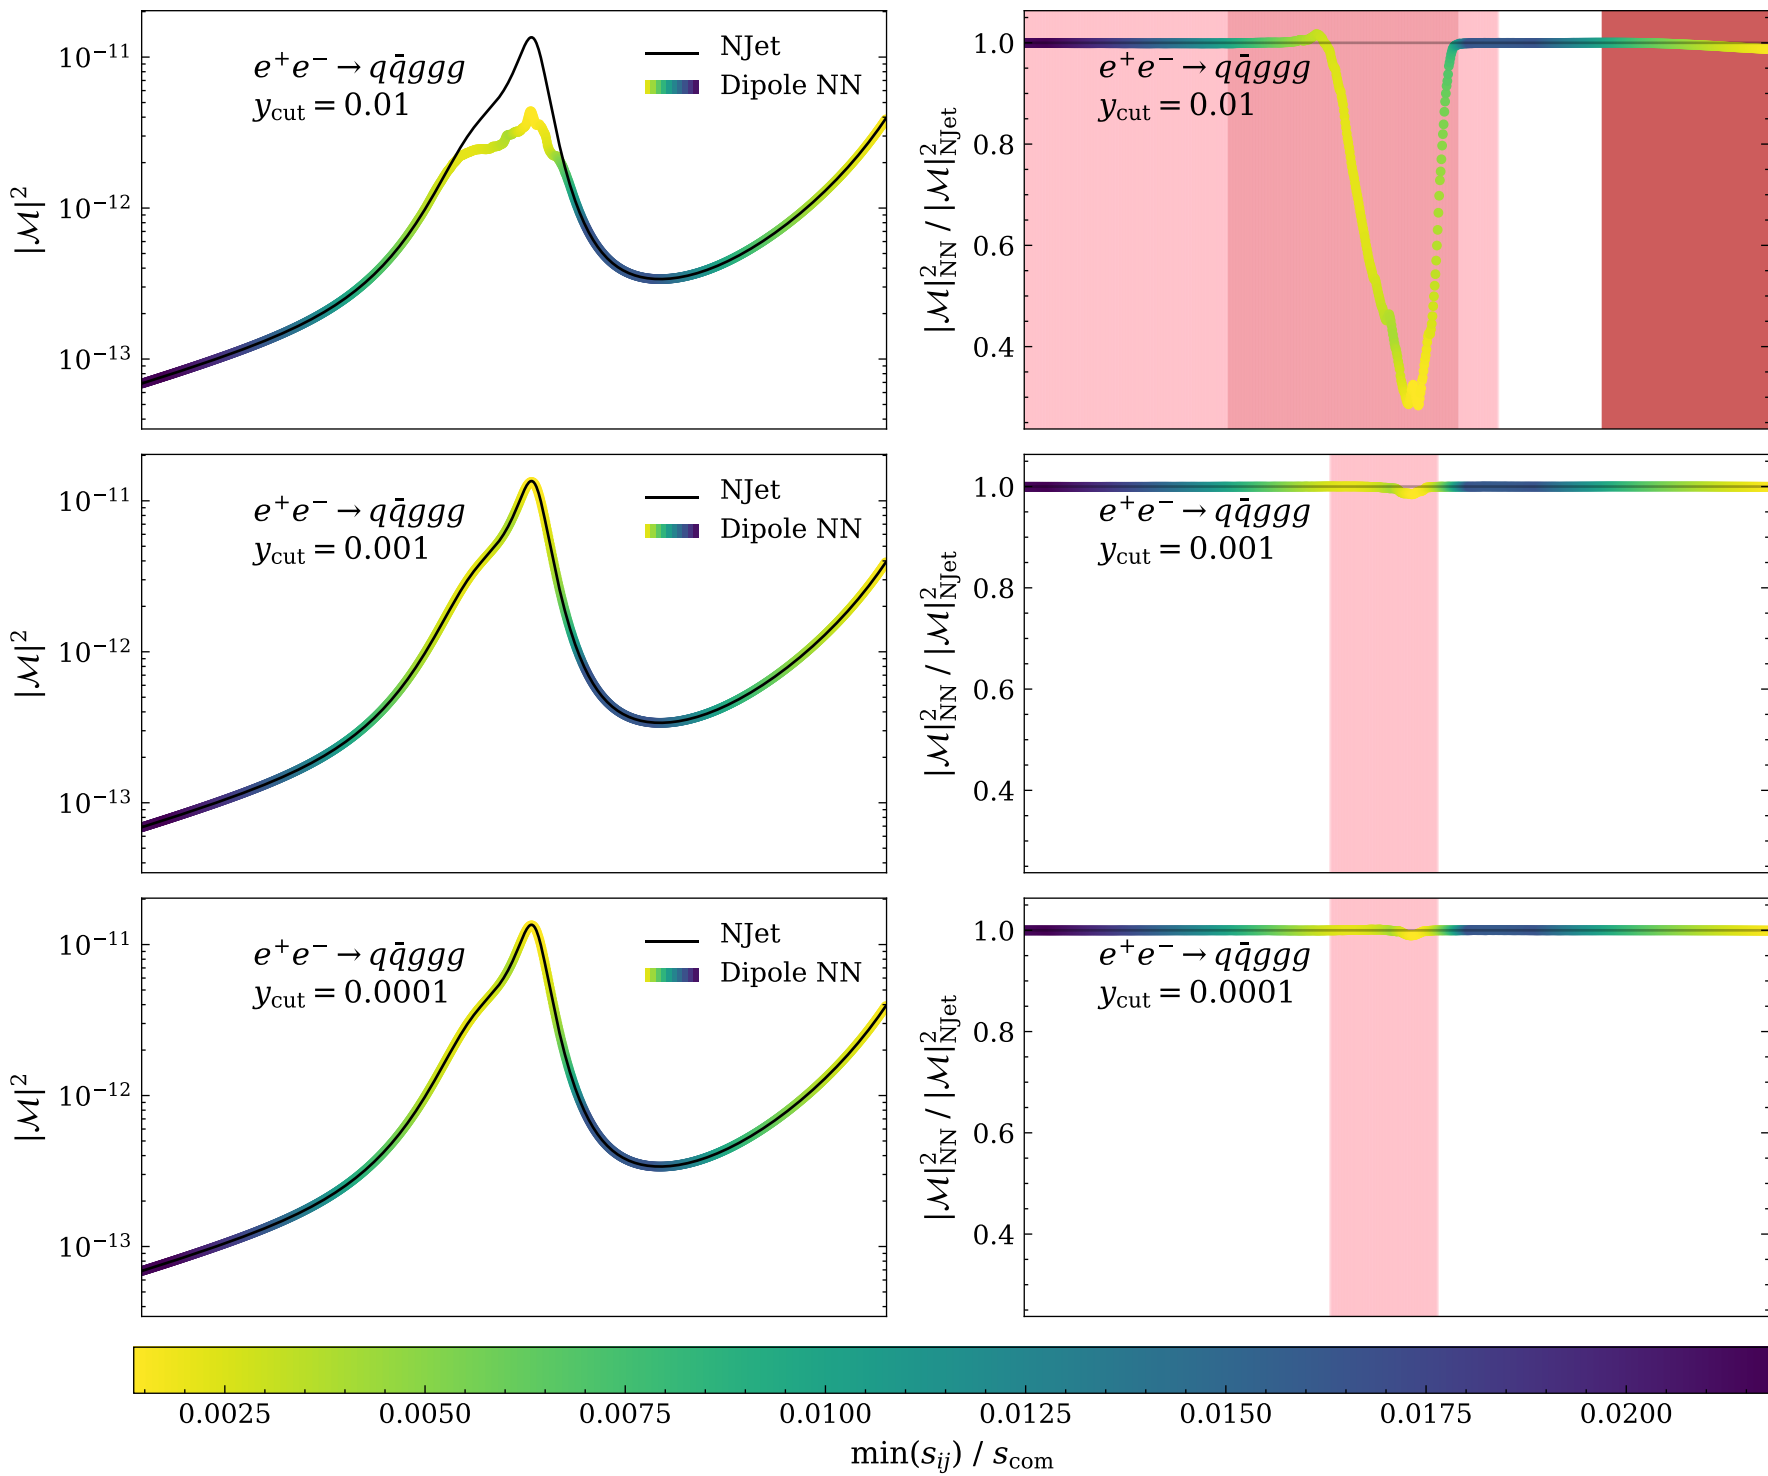

Trajectory 1242

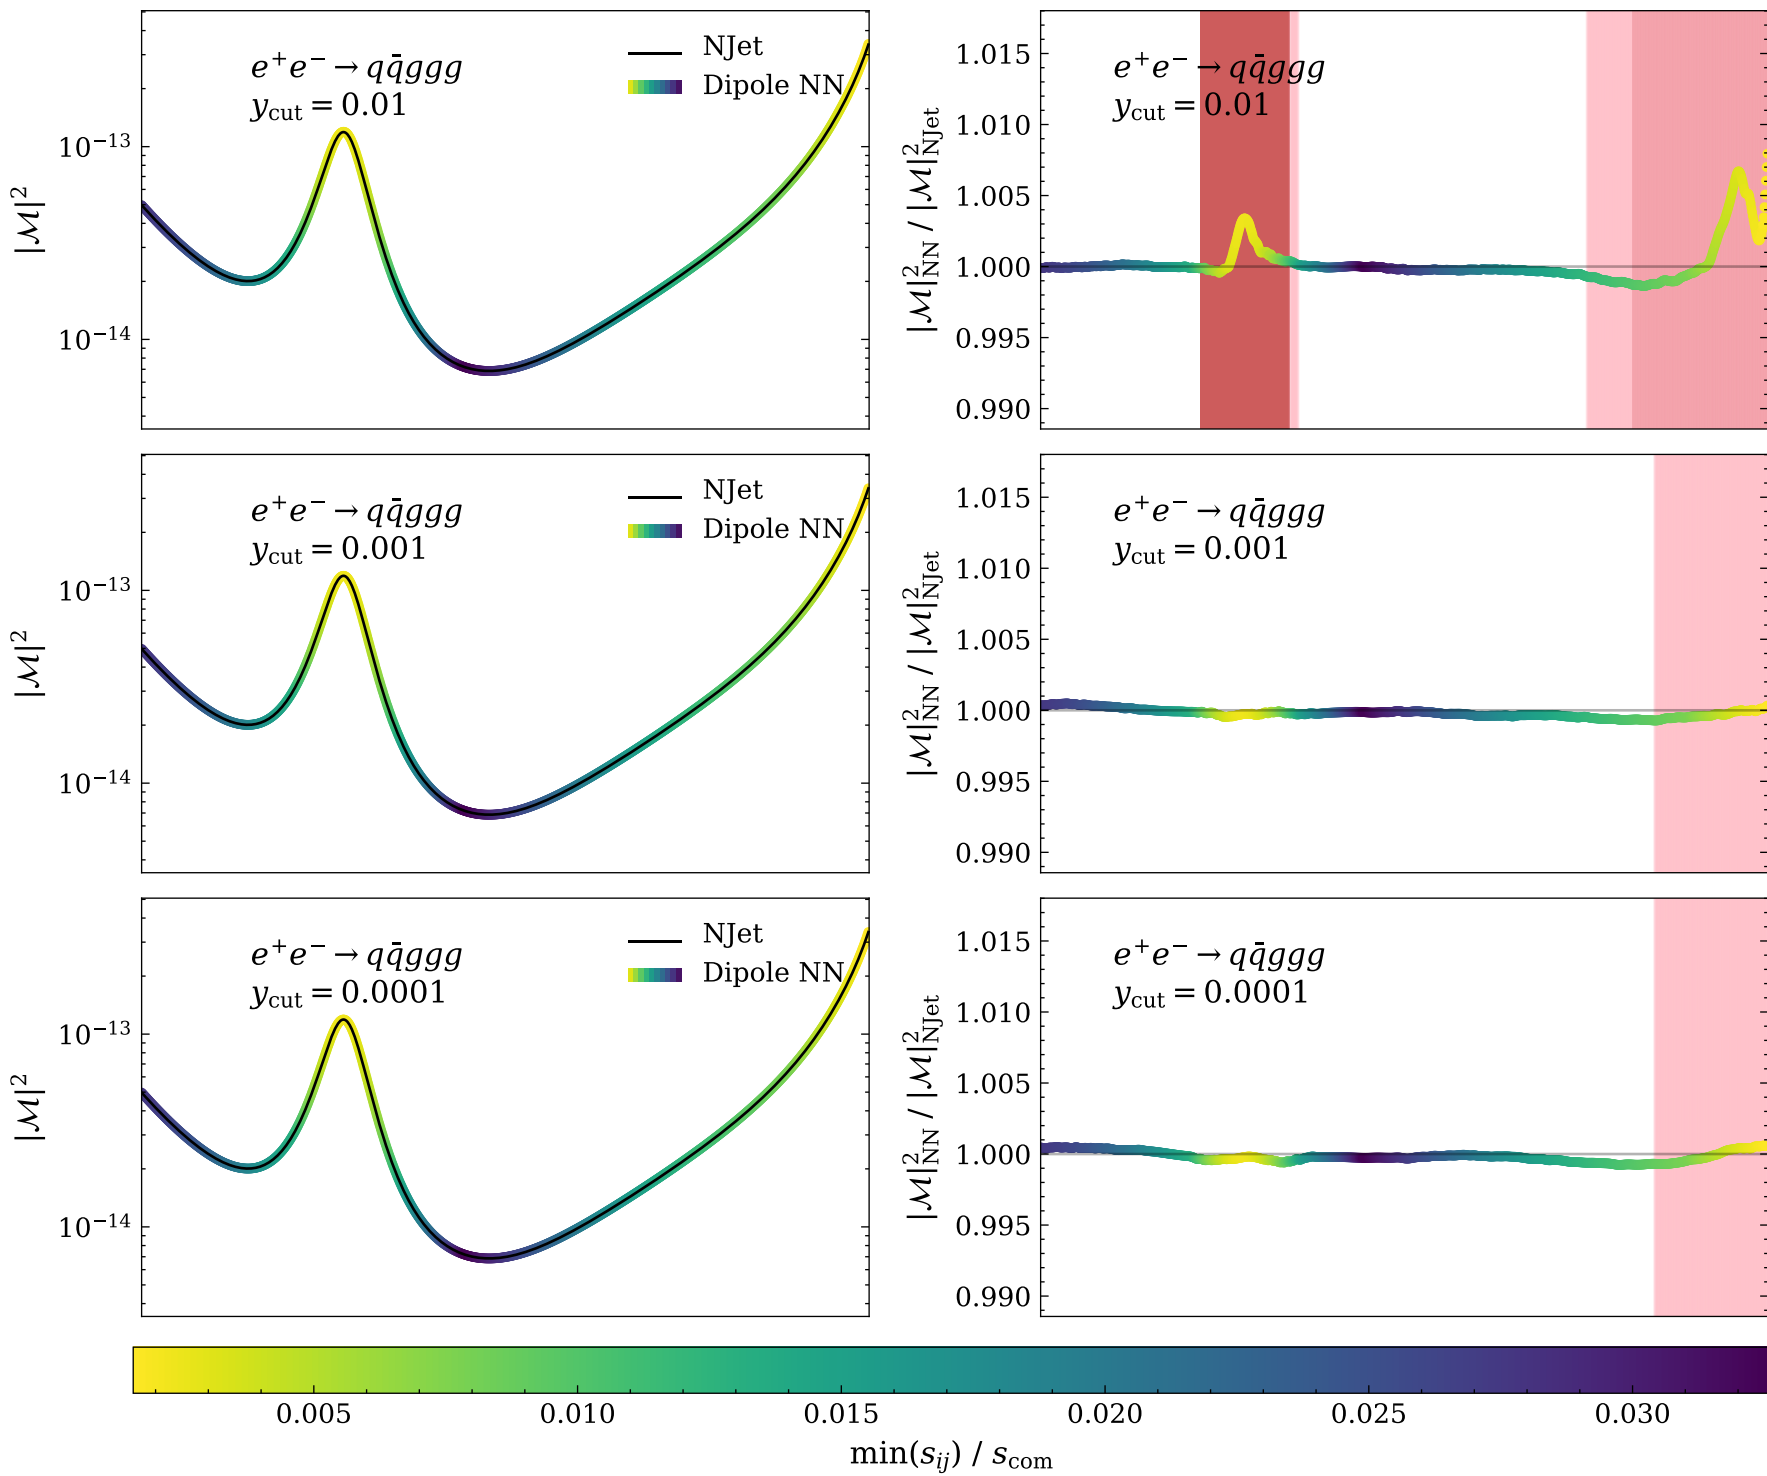

Trajectory 1243

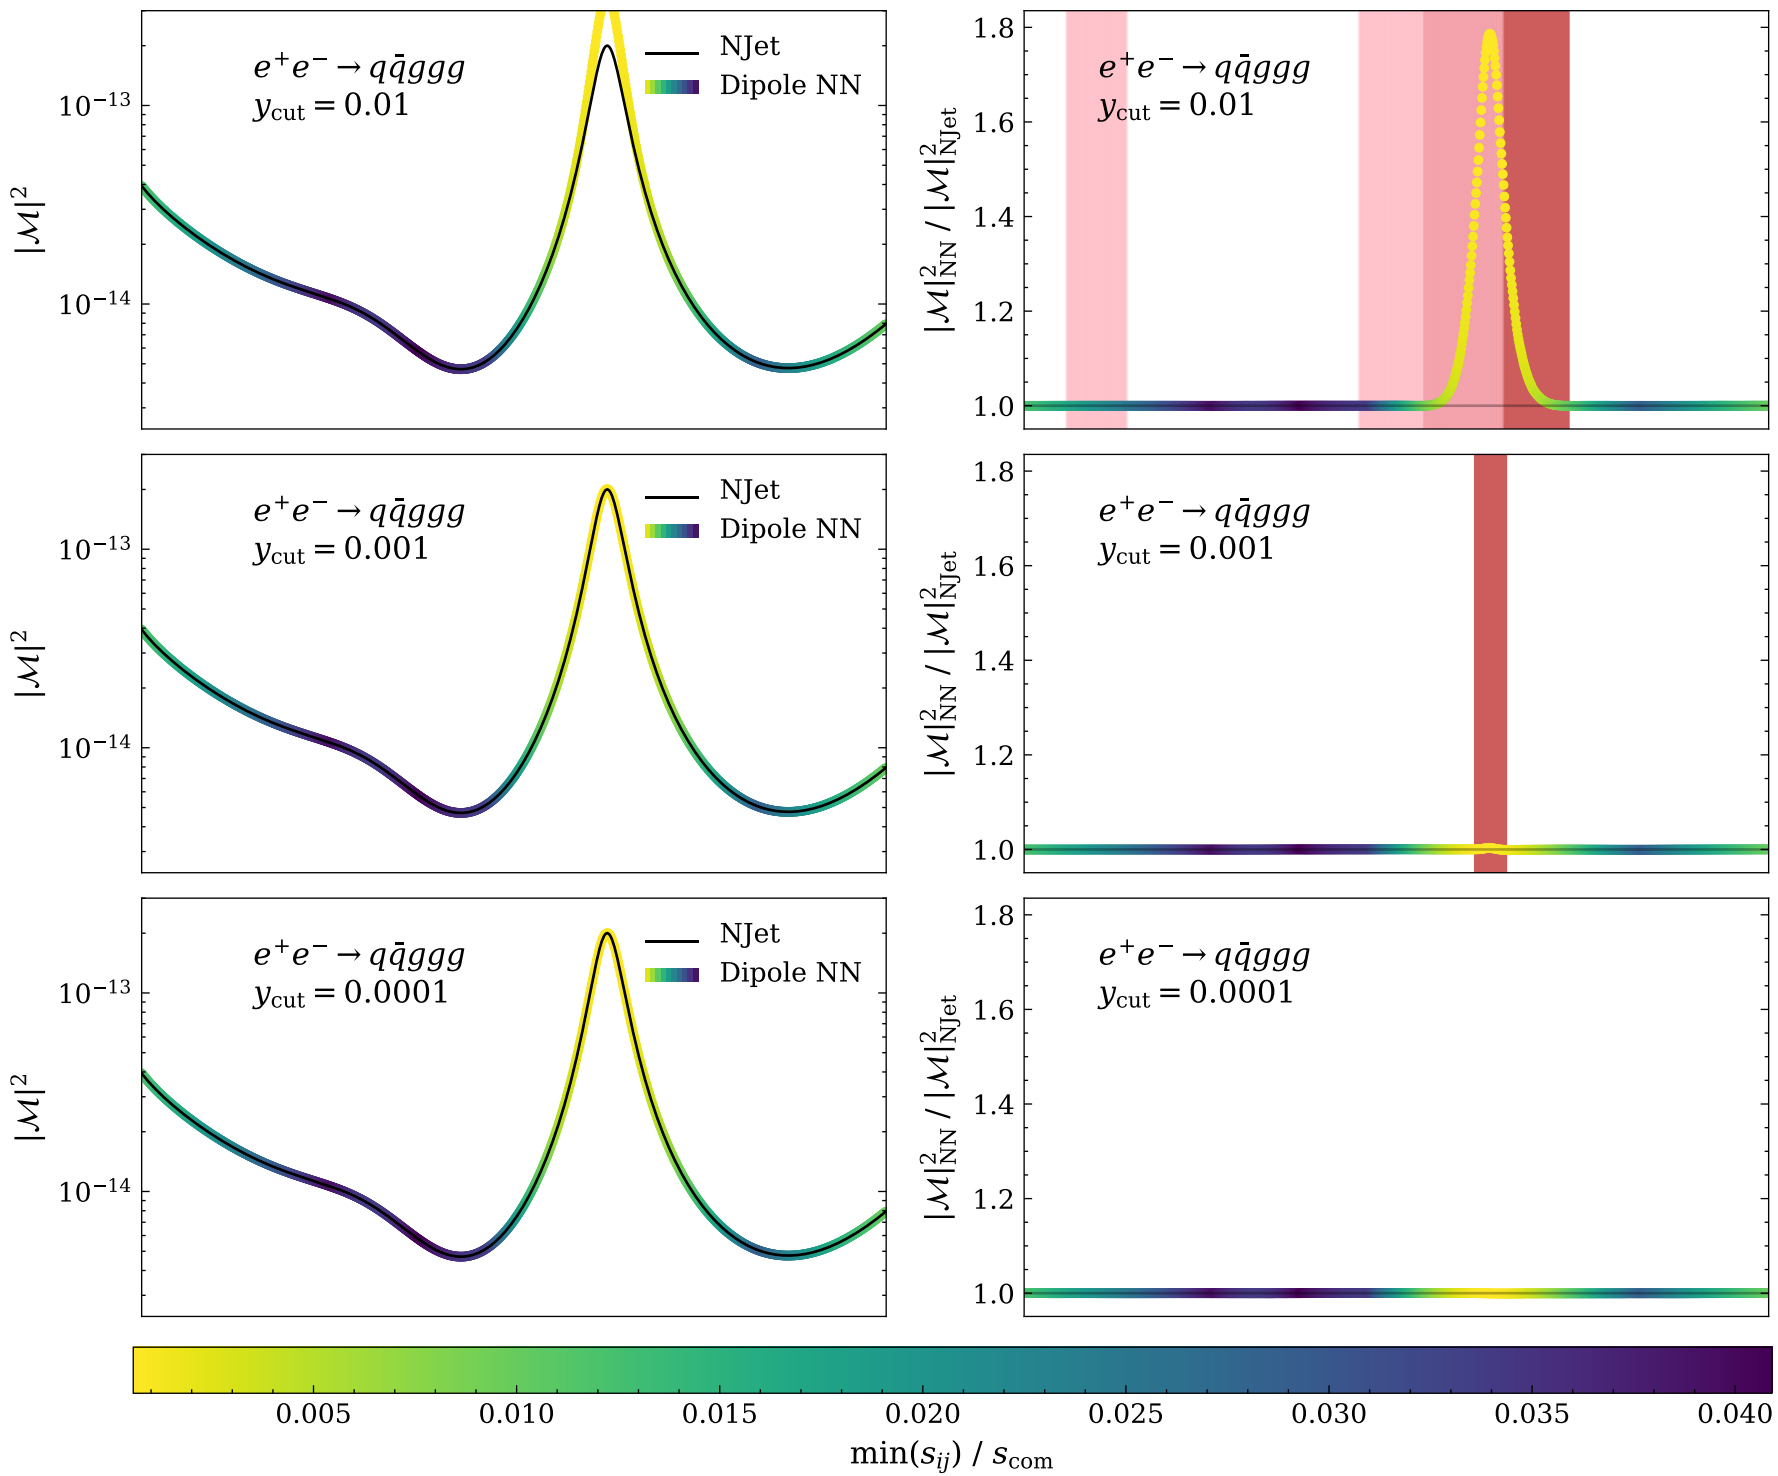

Trajectory 1244

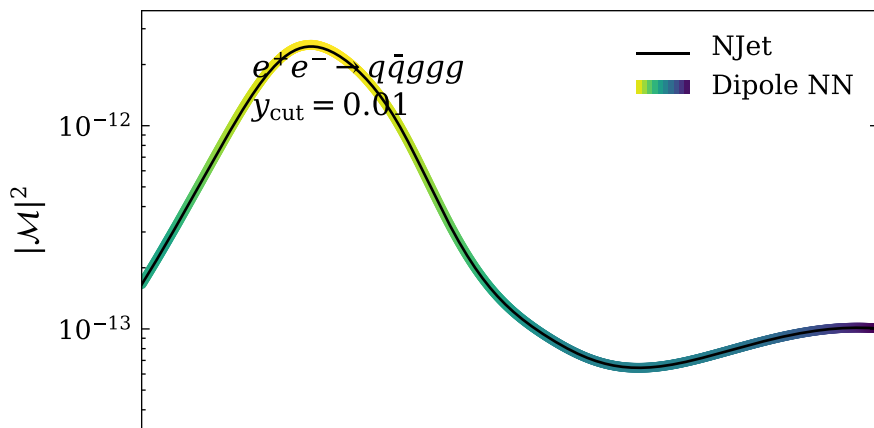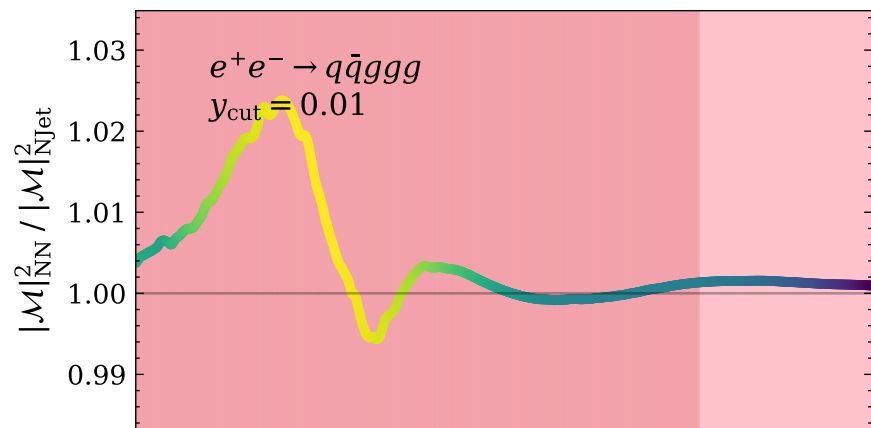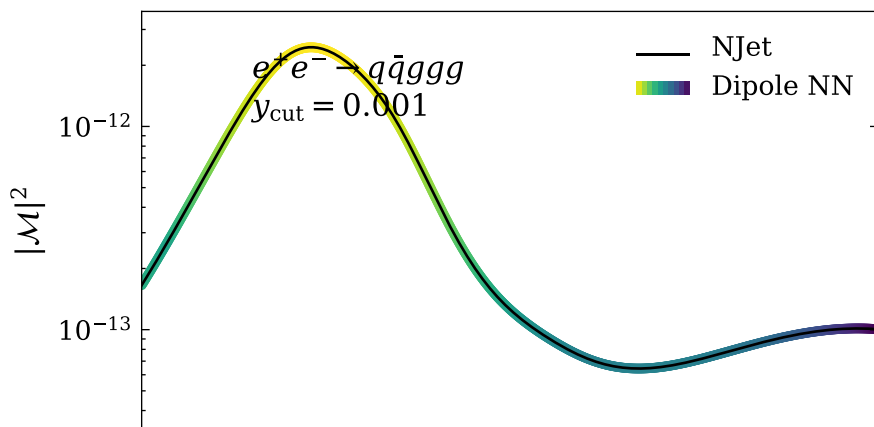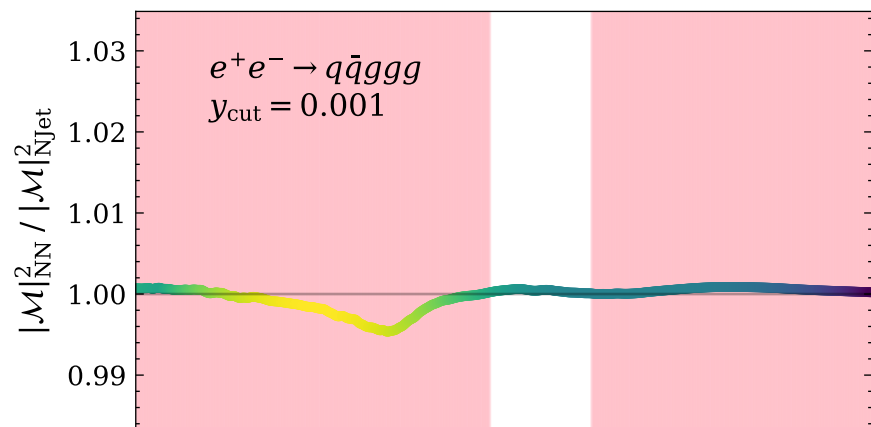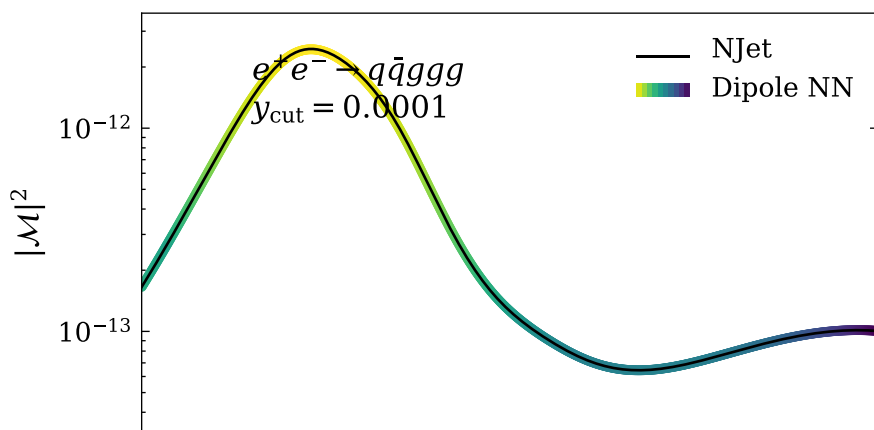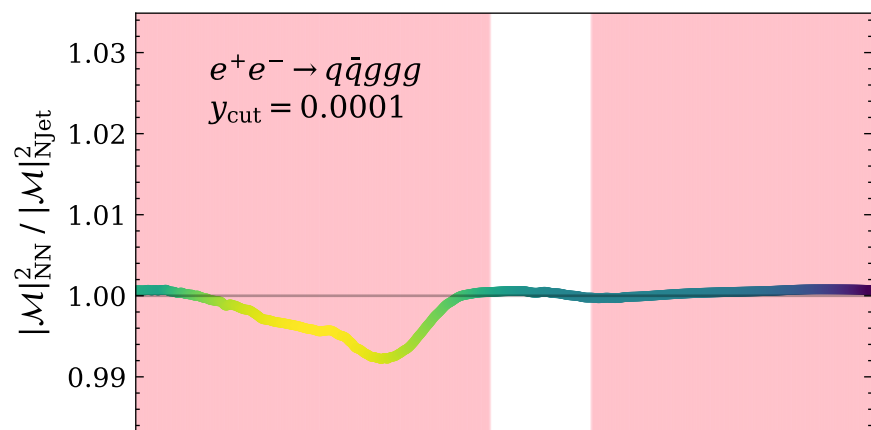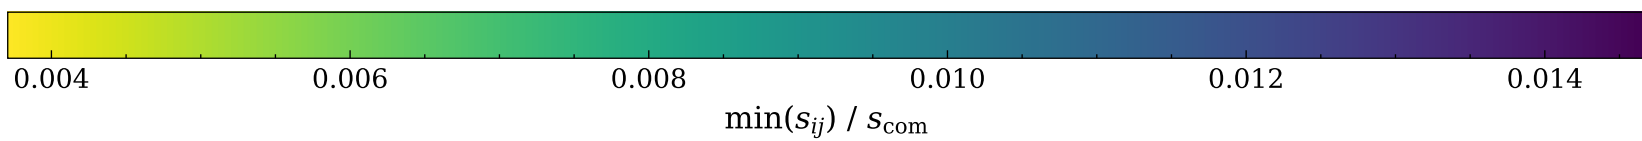

Trajectory 1245

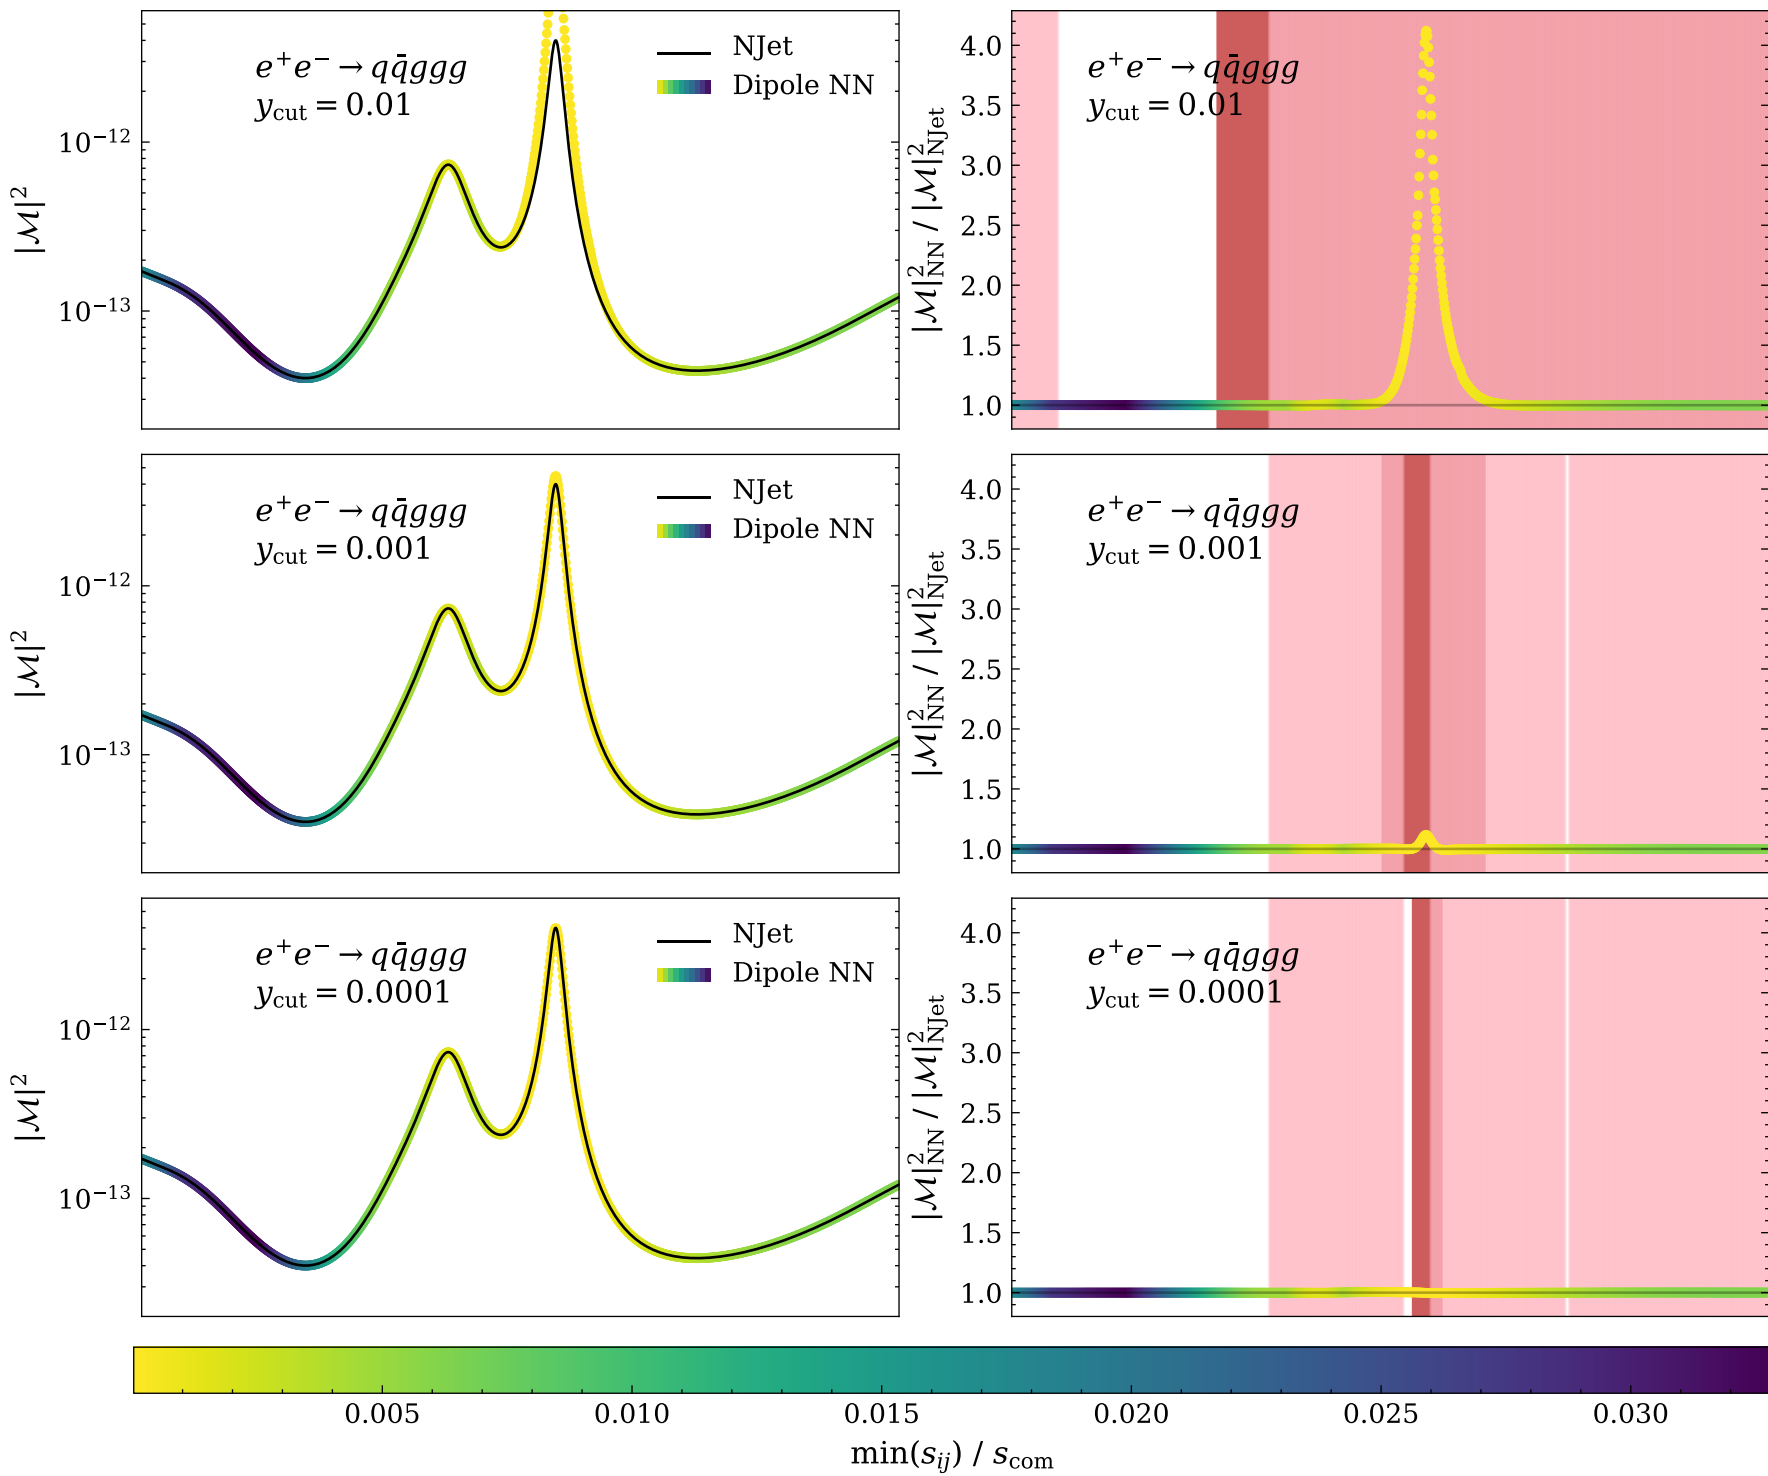

Trajectory 1246

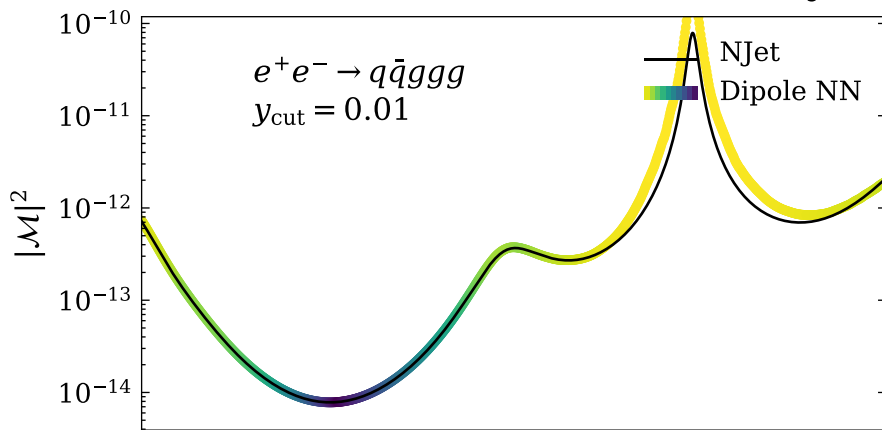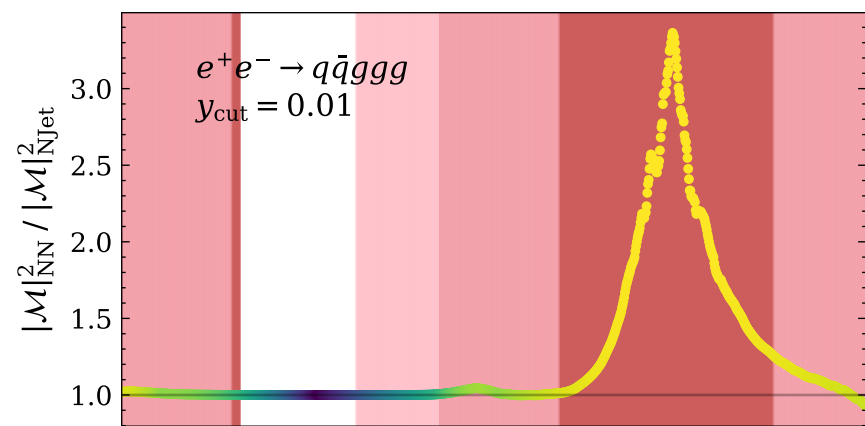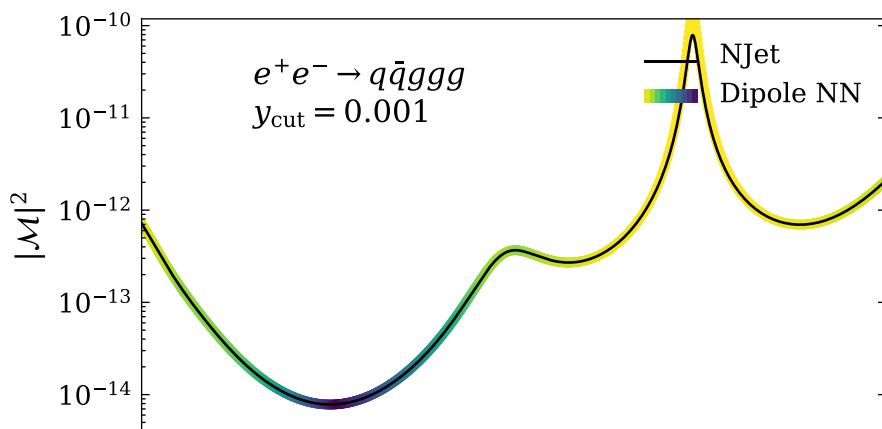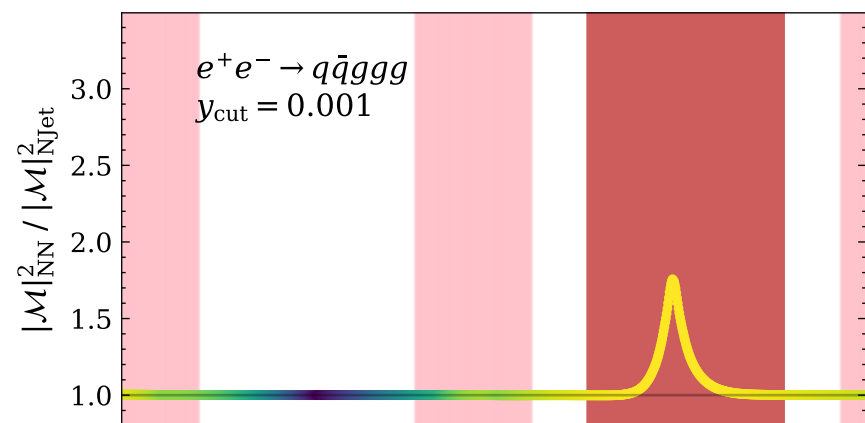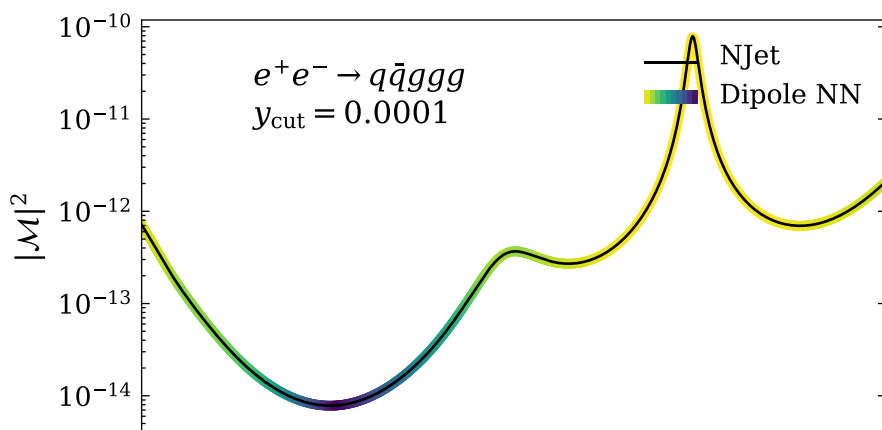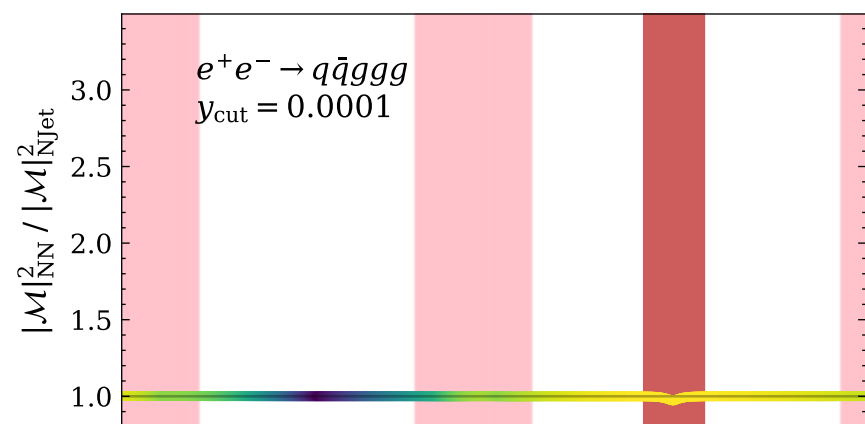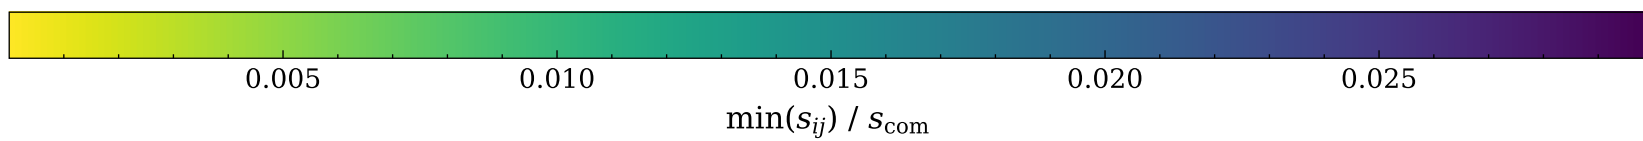

Trajectory 1247

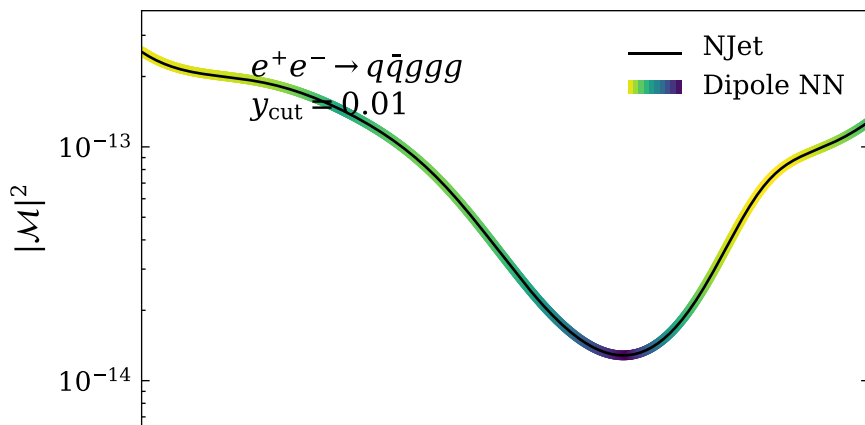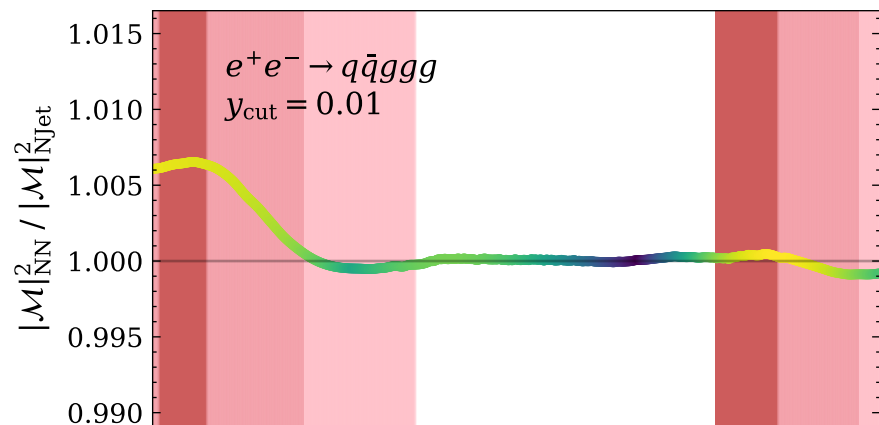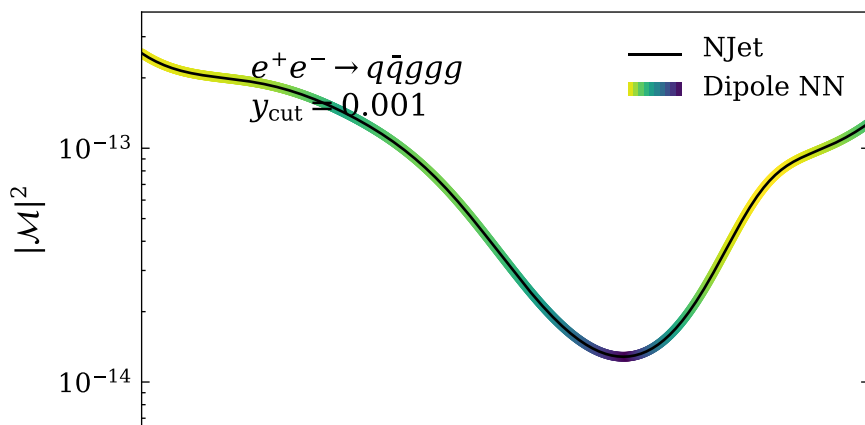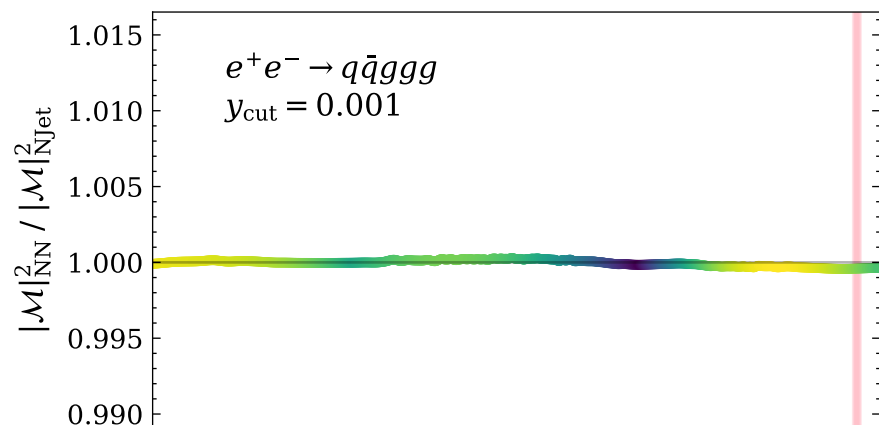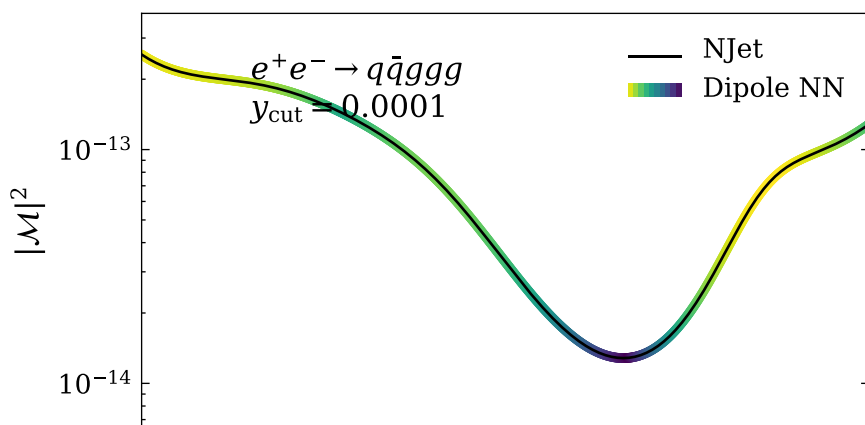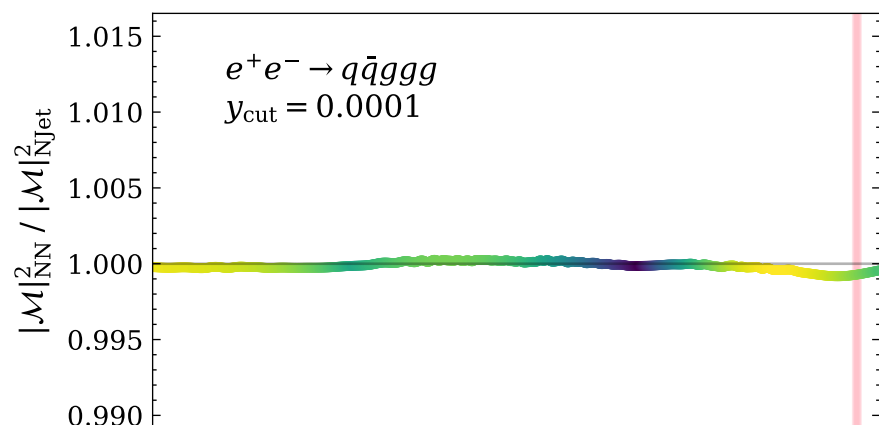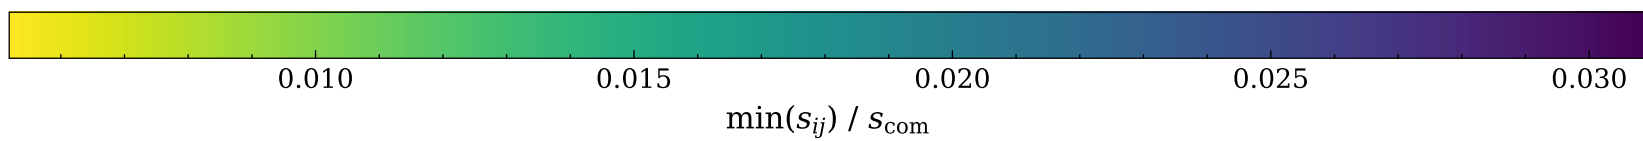

Trajectory 1248

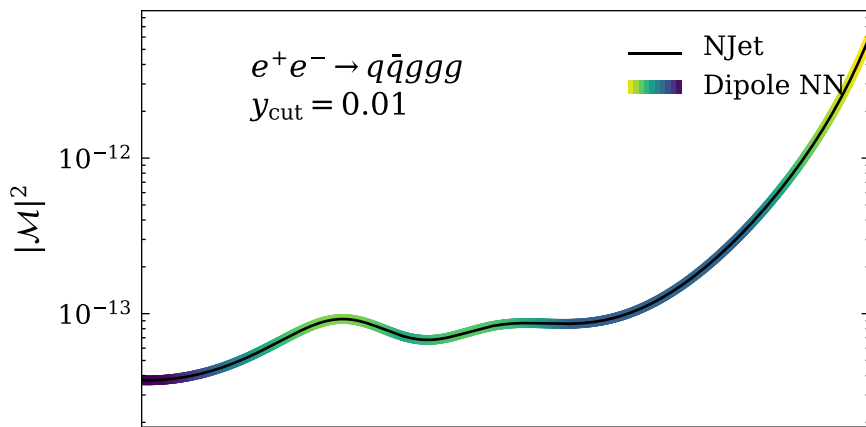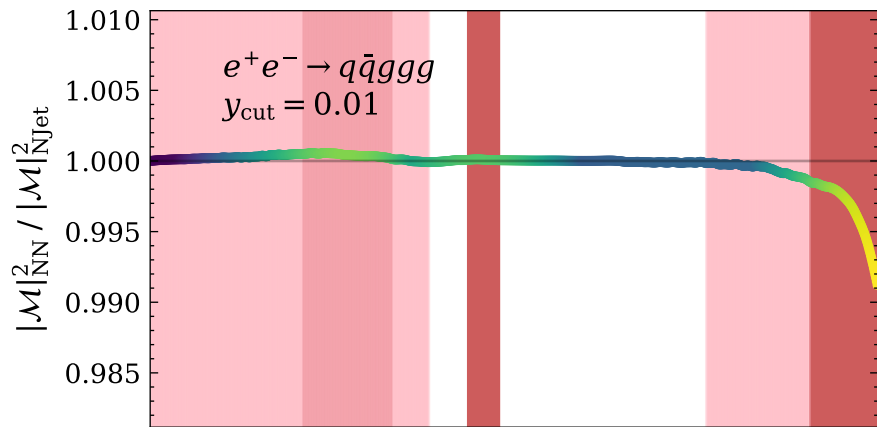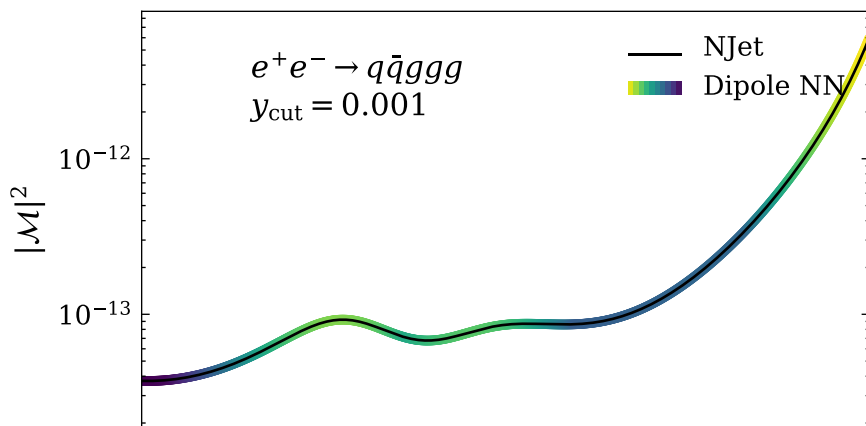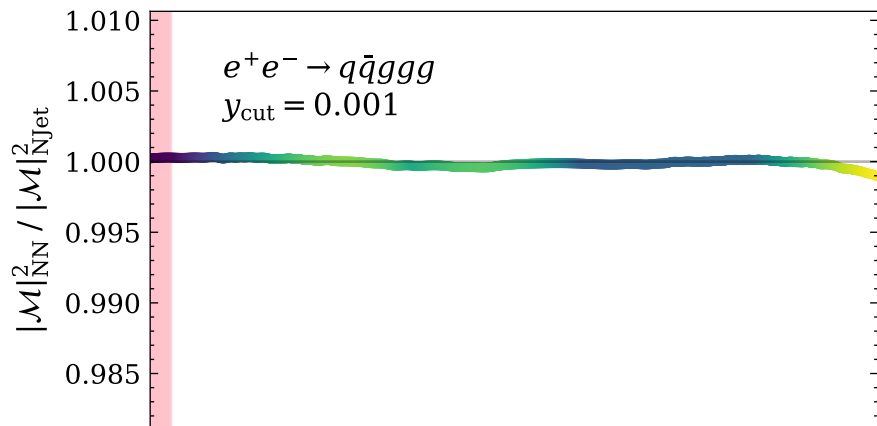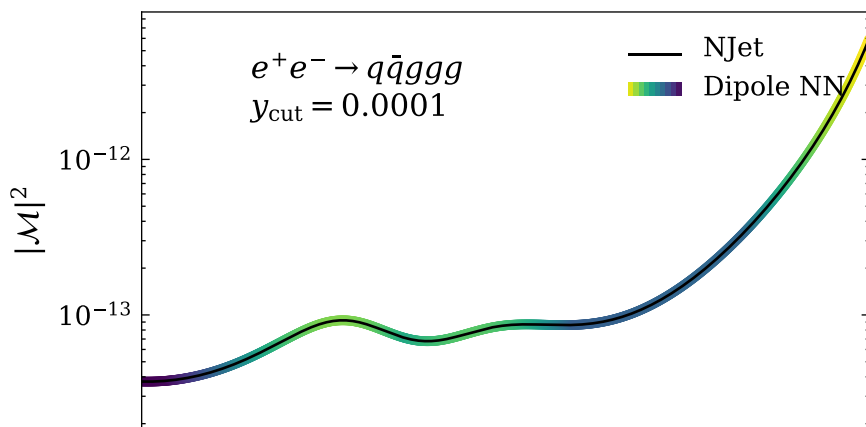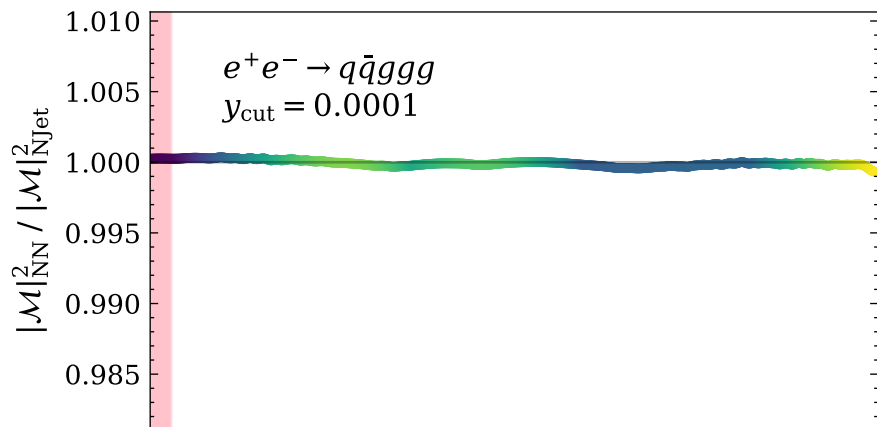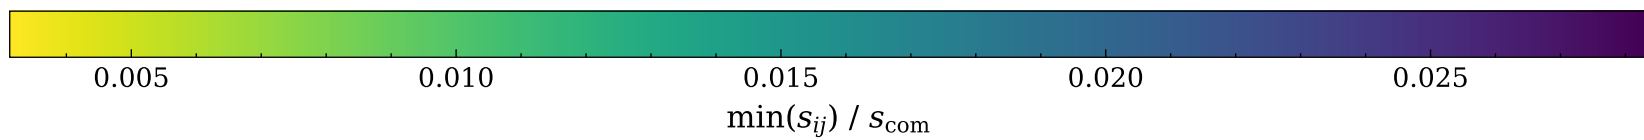

Trajectory 1249

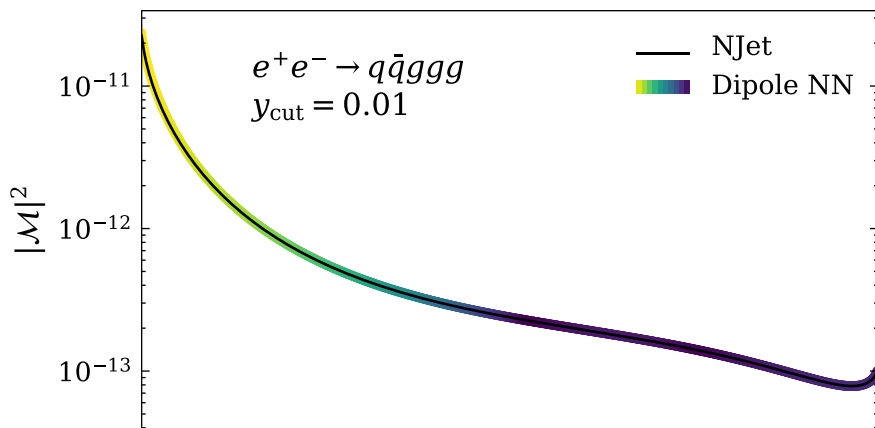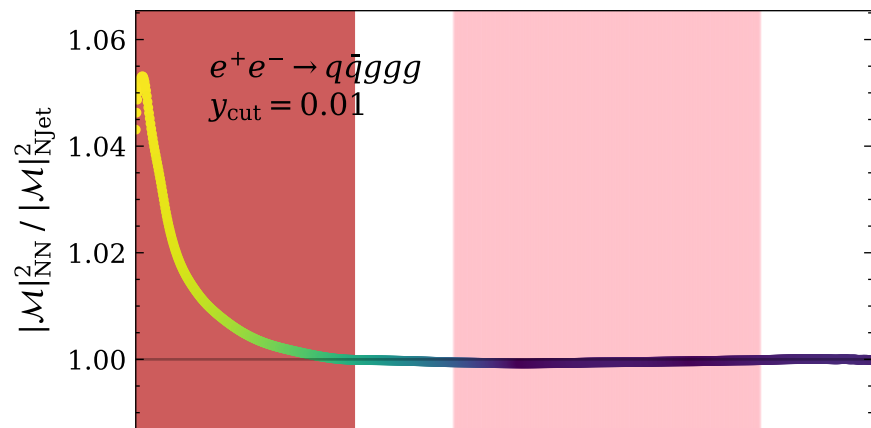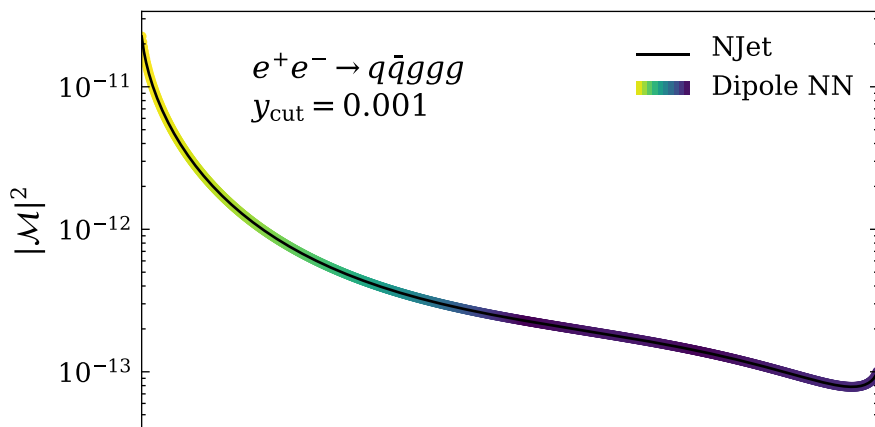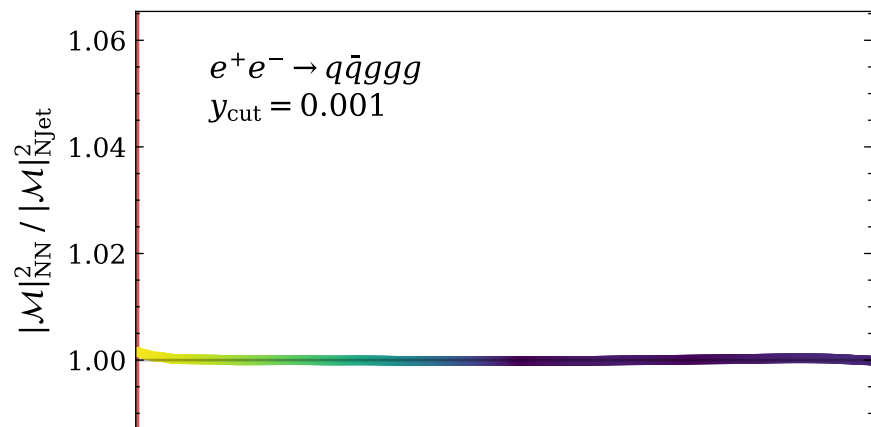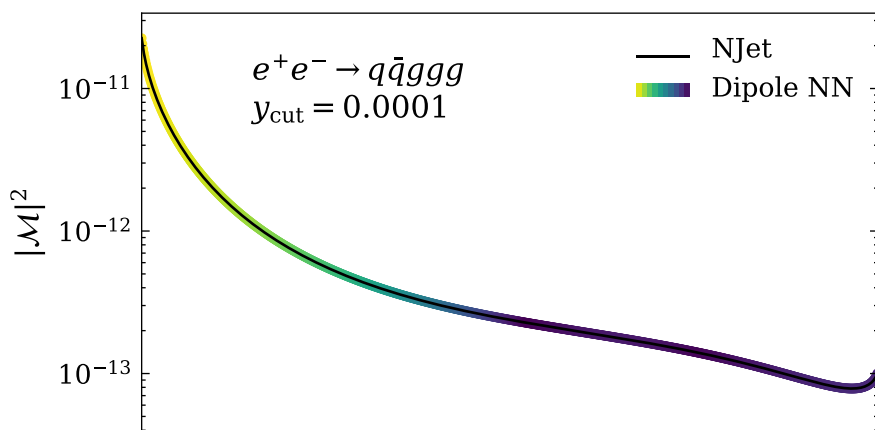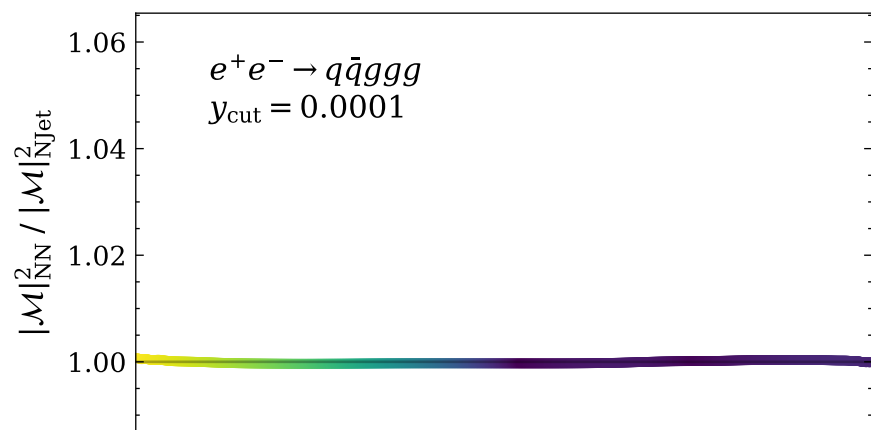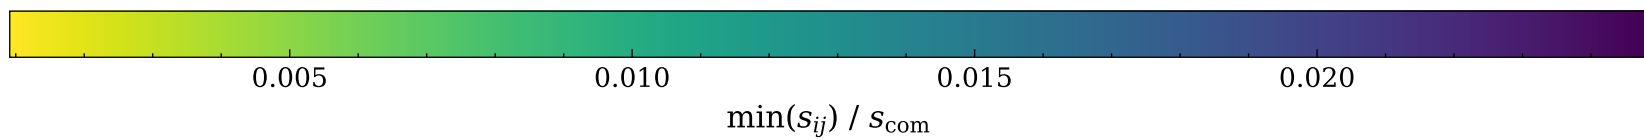

Trajectory 1250

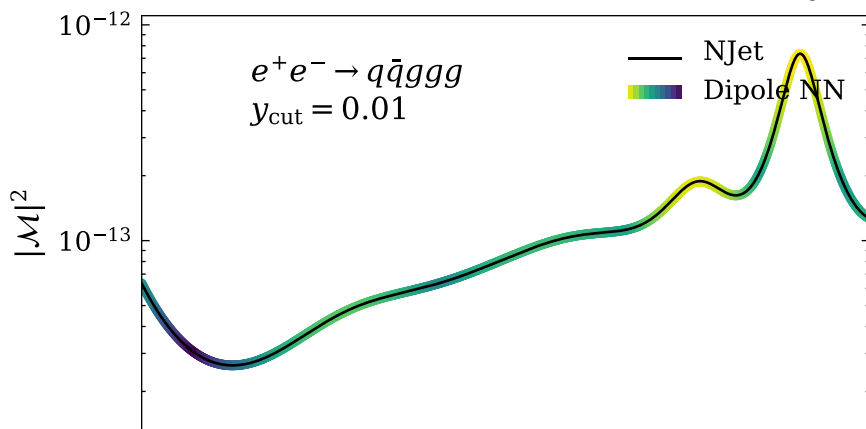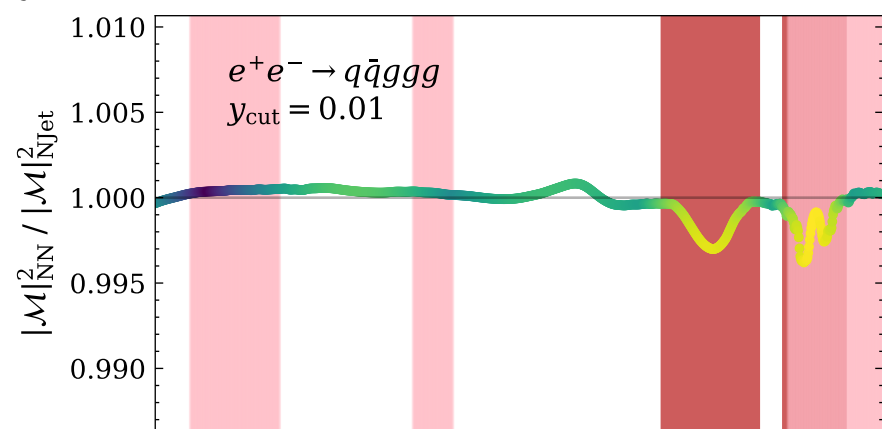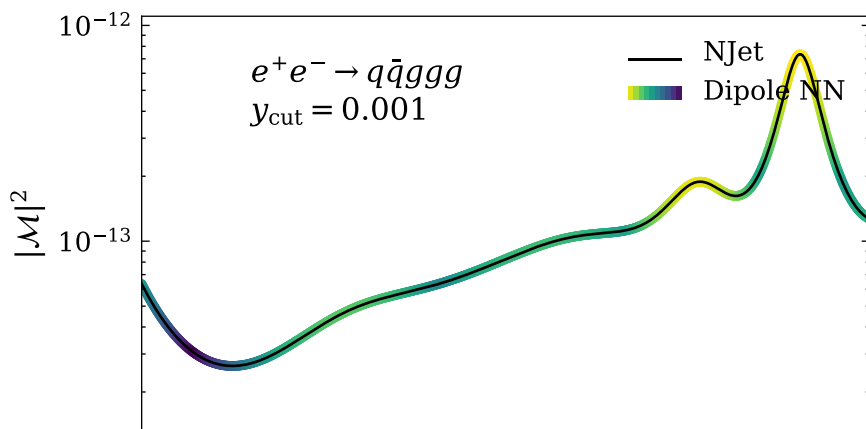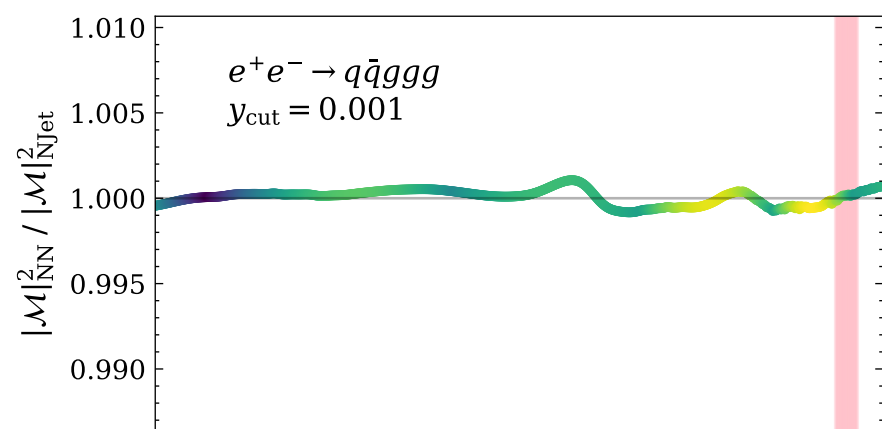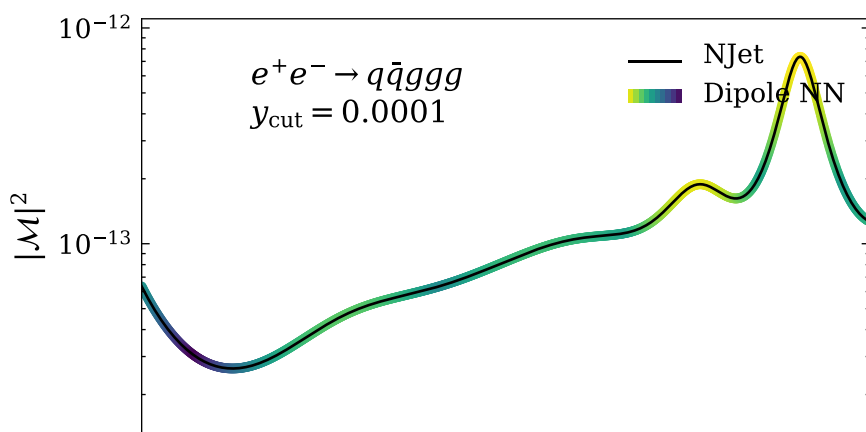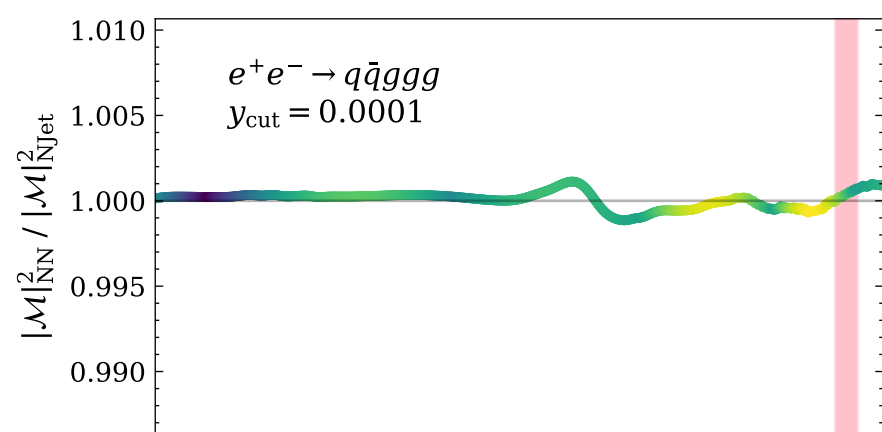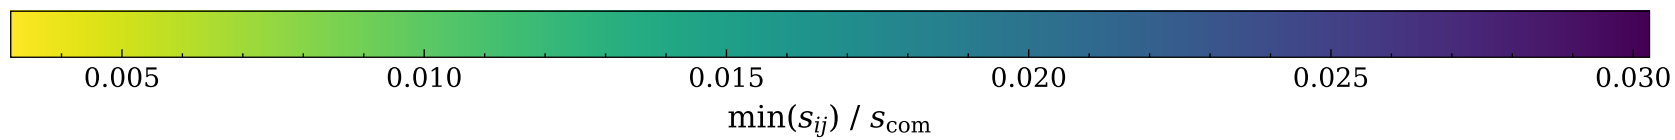

Trajectory 1251

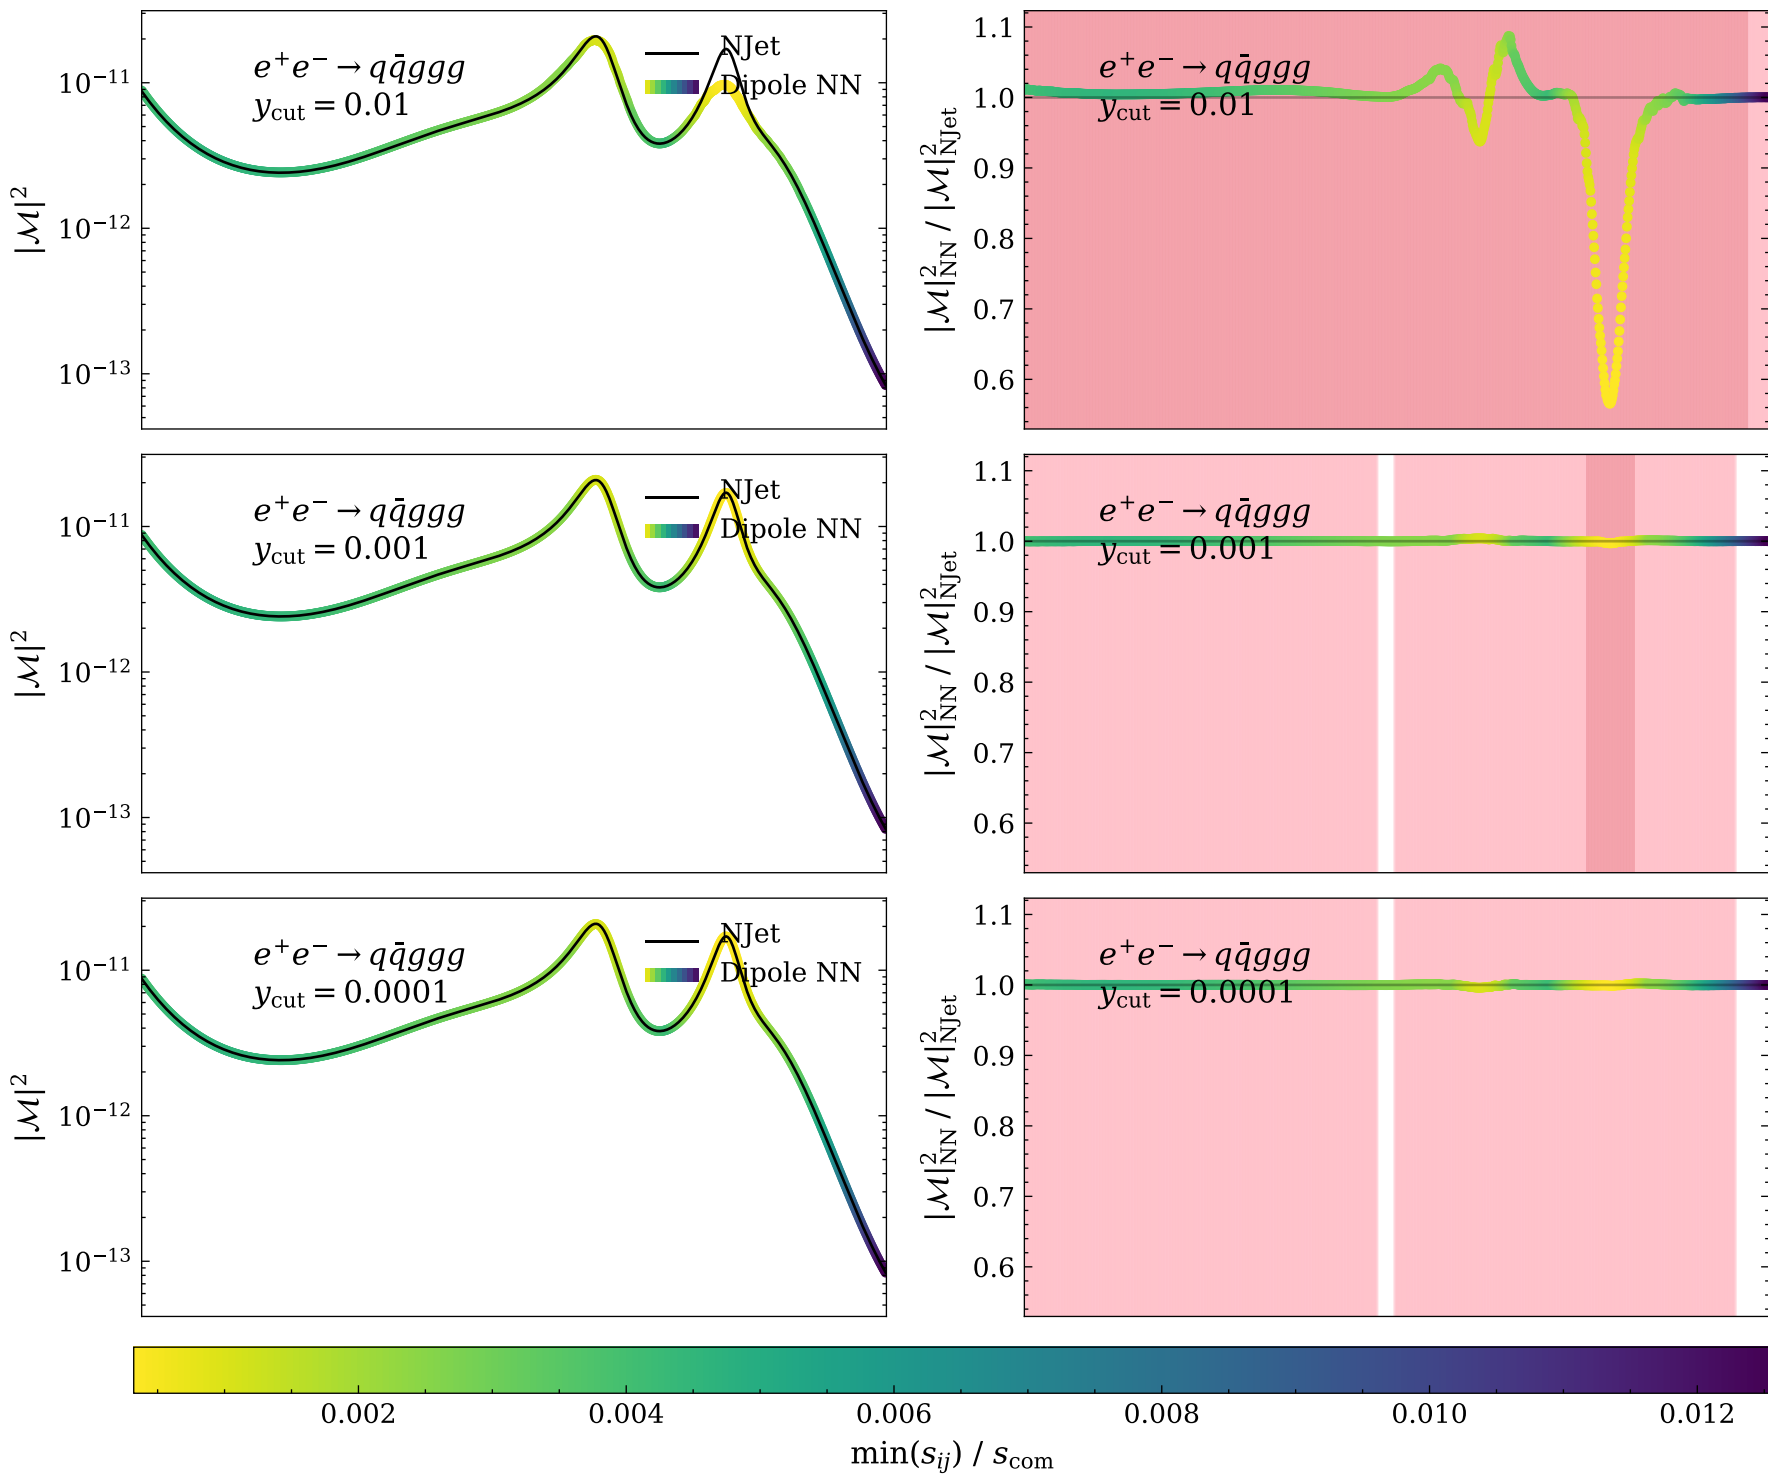

Trajectory 1252

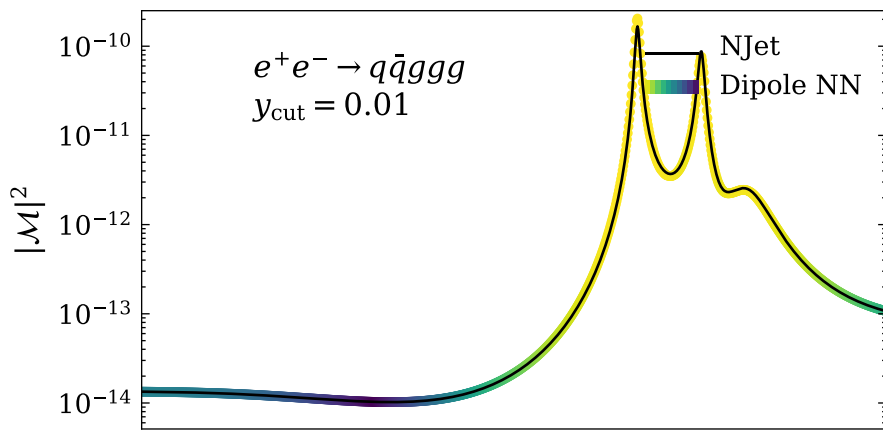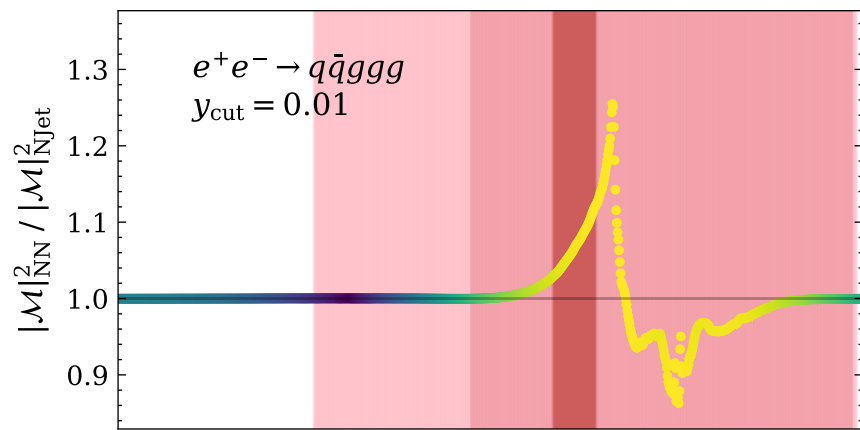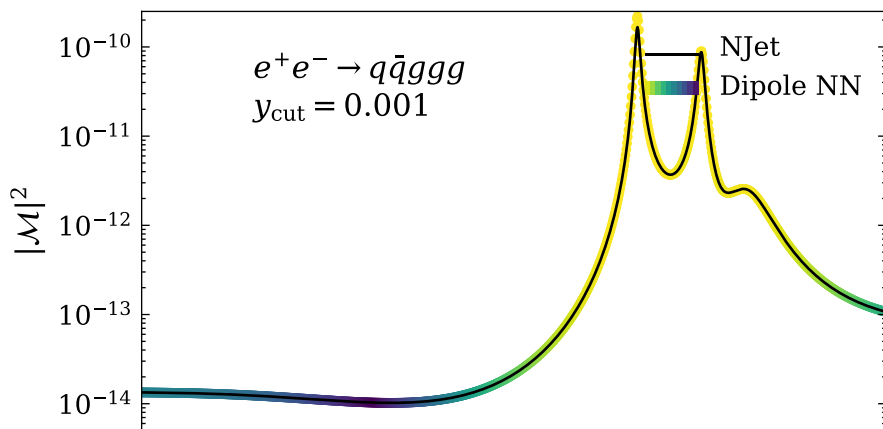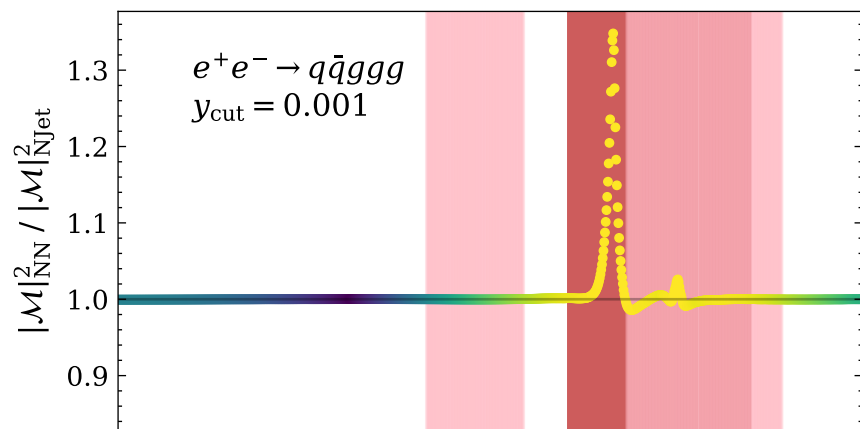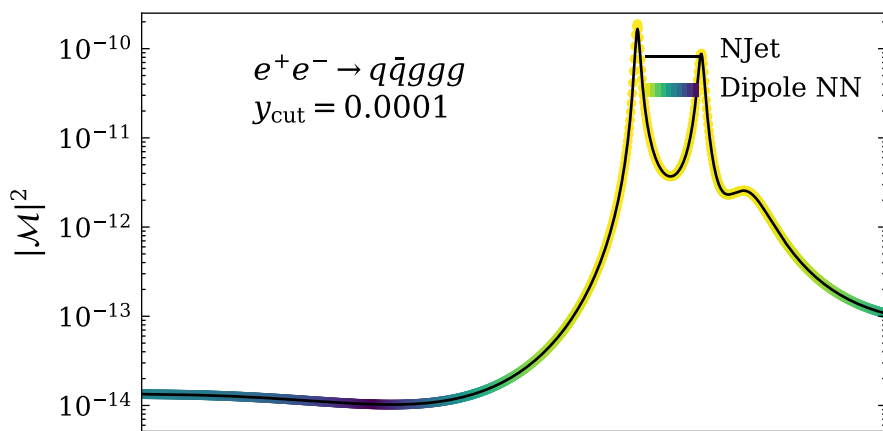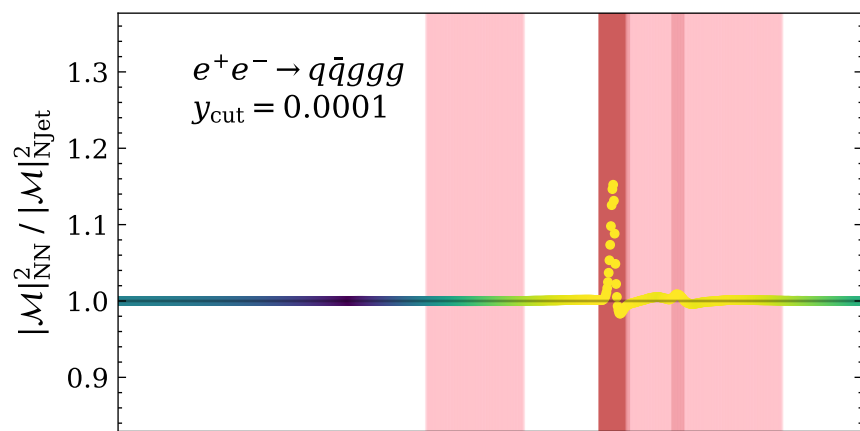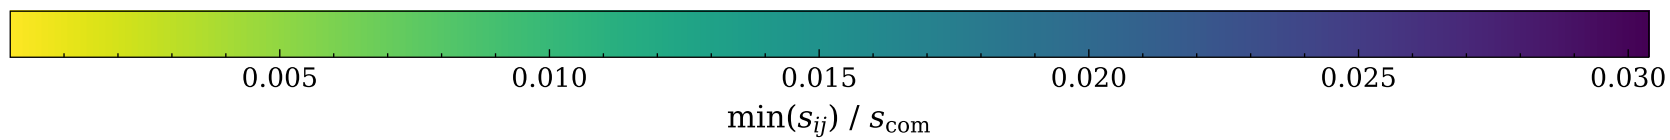

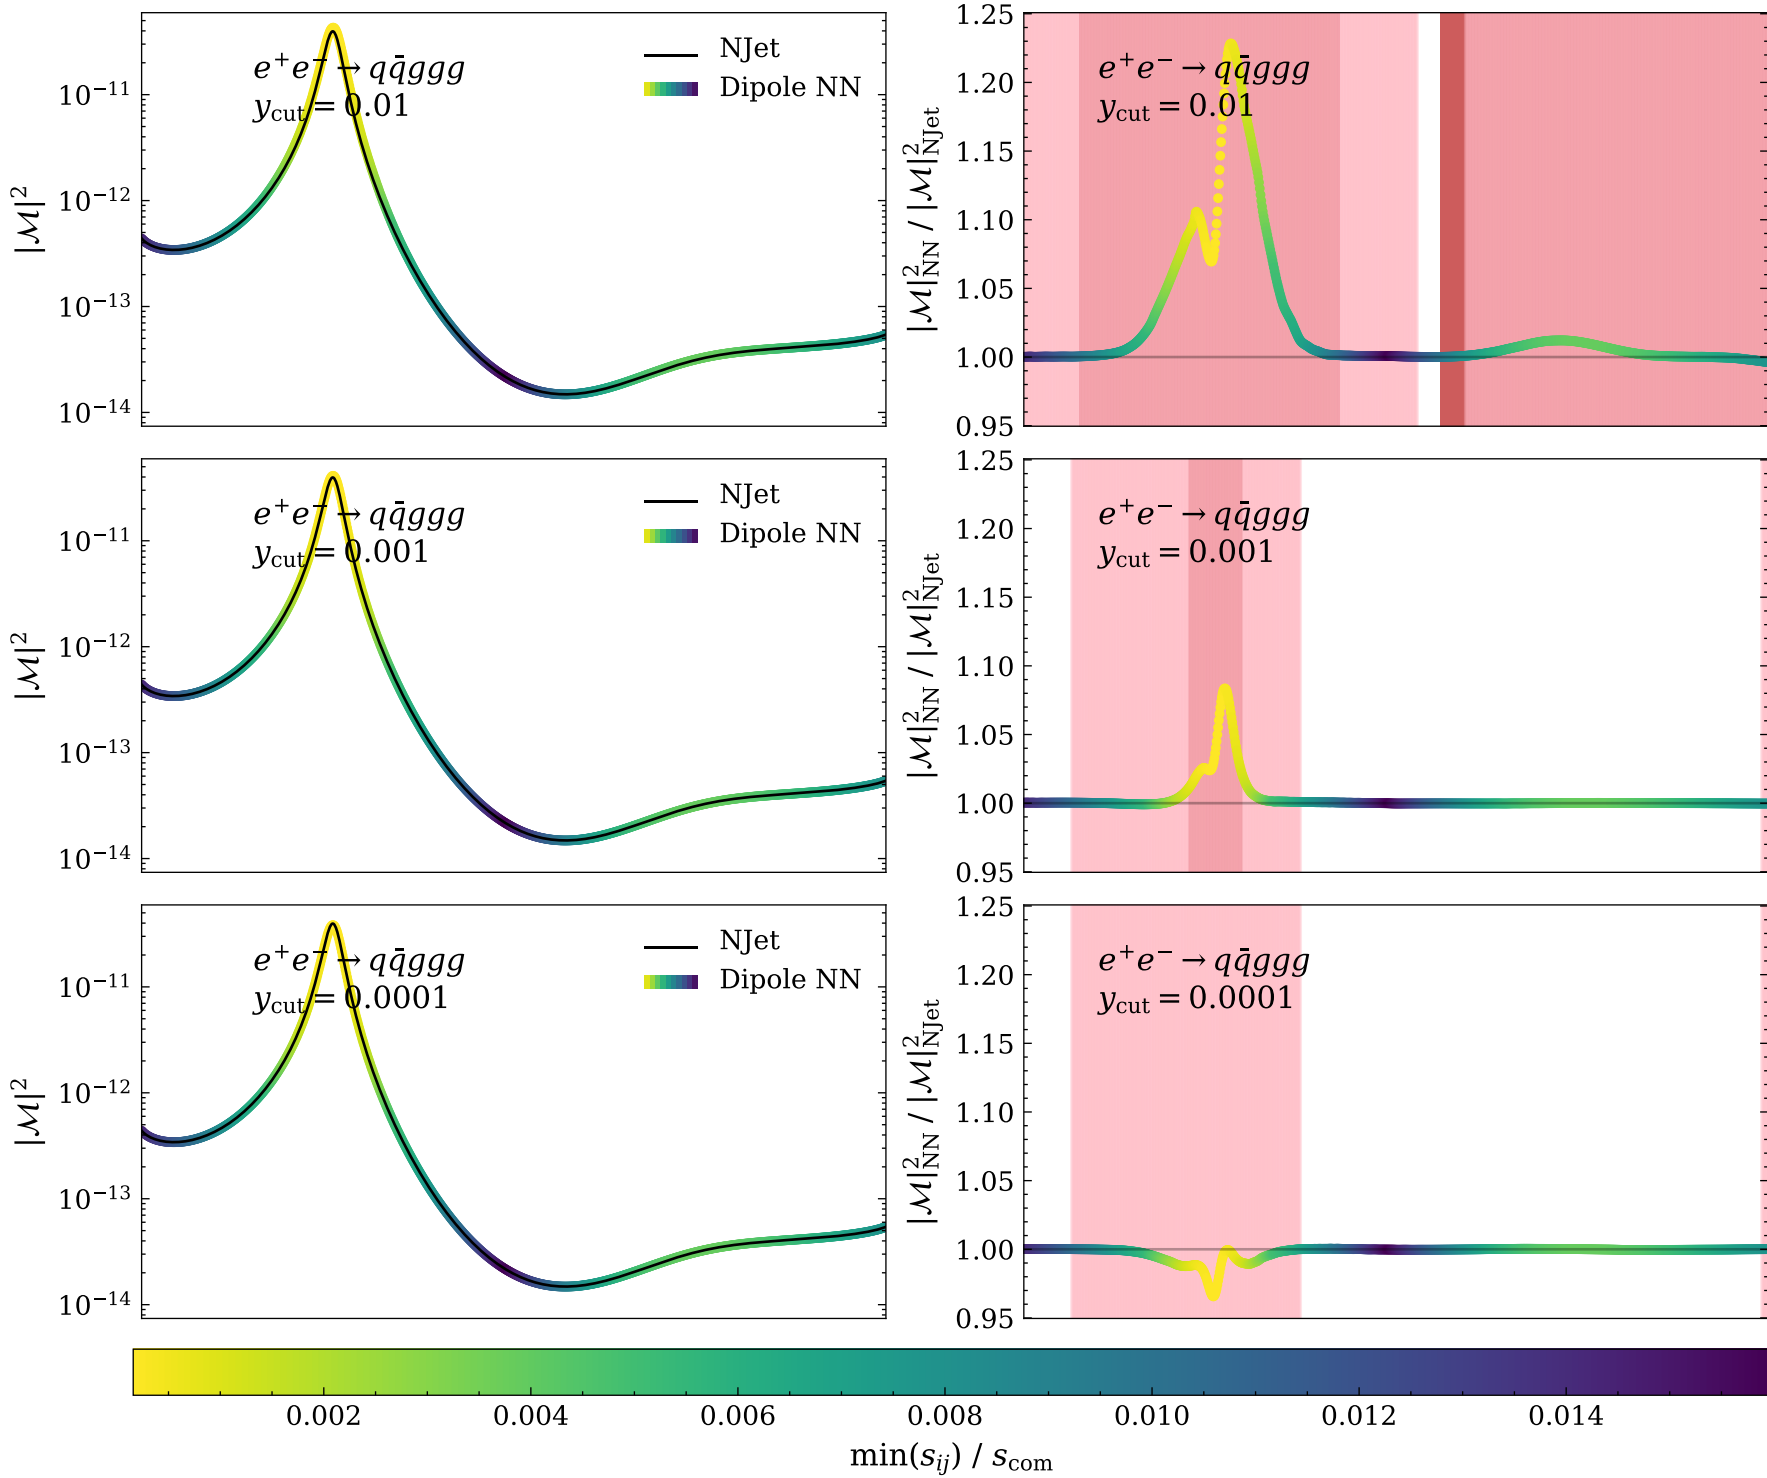

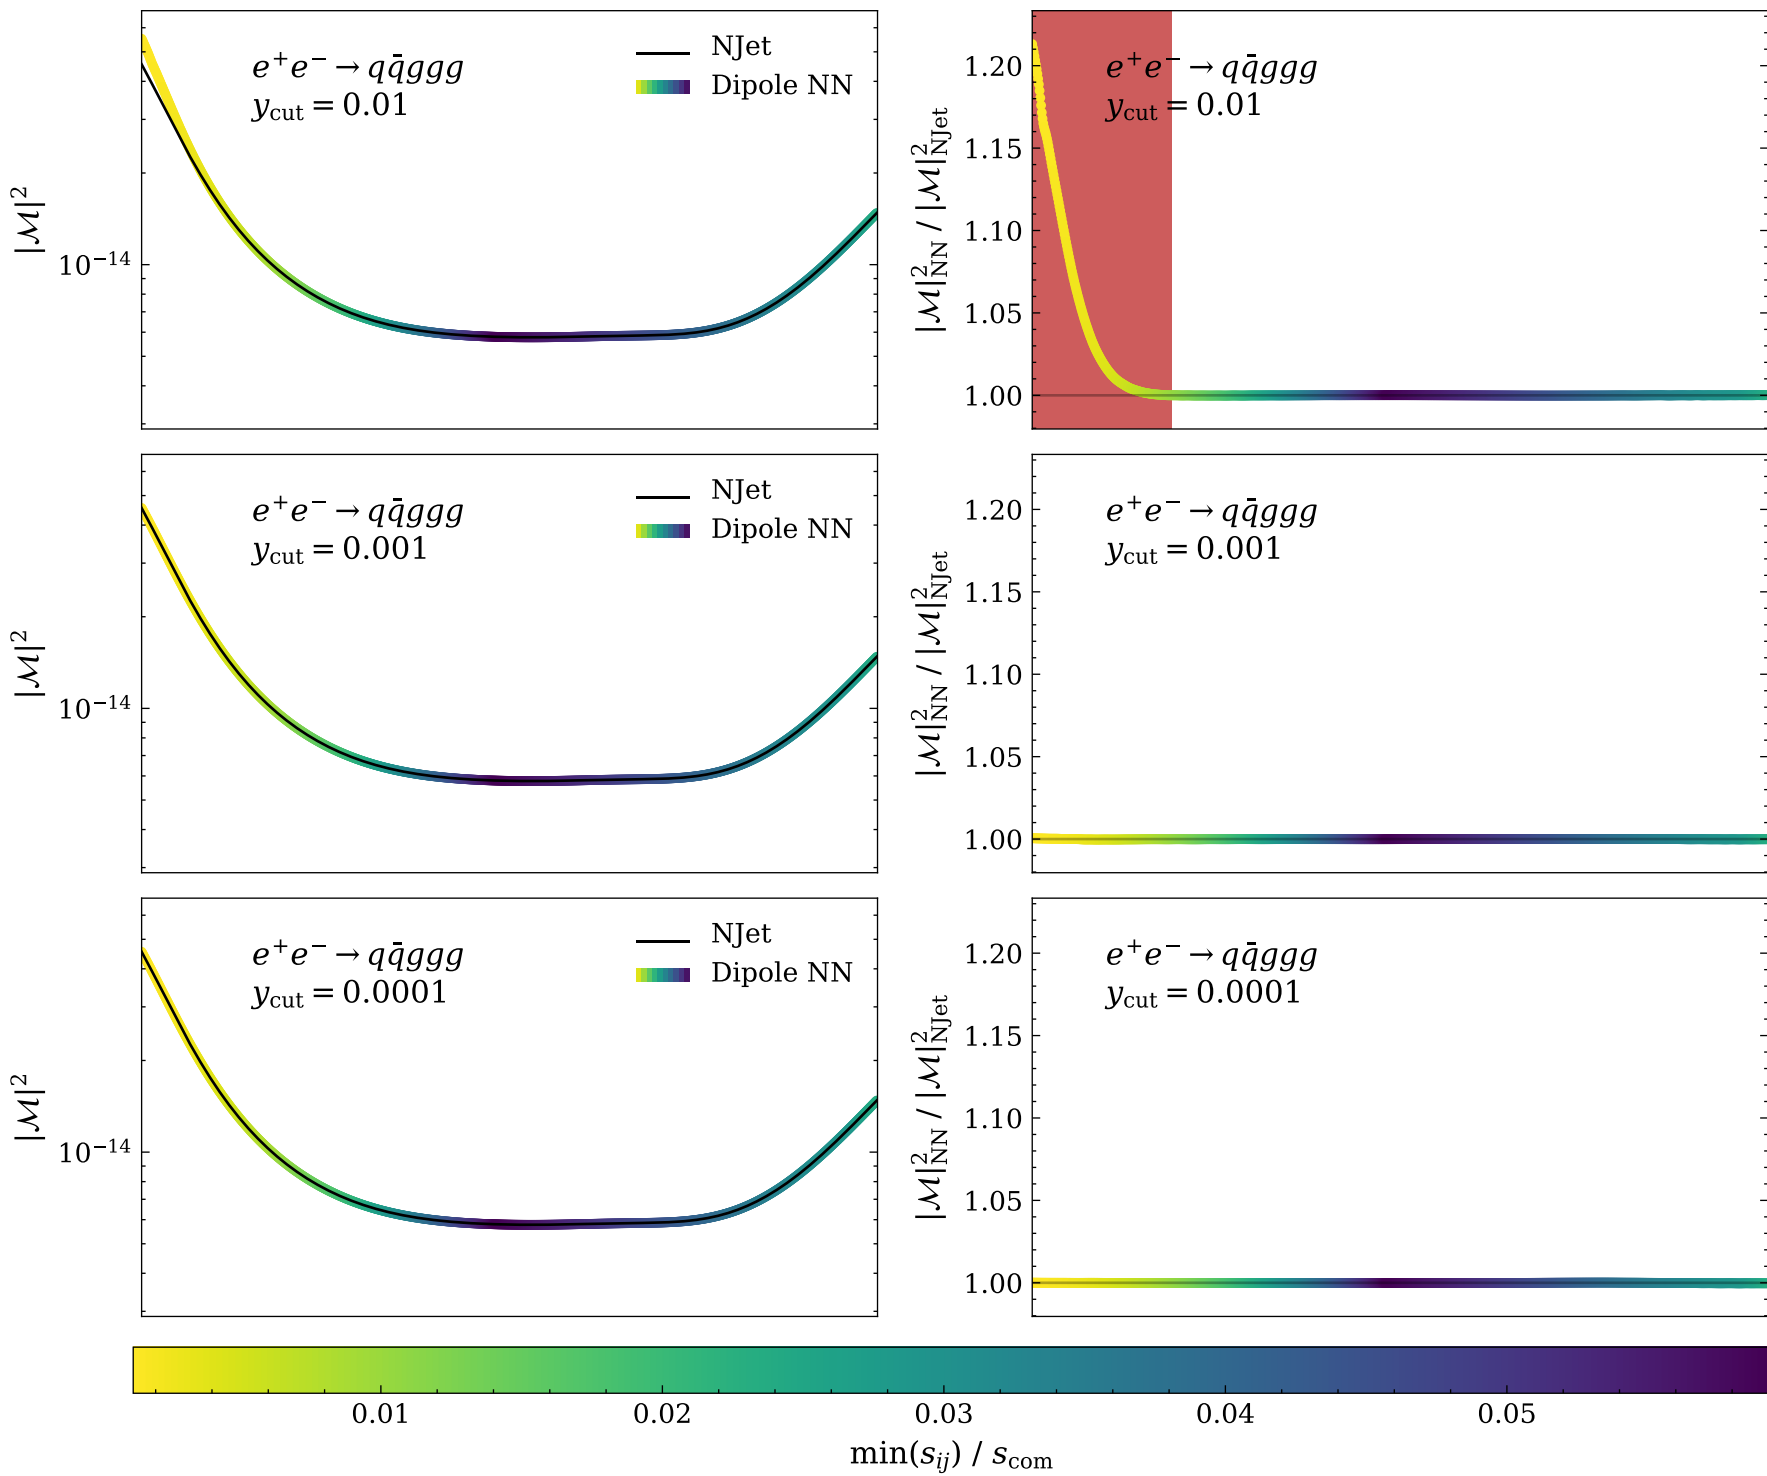

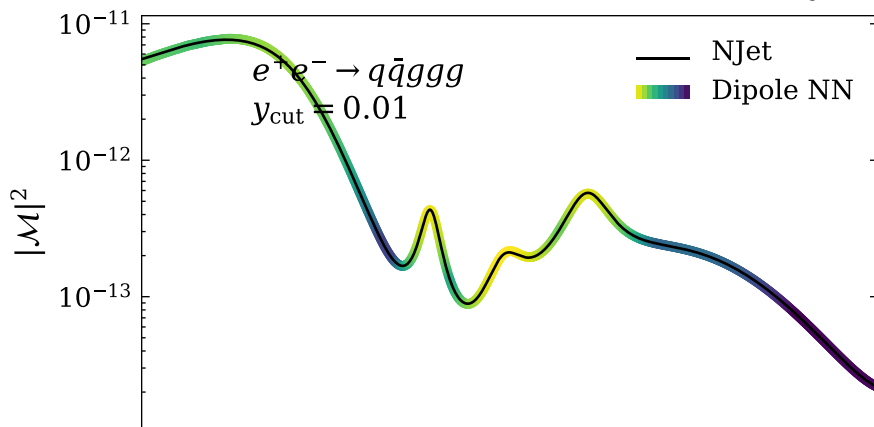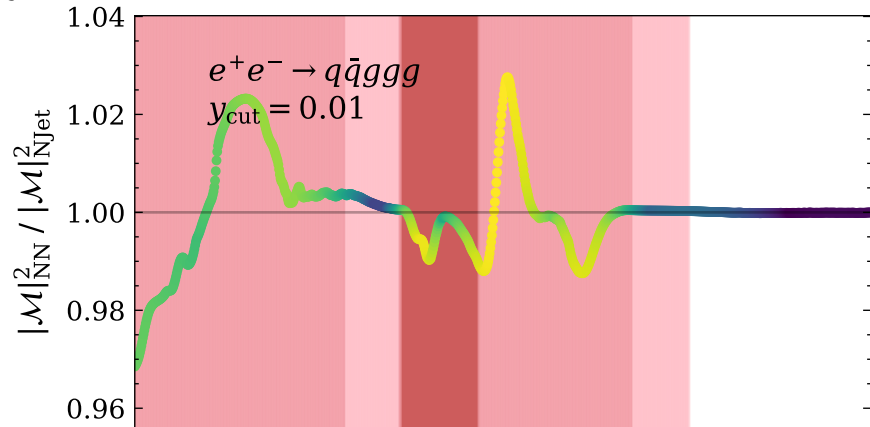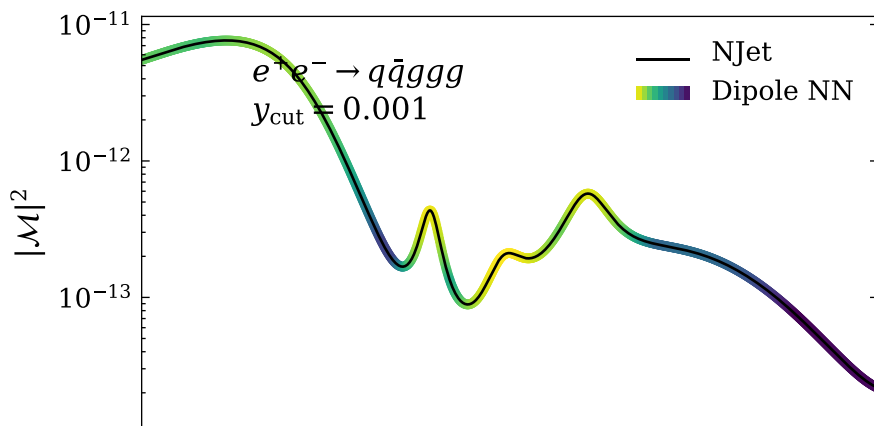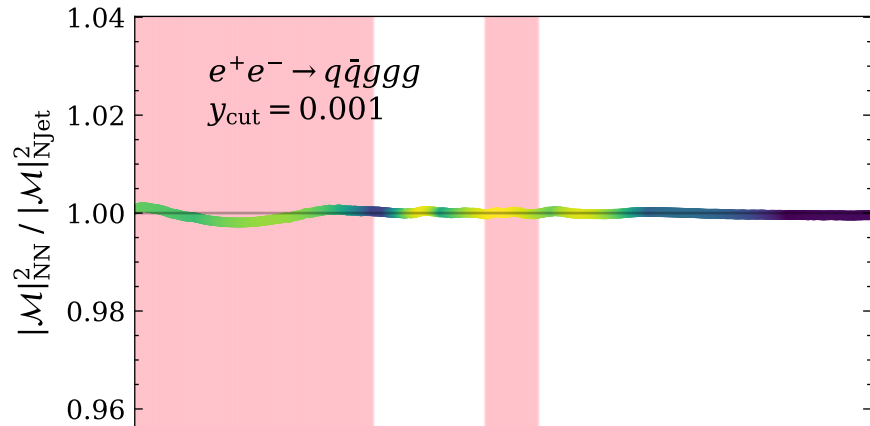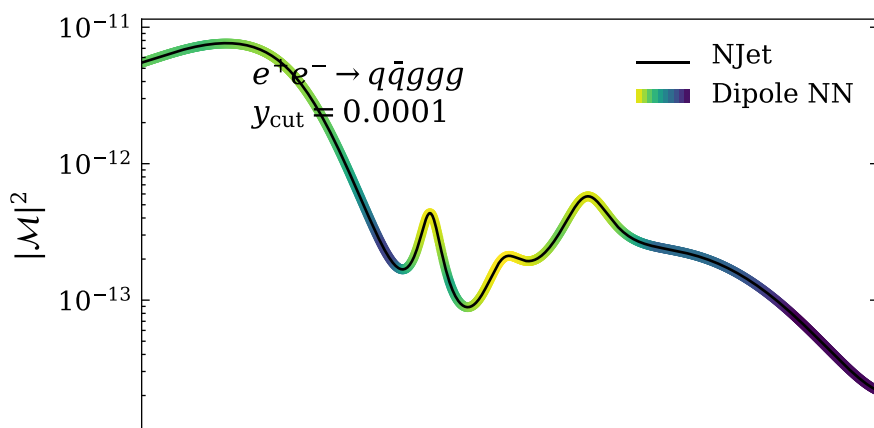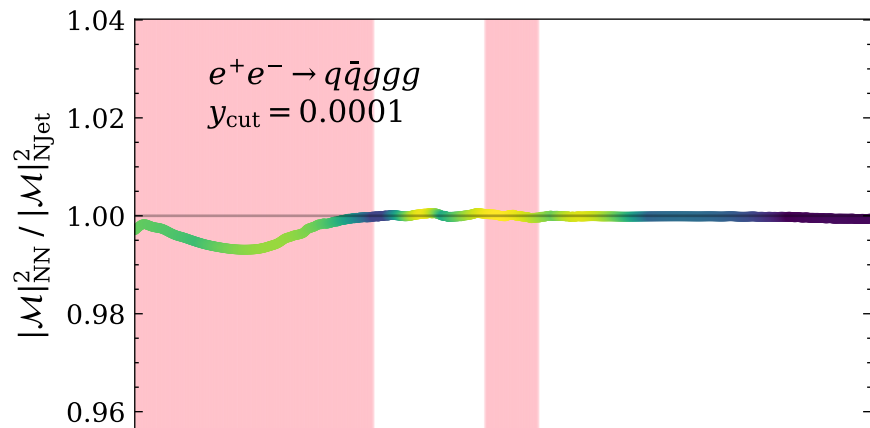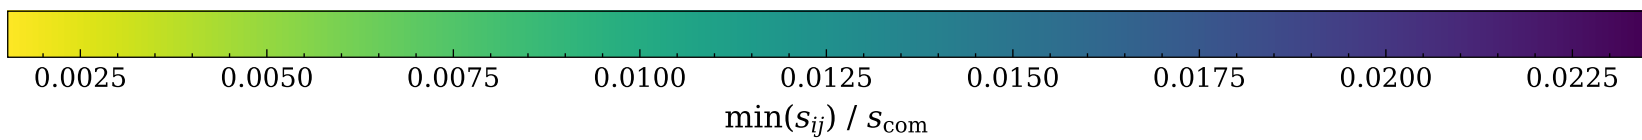

Trajectory 1256

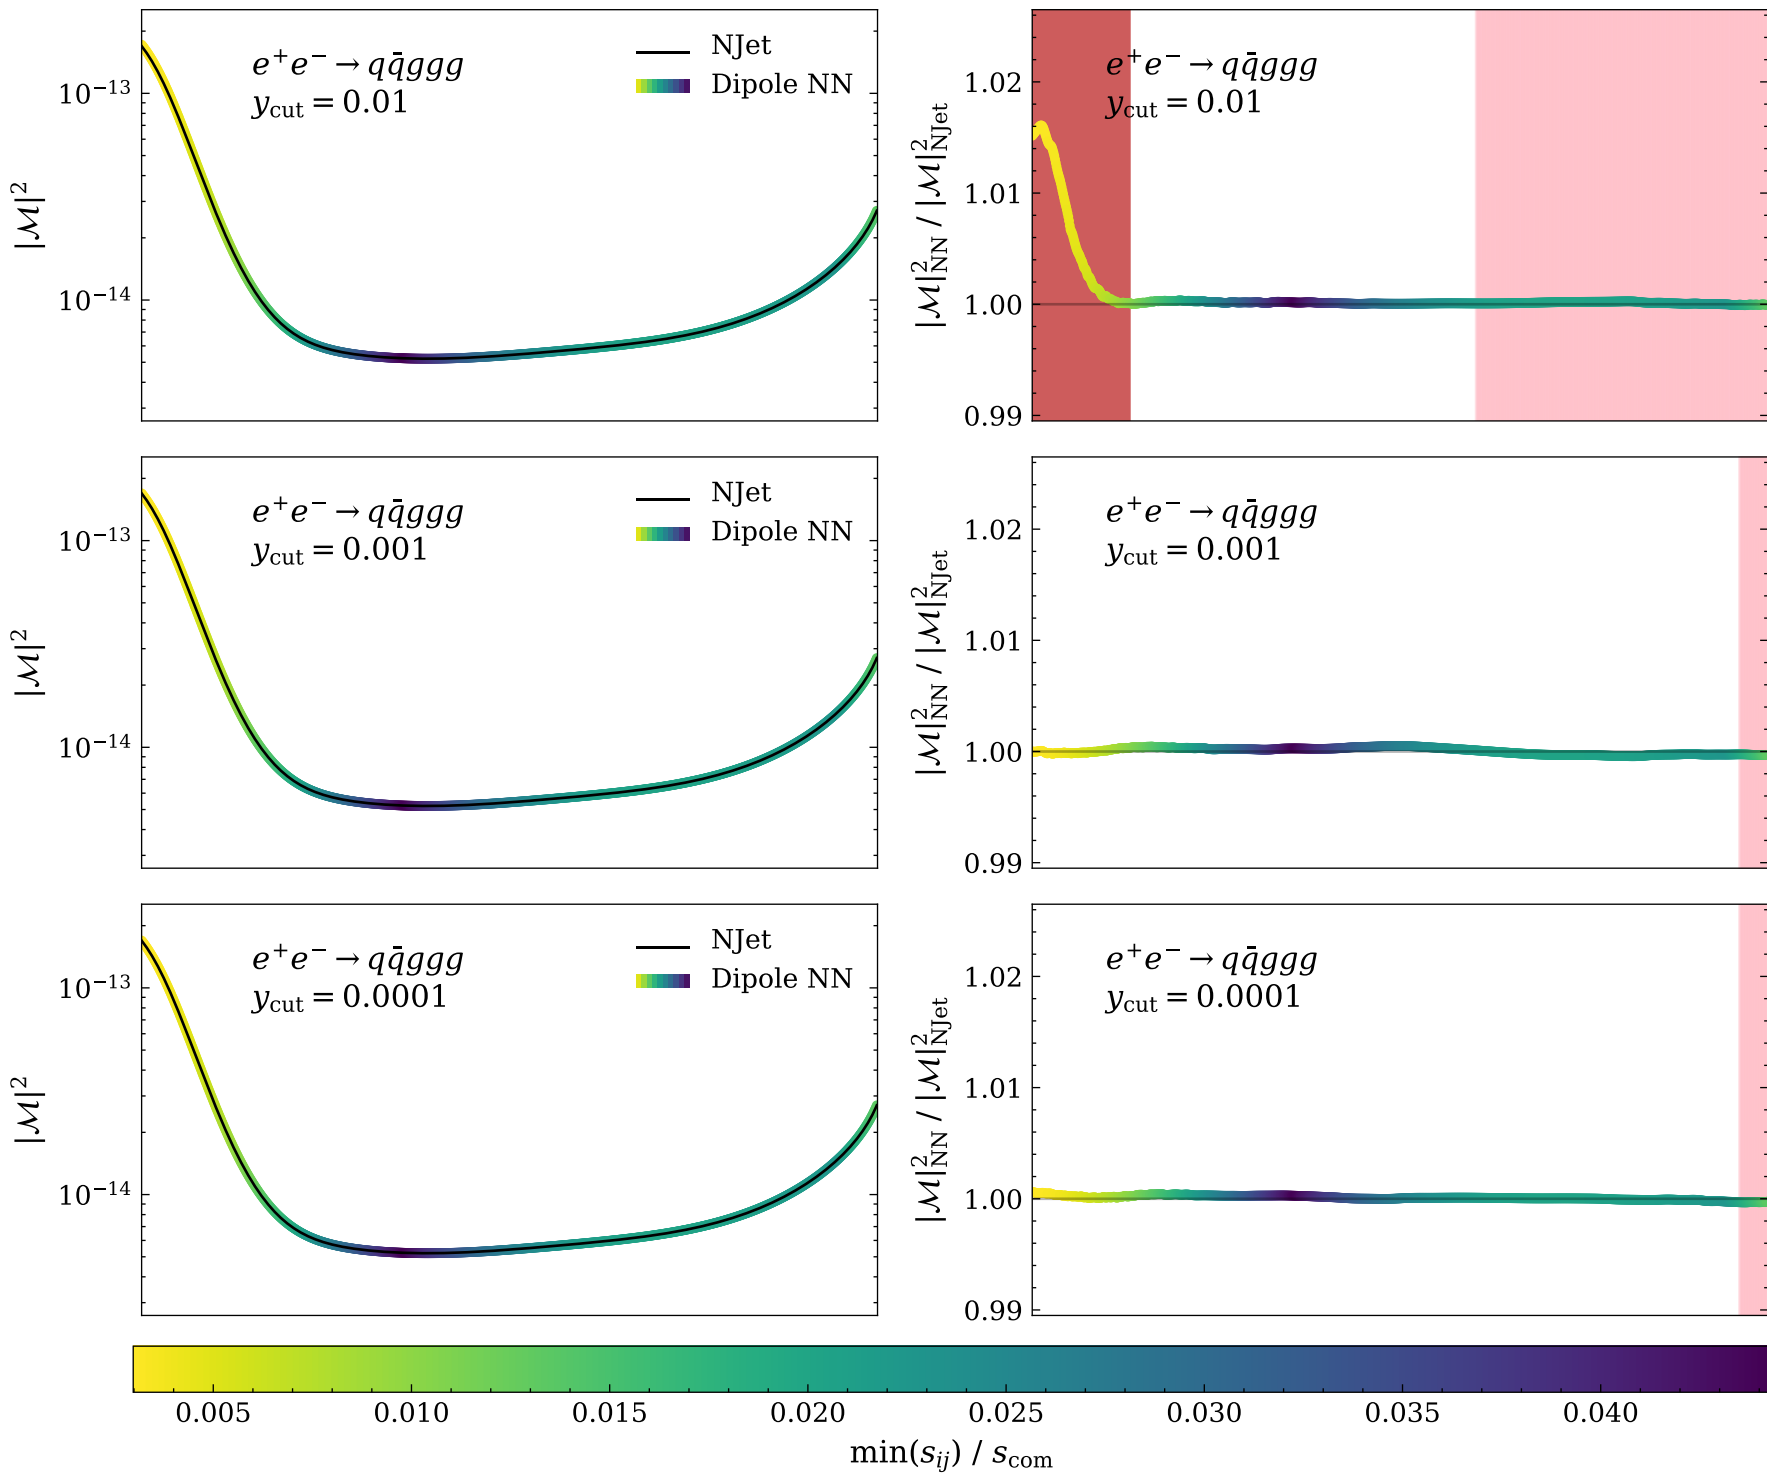

Trajectory 1257

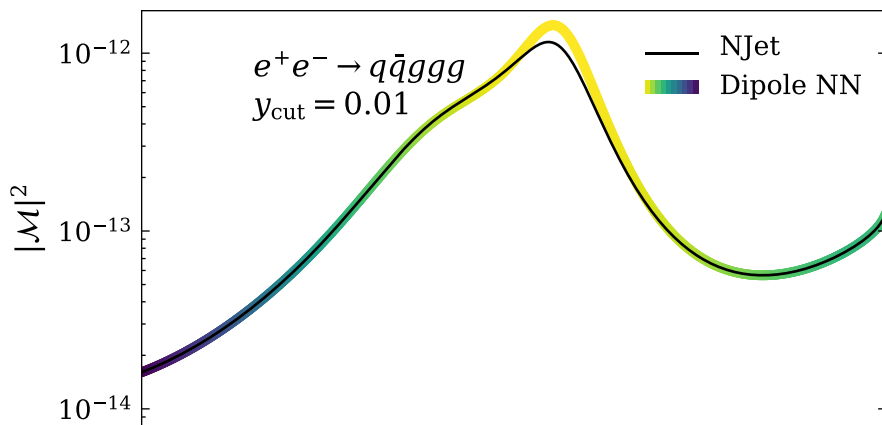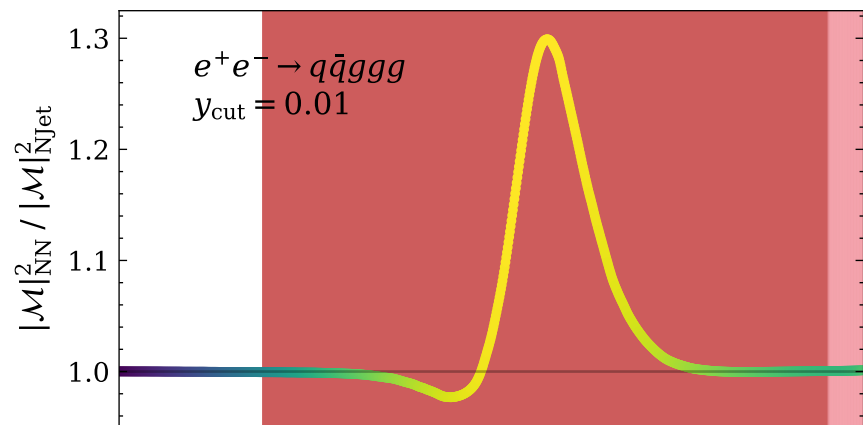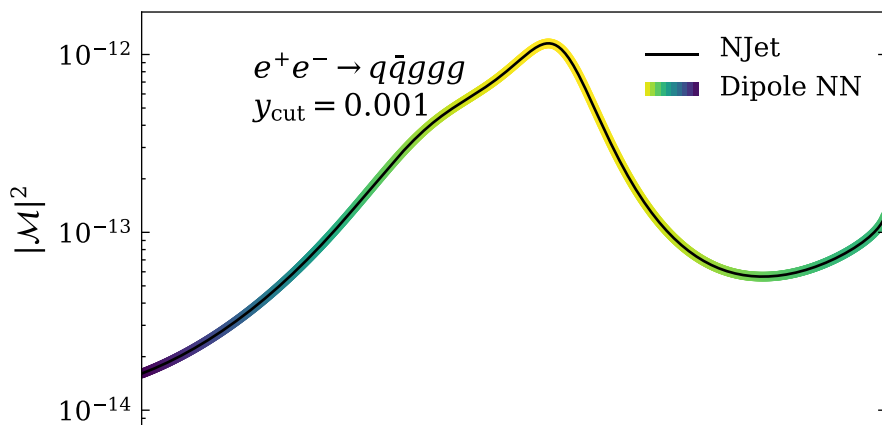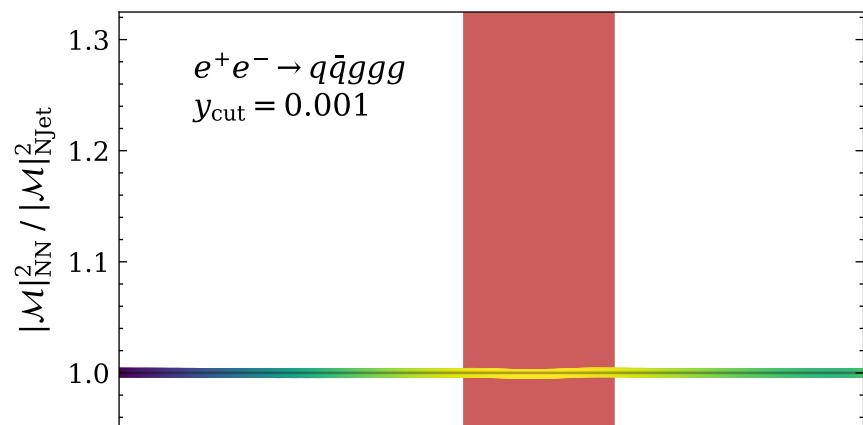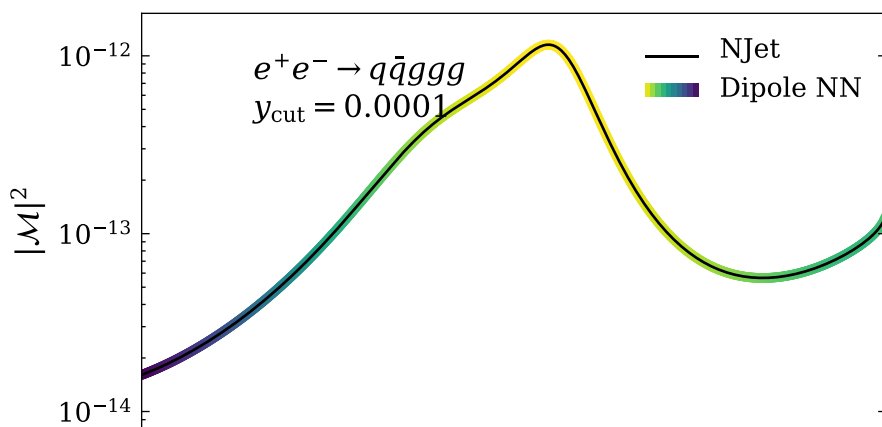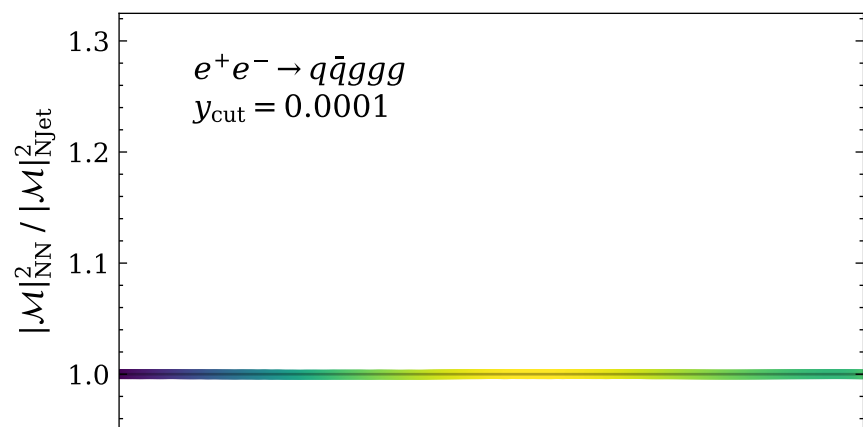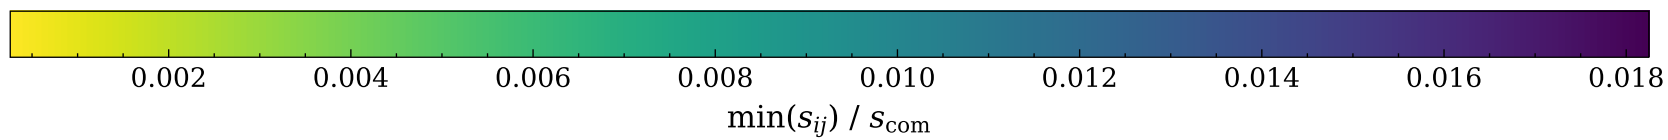

Trajectory 1258

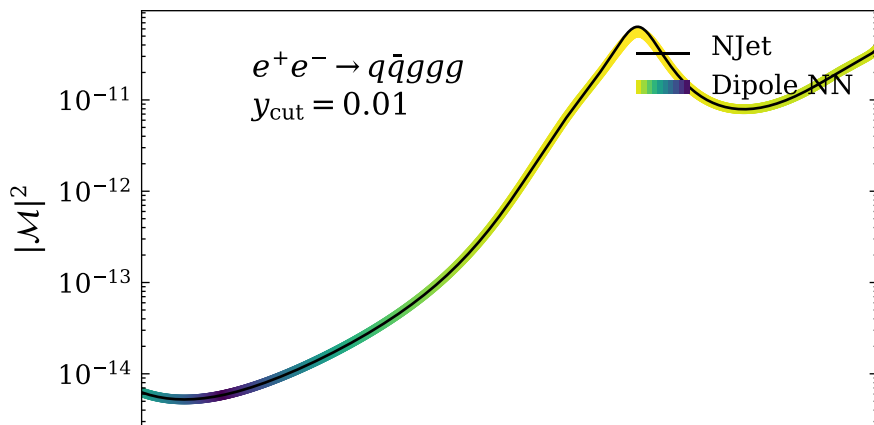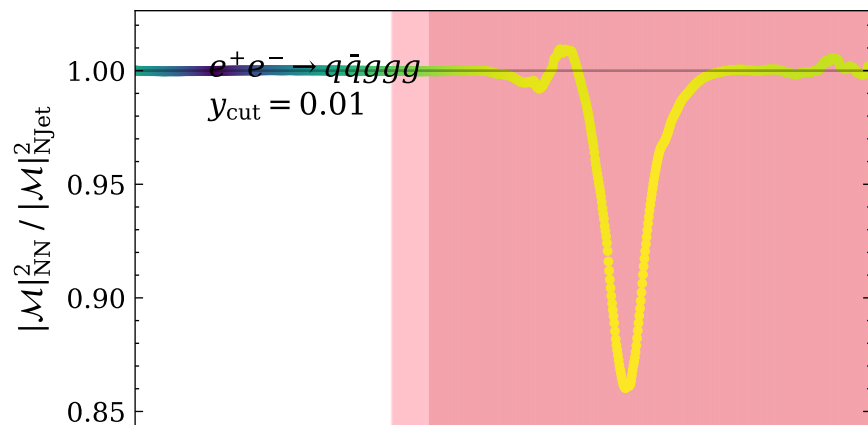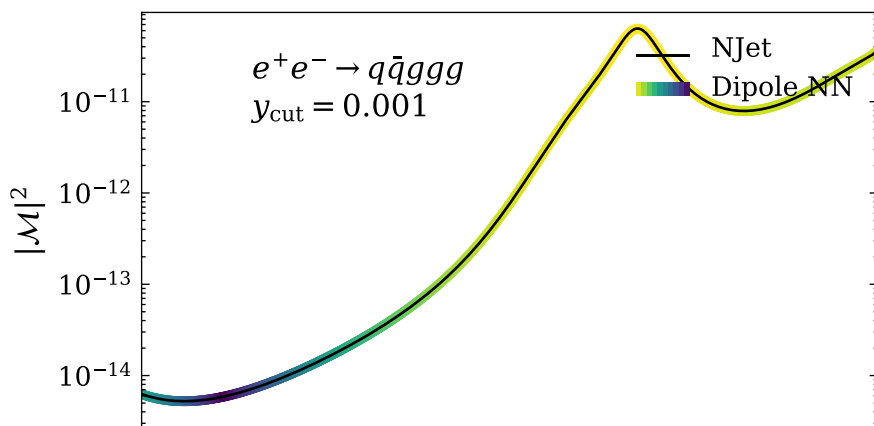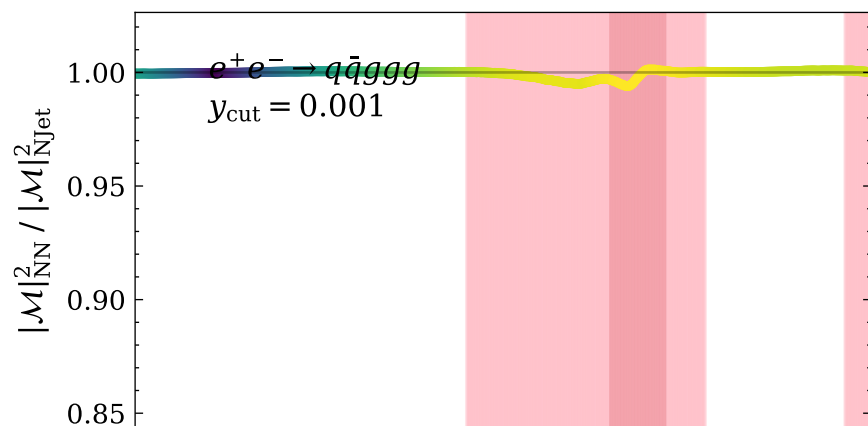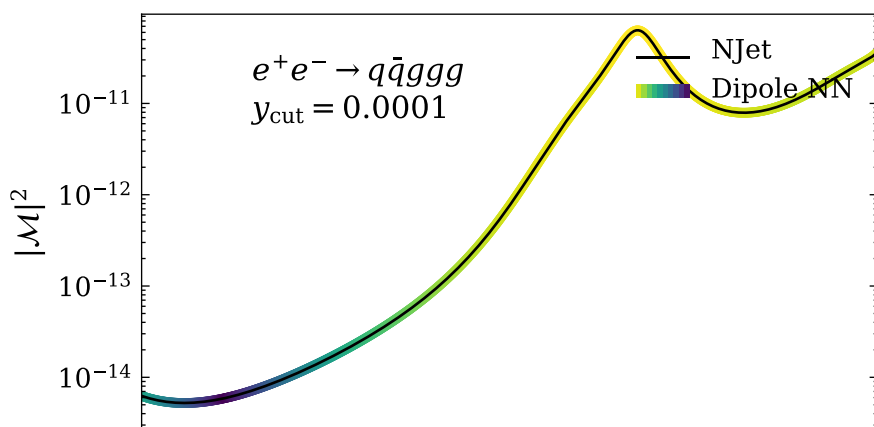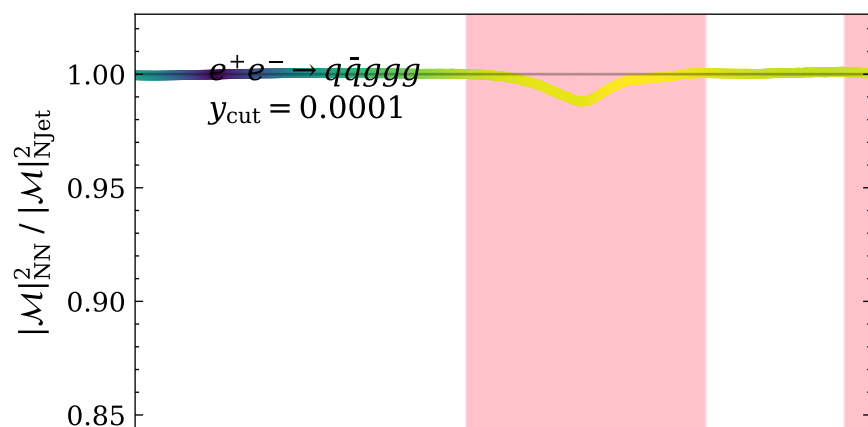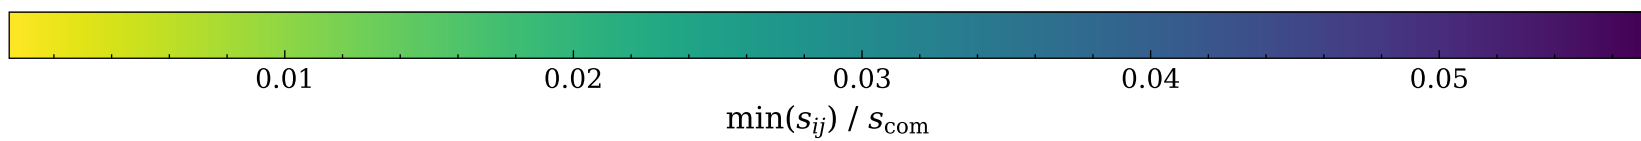

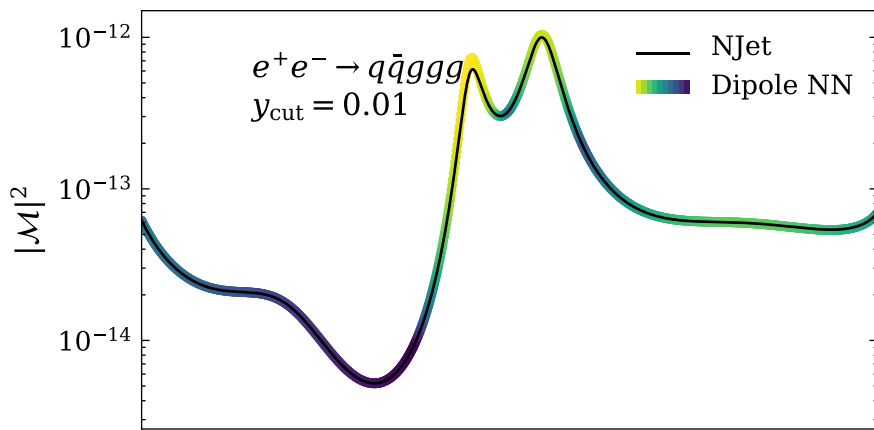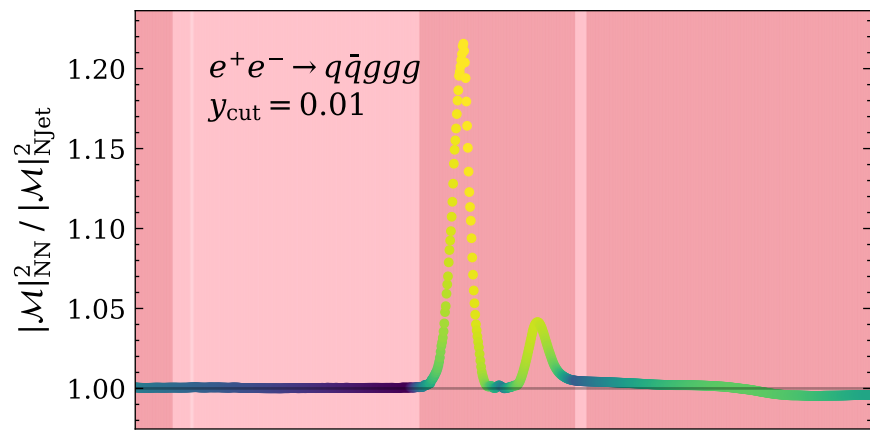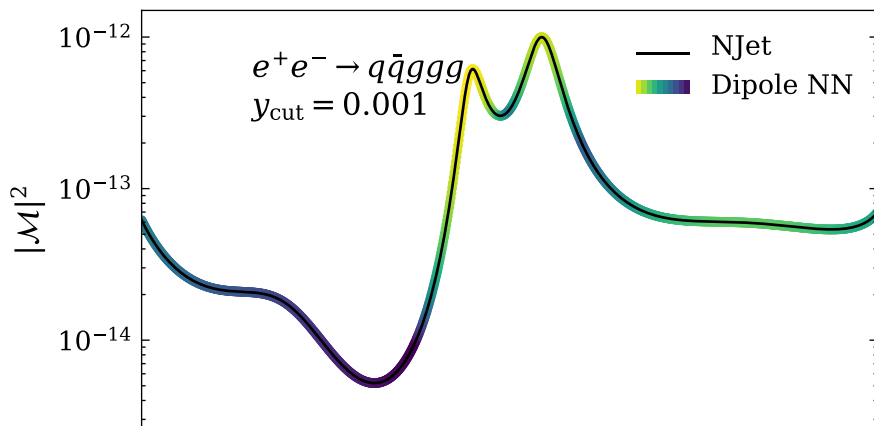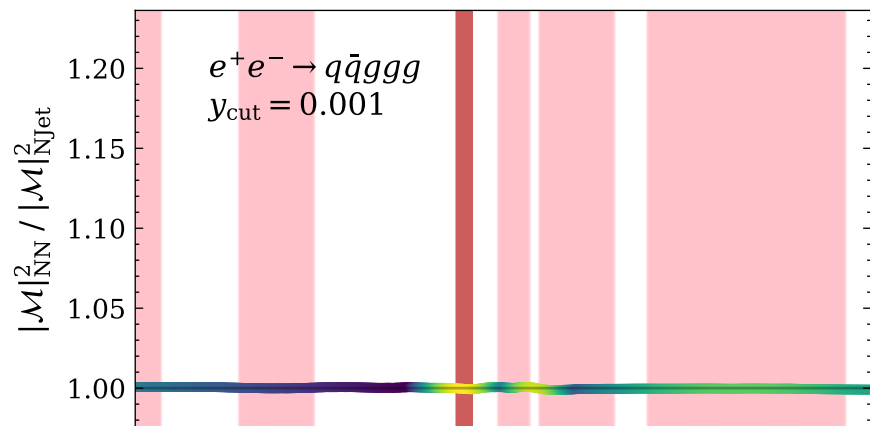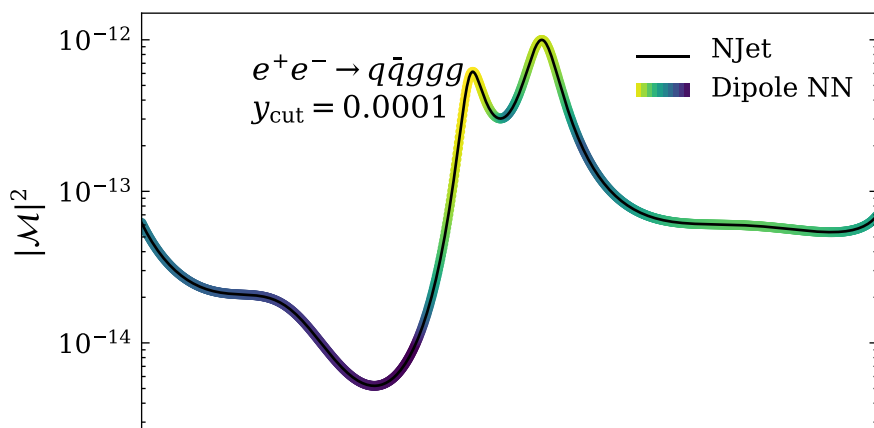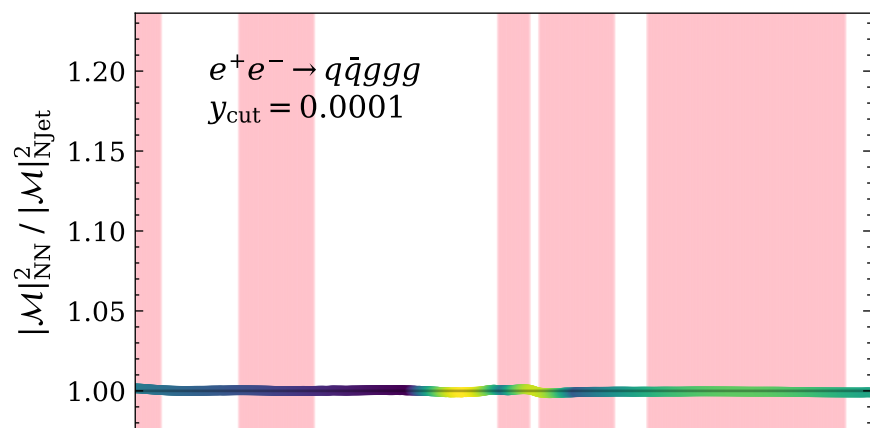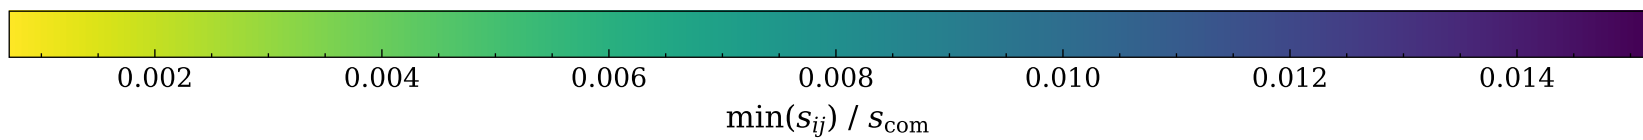

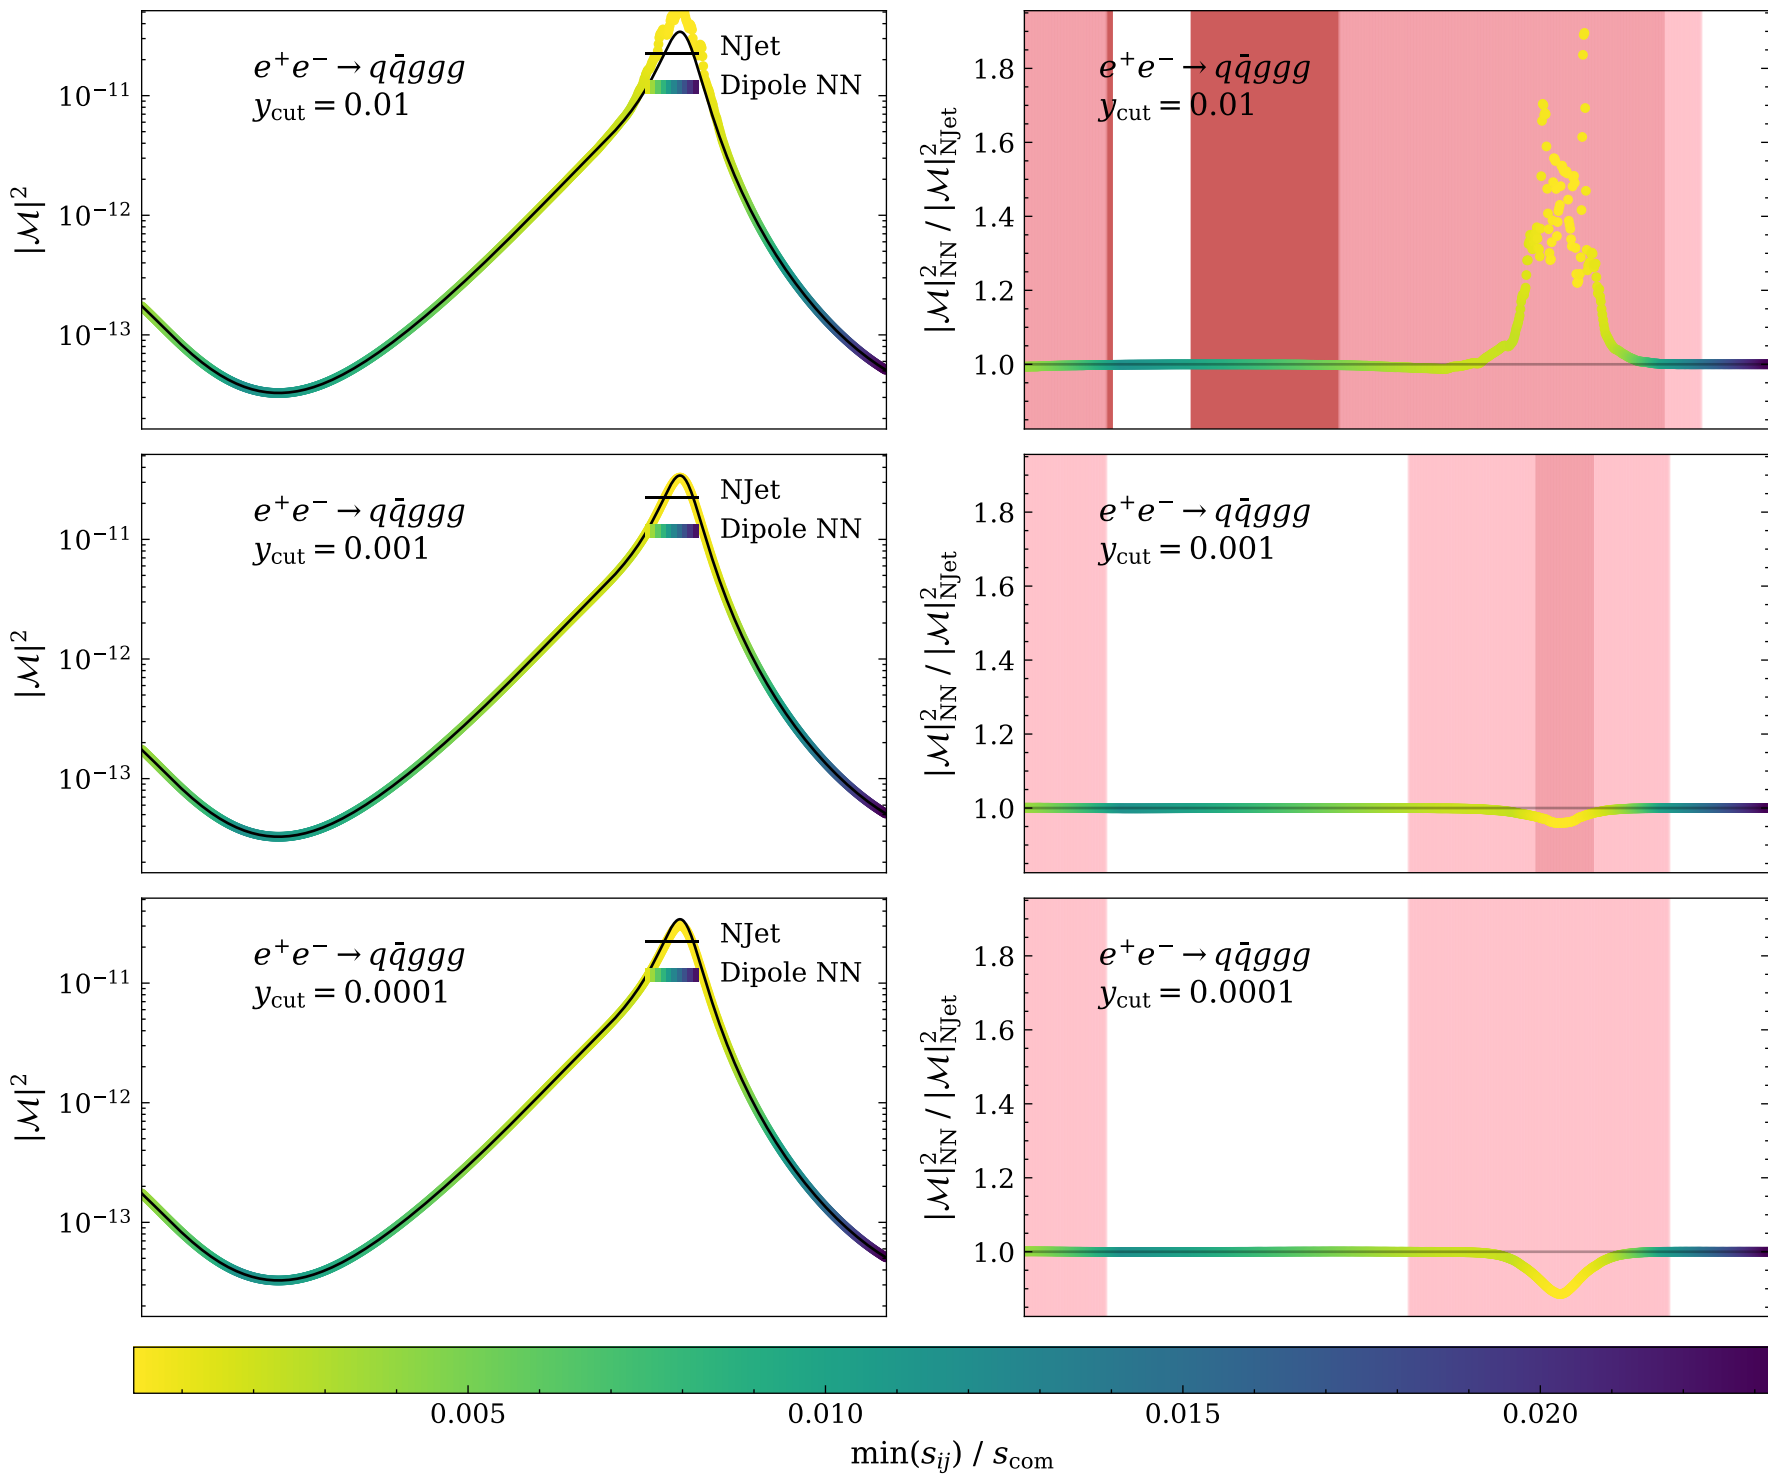

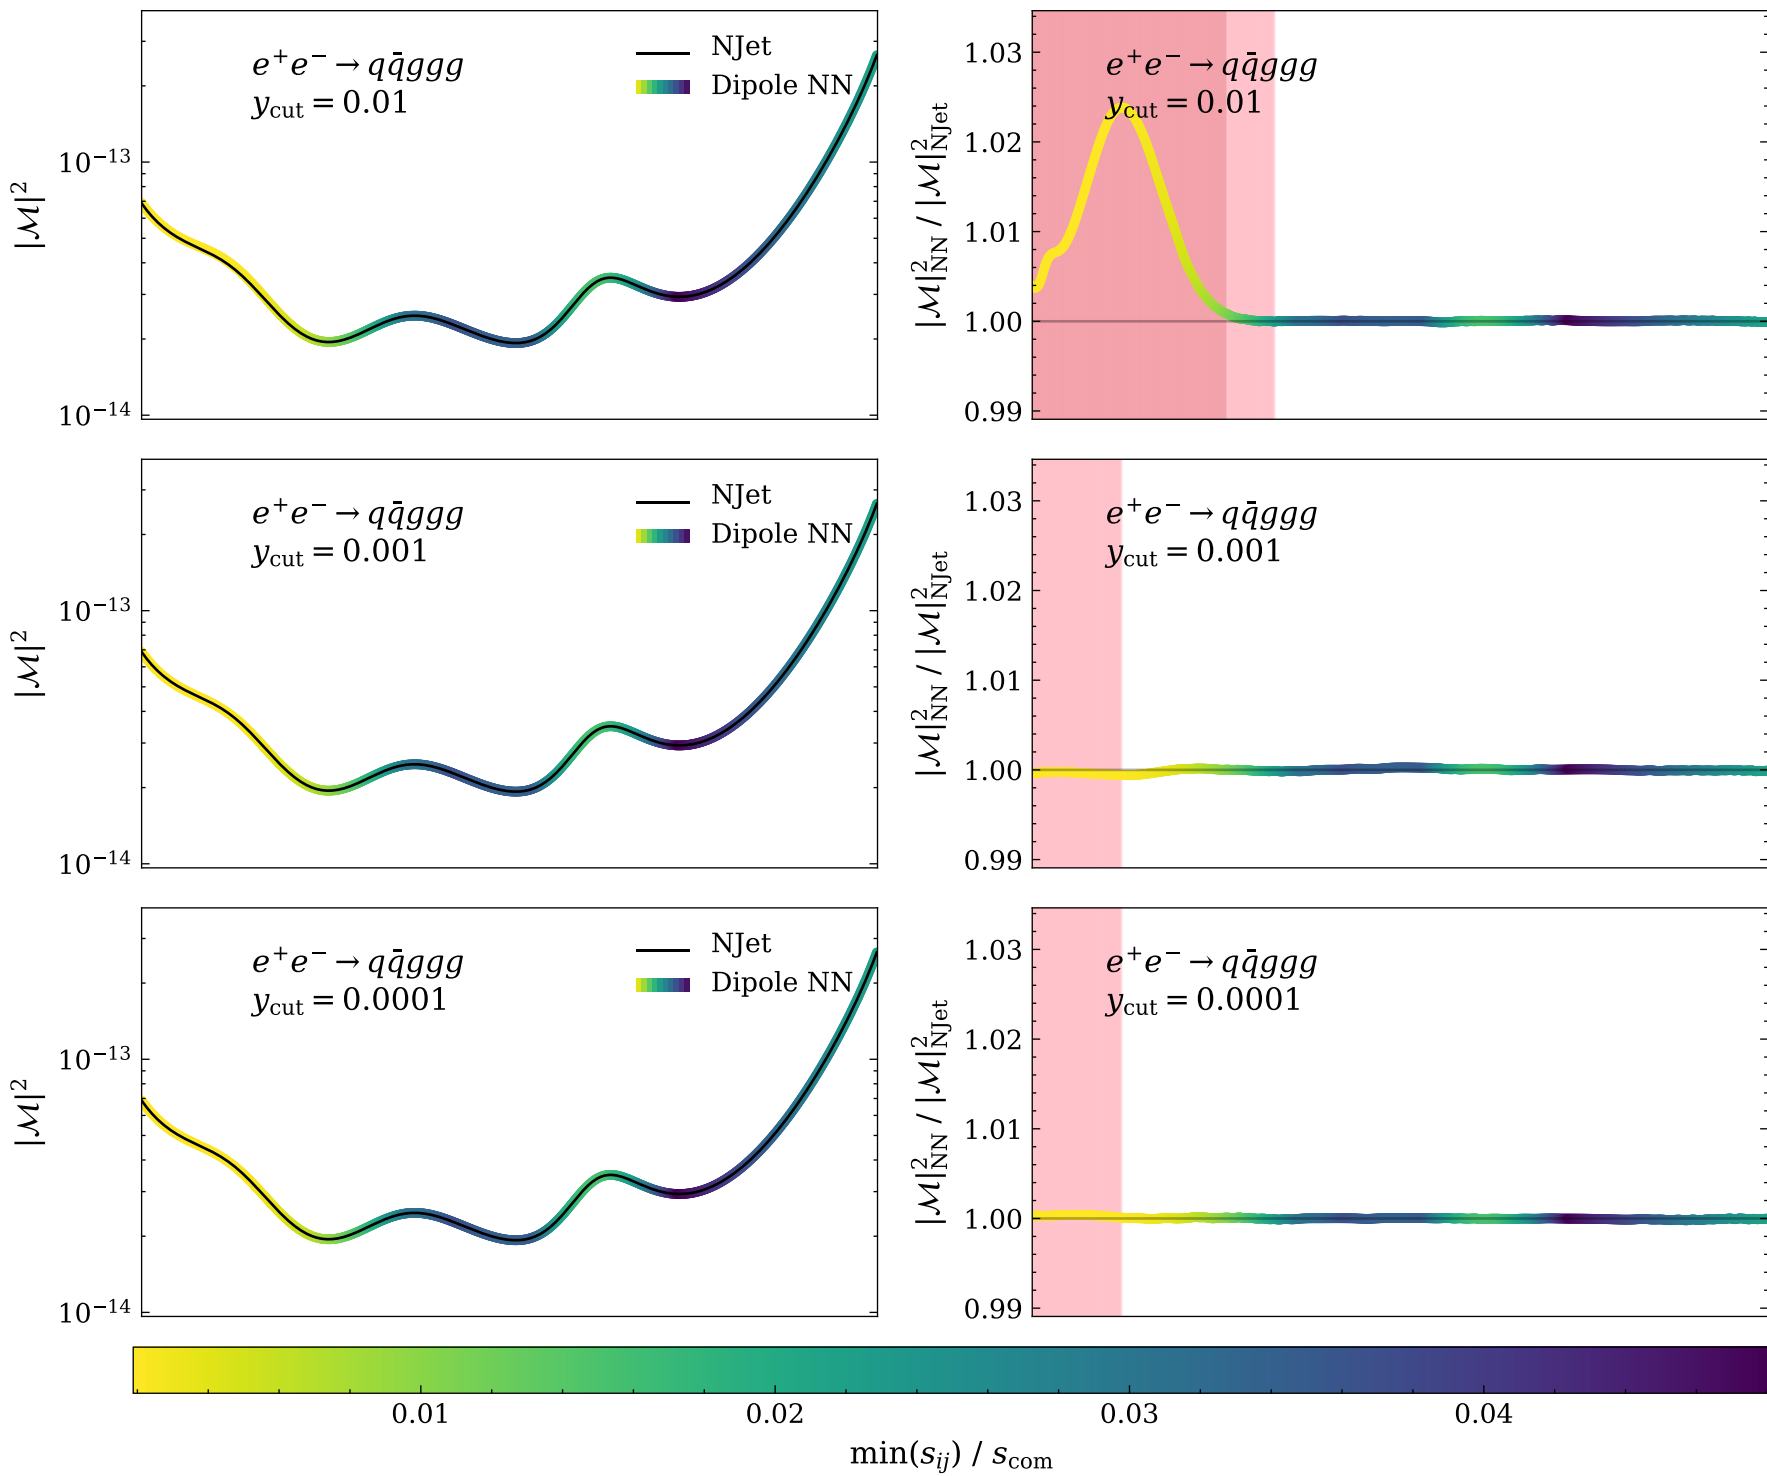

Trajectory 1262

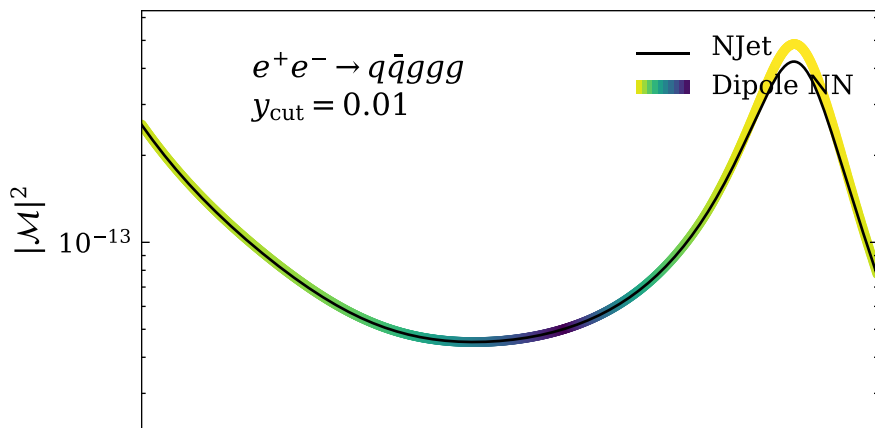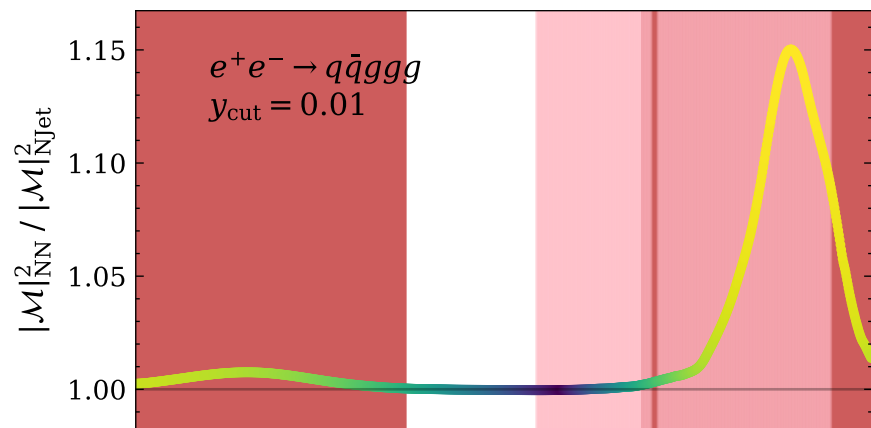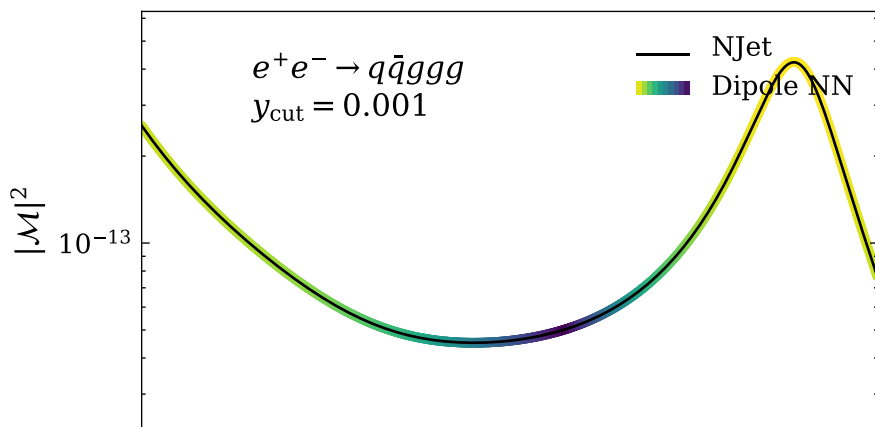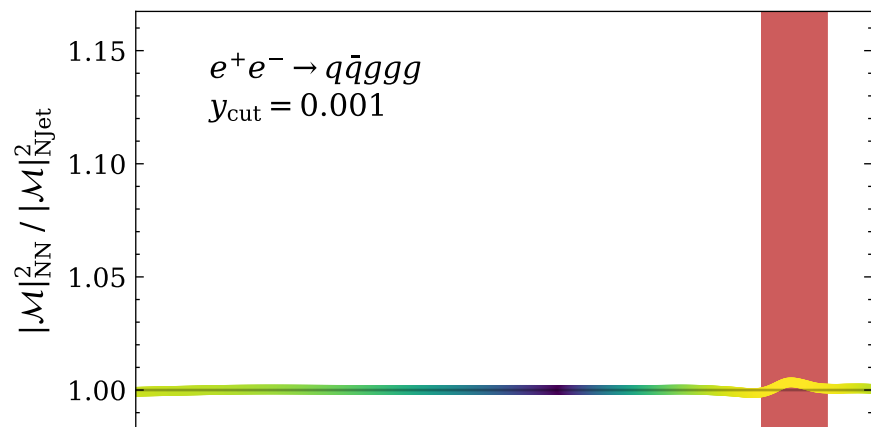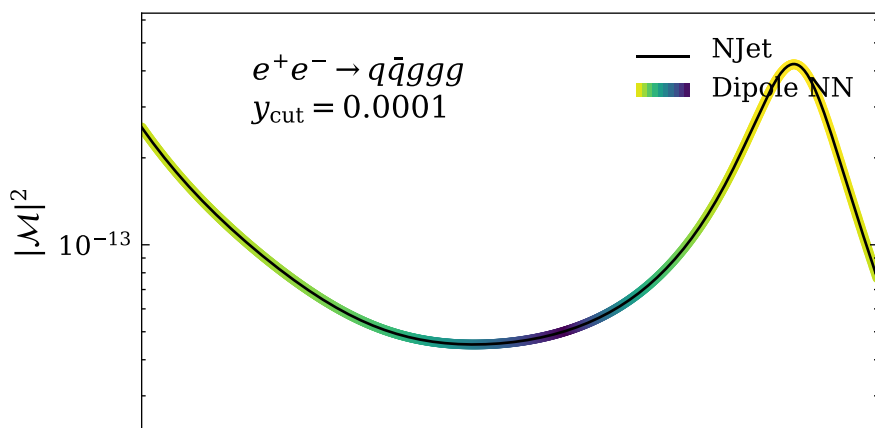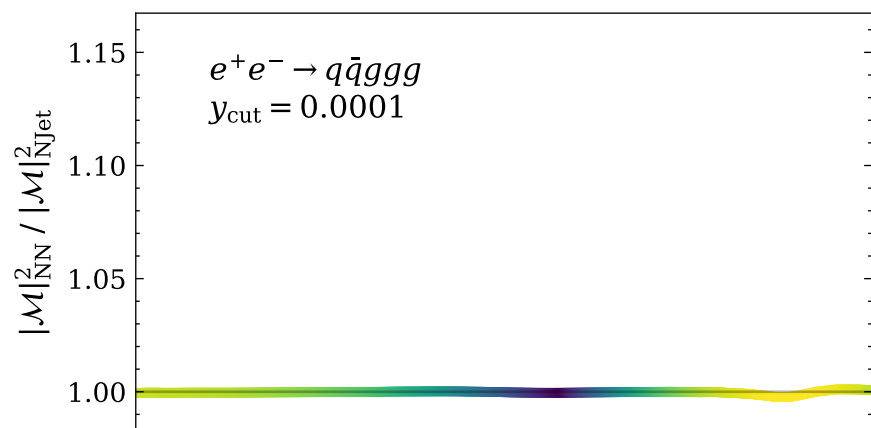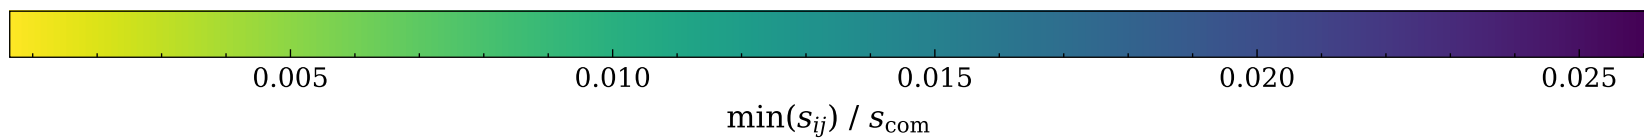

Trajectory 1263

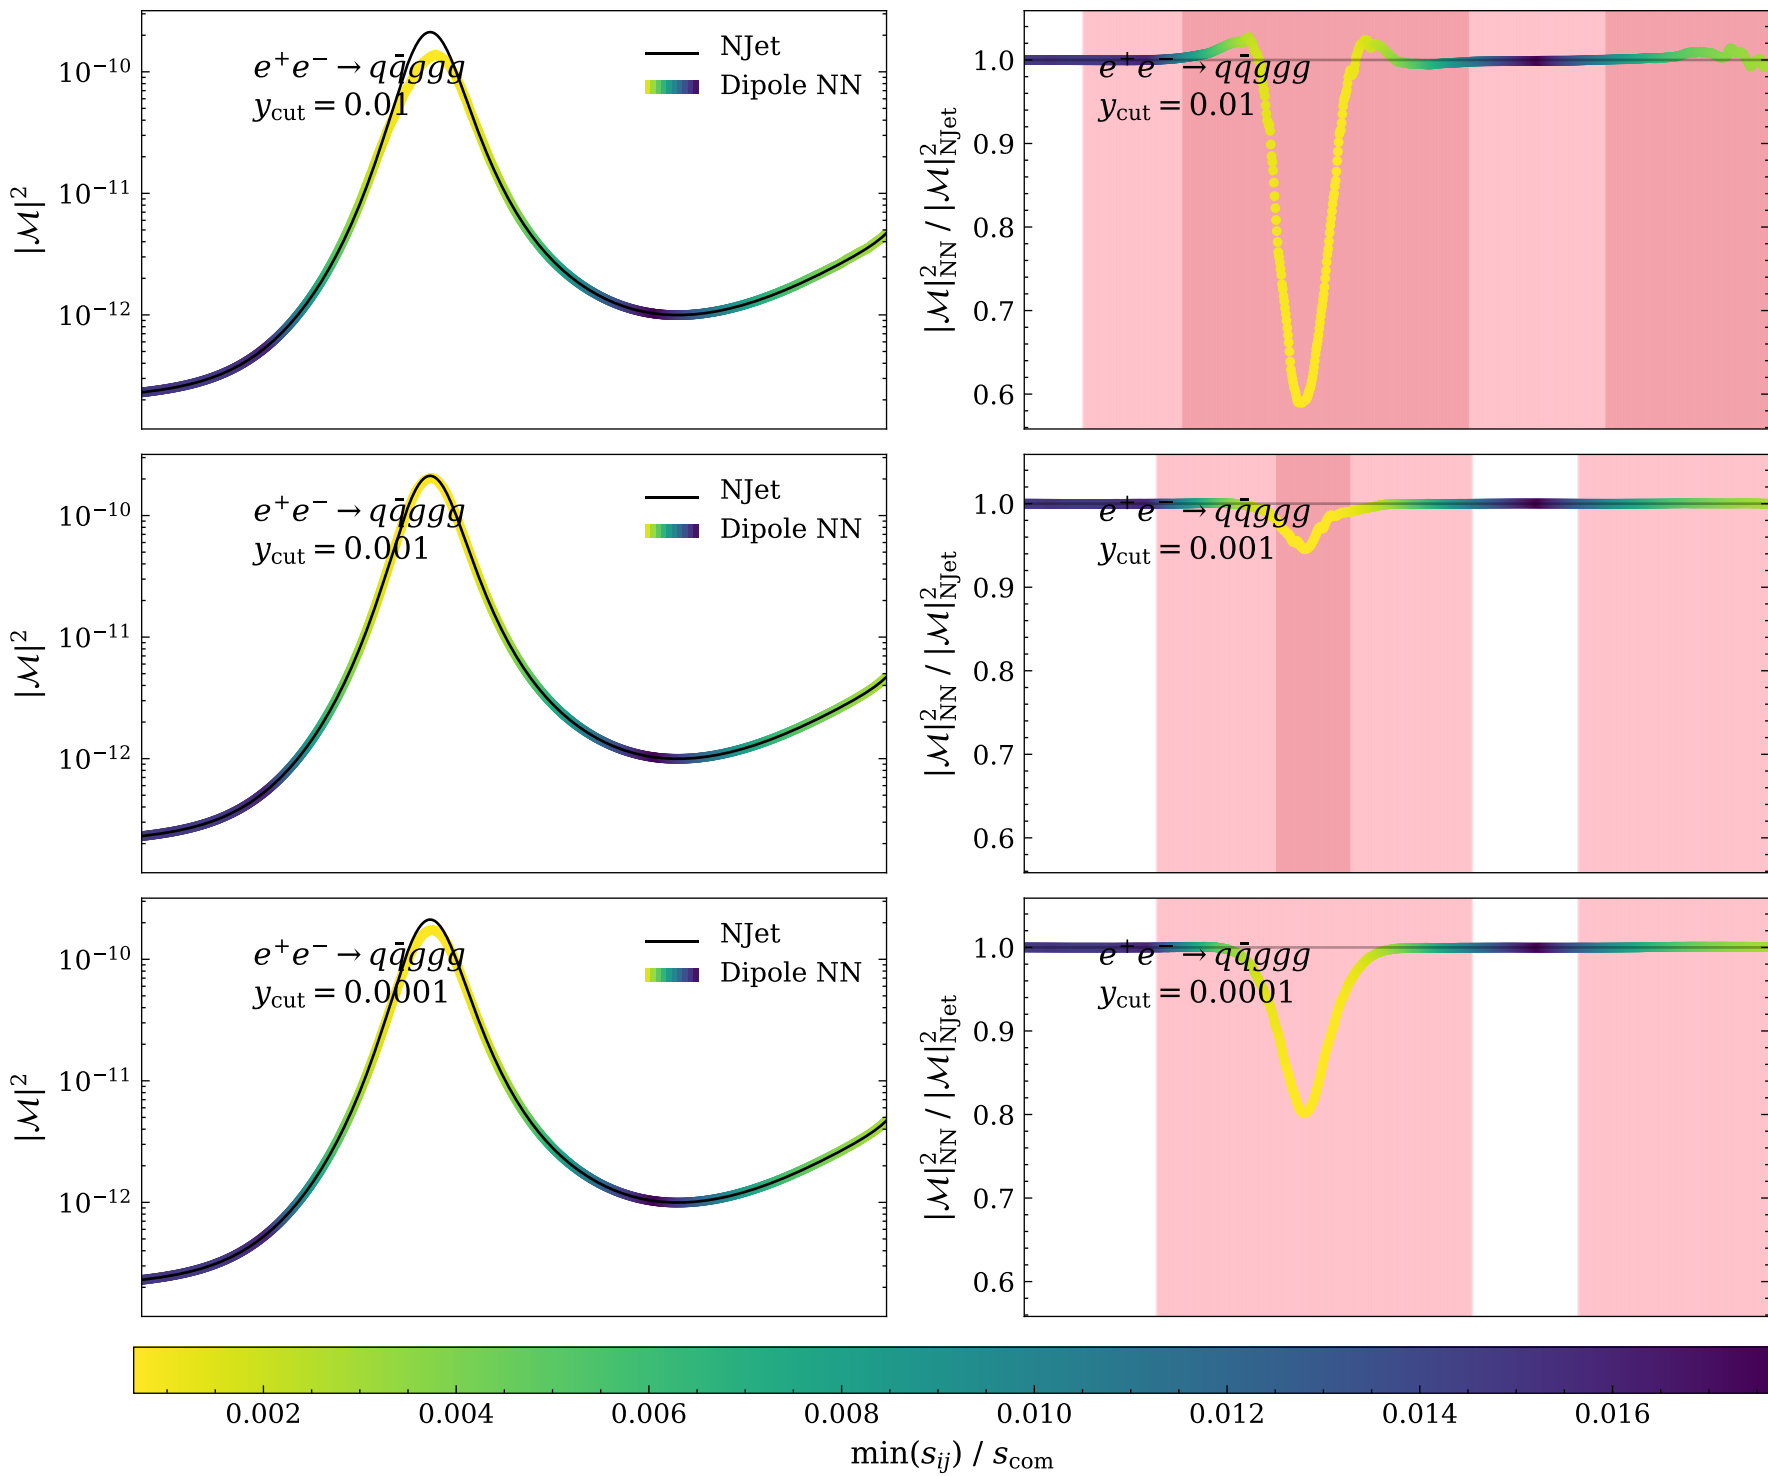

Trajectory 1264

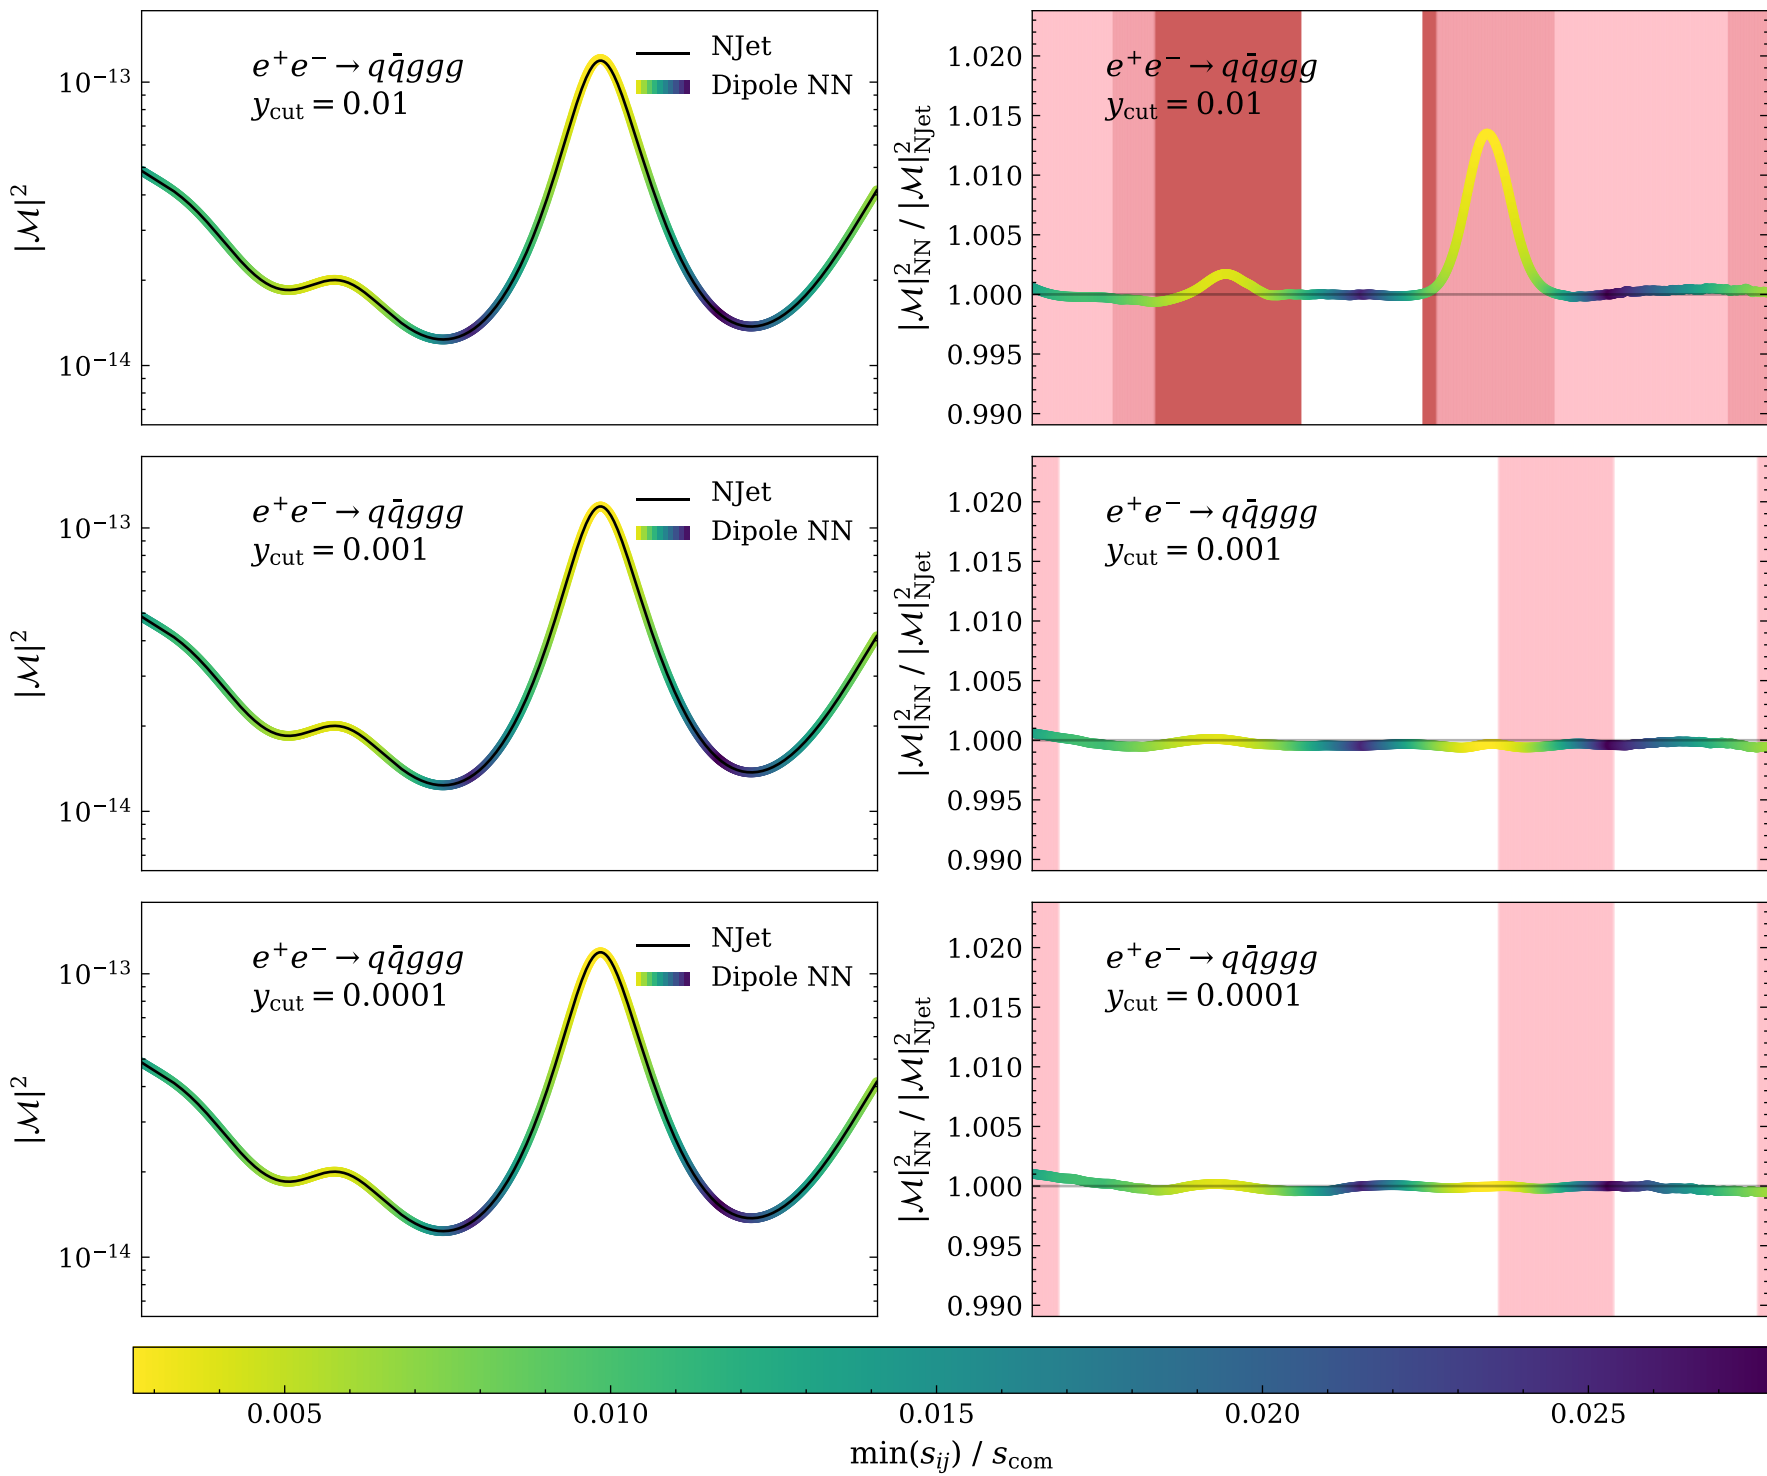

Trajectory 1265

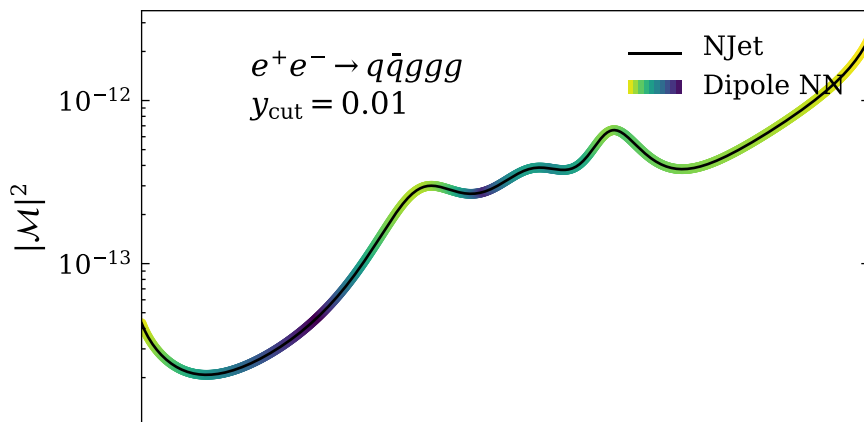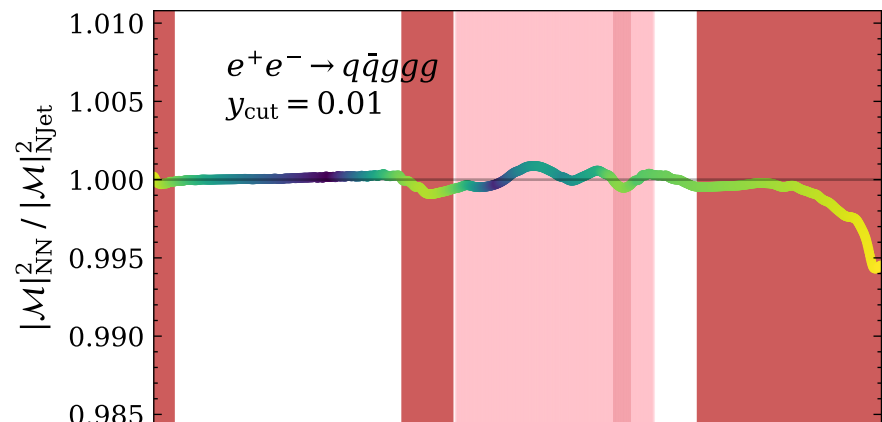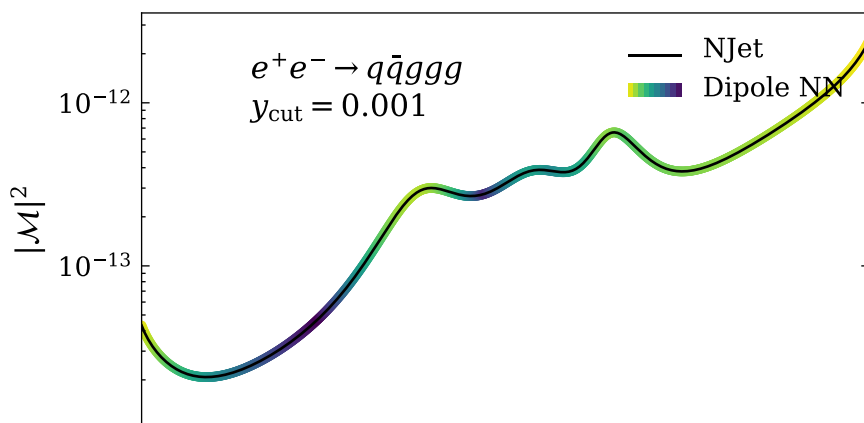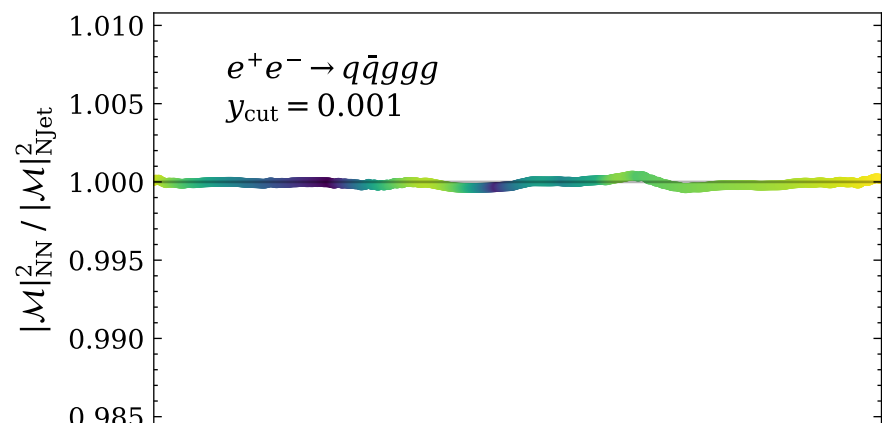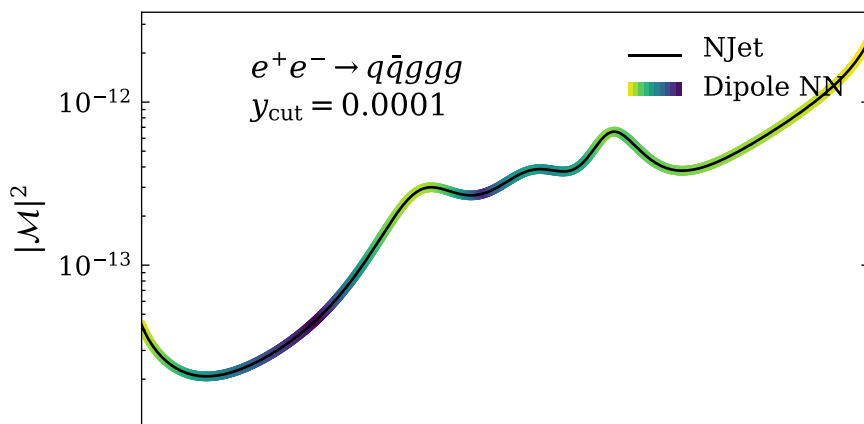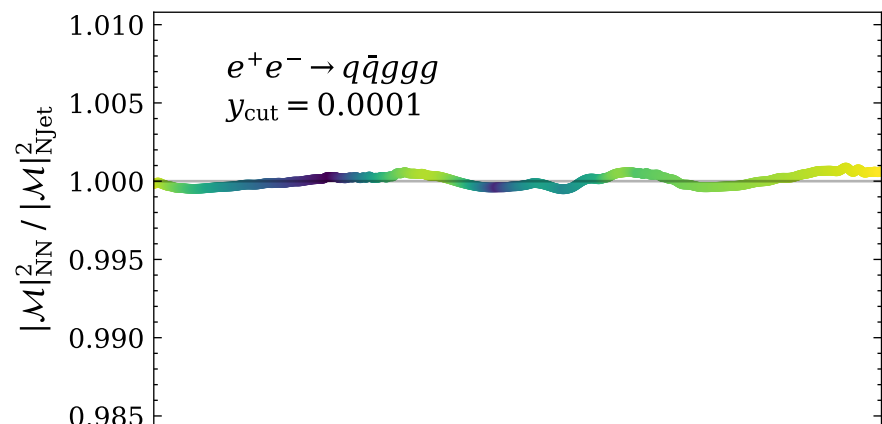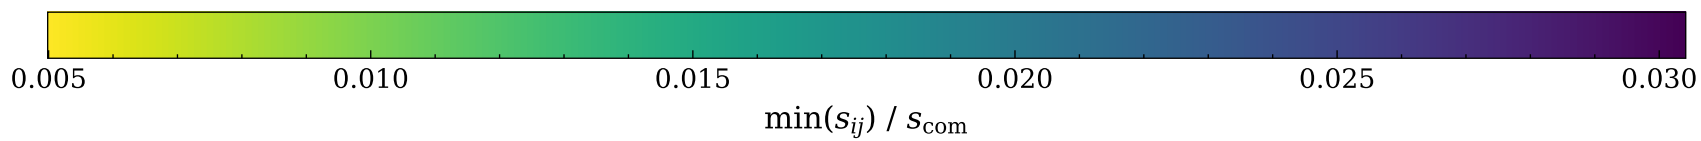

Trajectory 1266

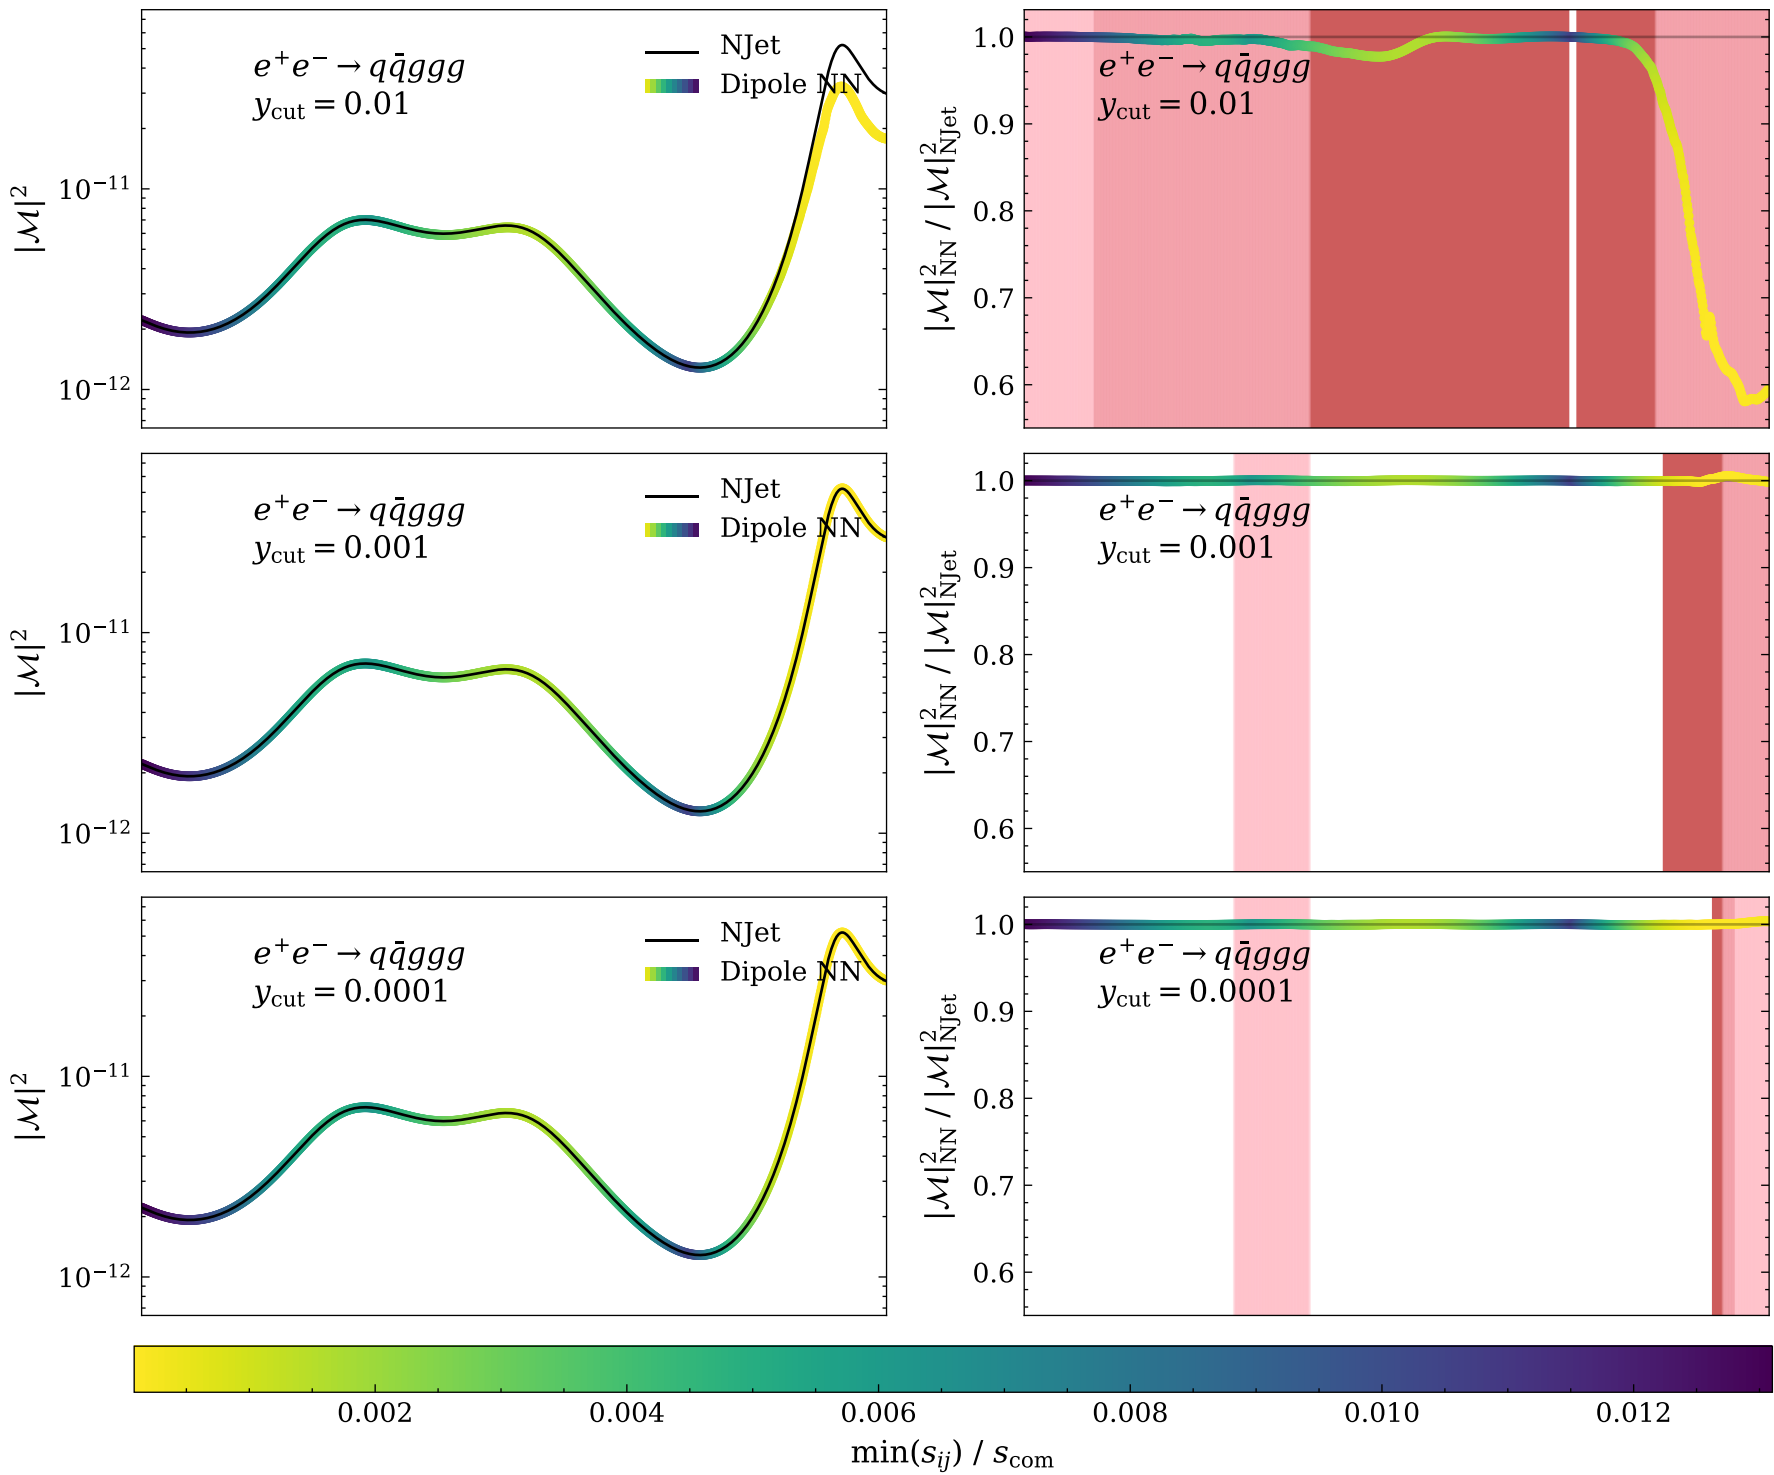

Trajectory 1267

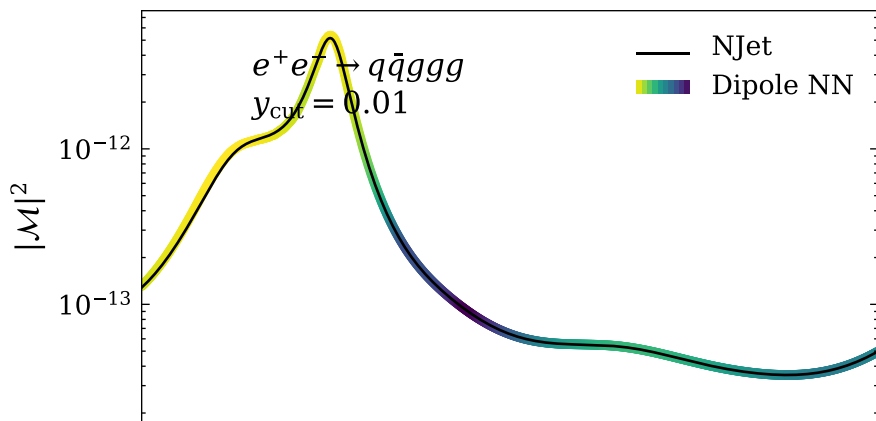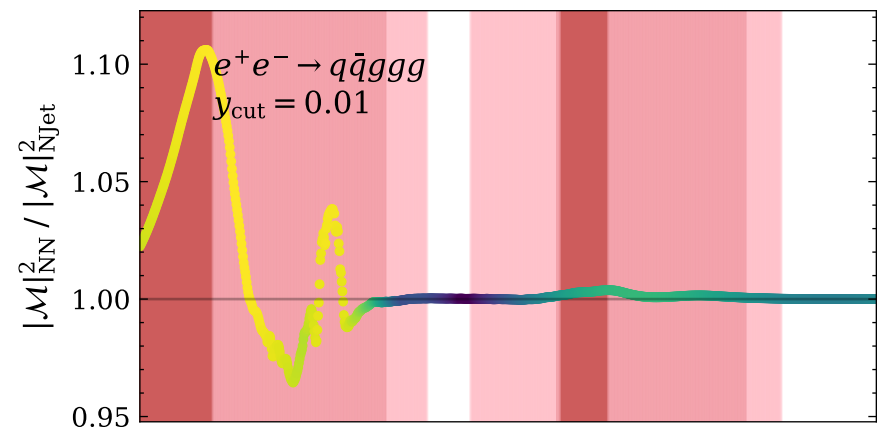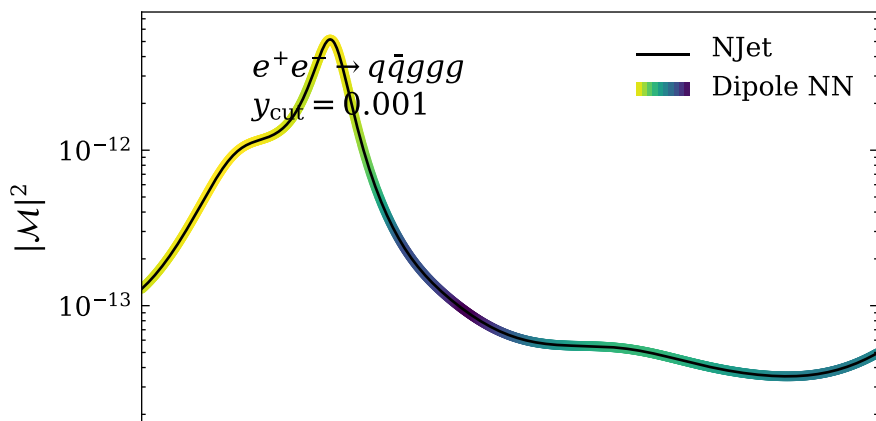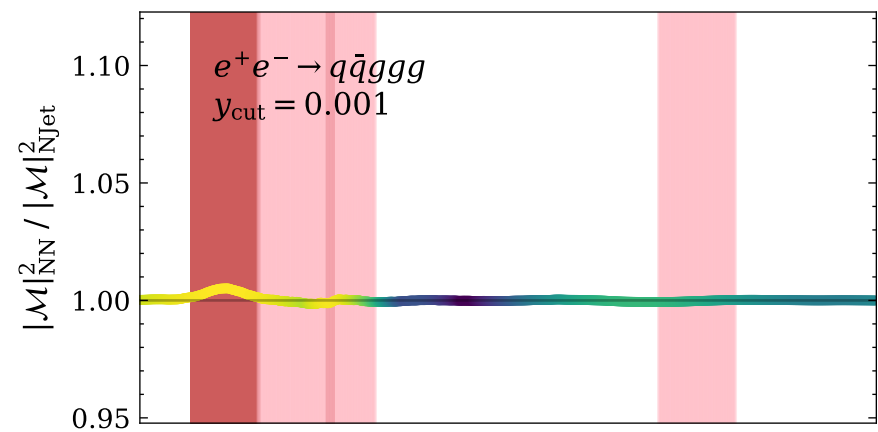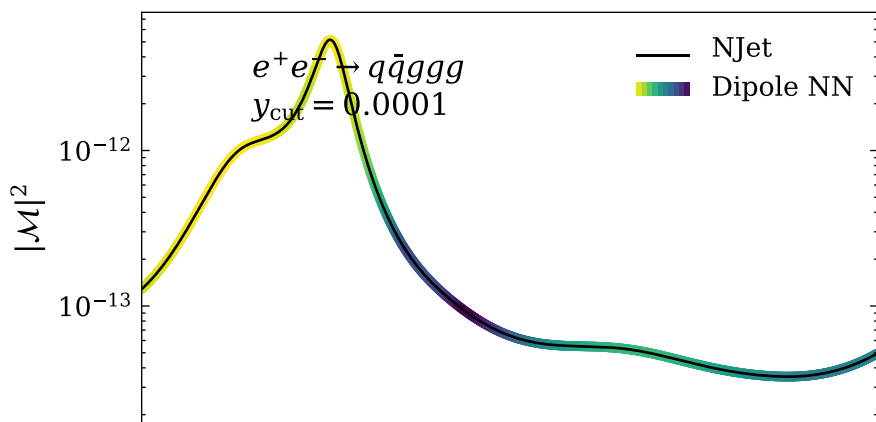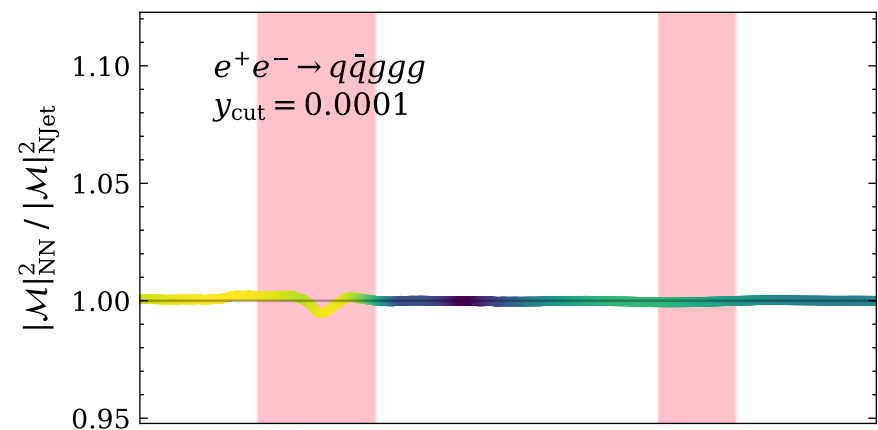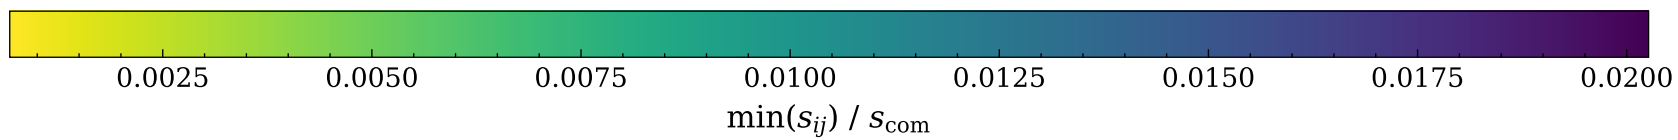

Trajectory 1268

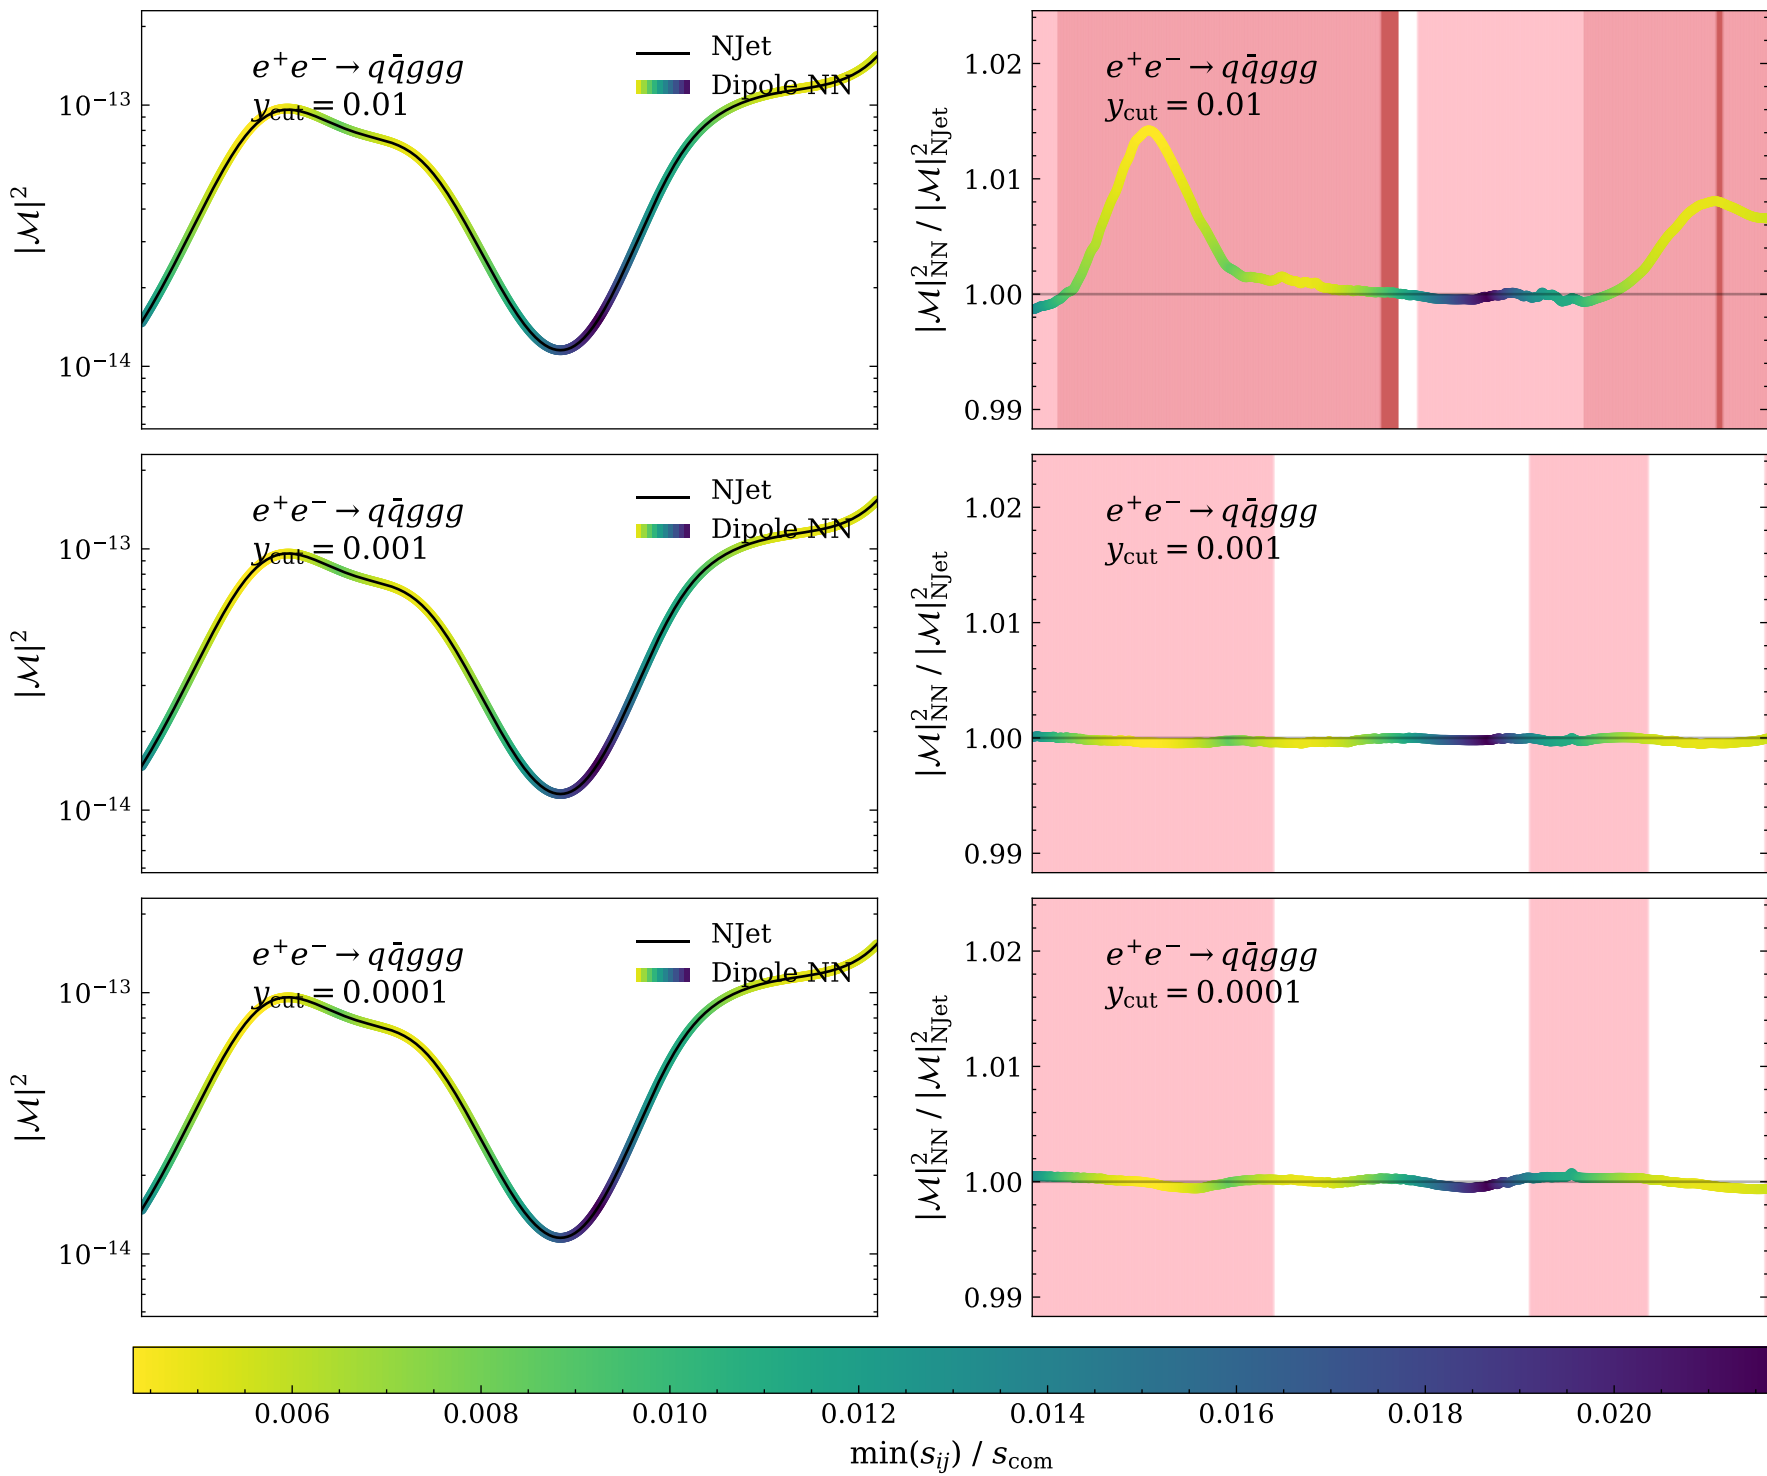

Trajectory 1269

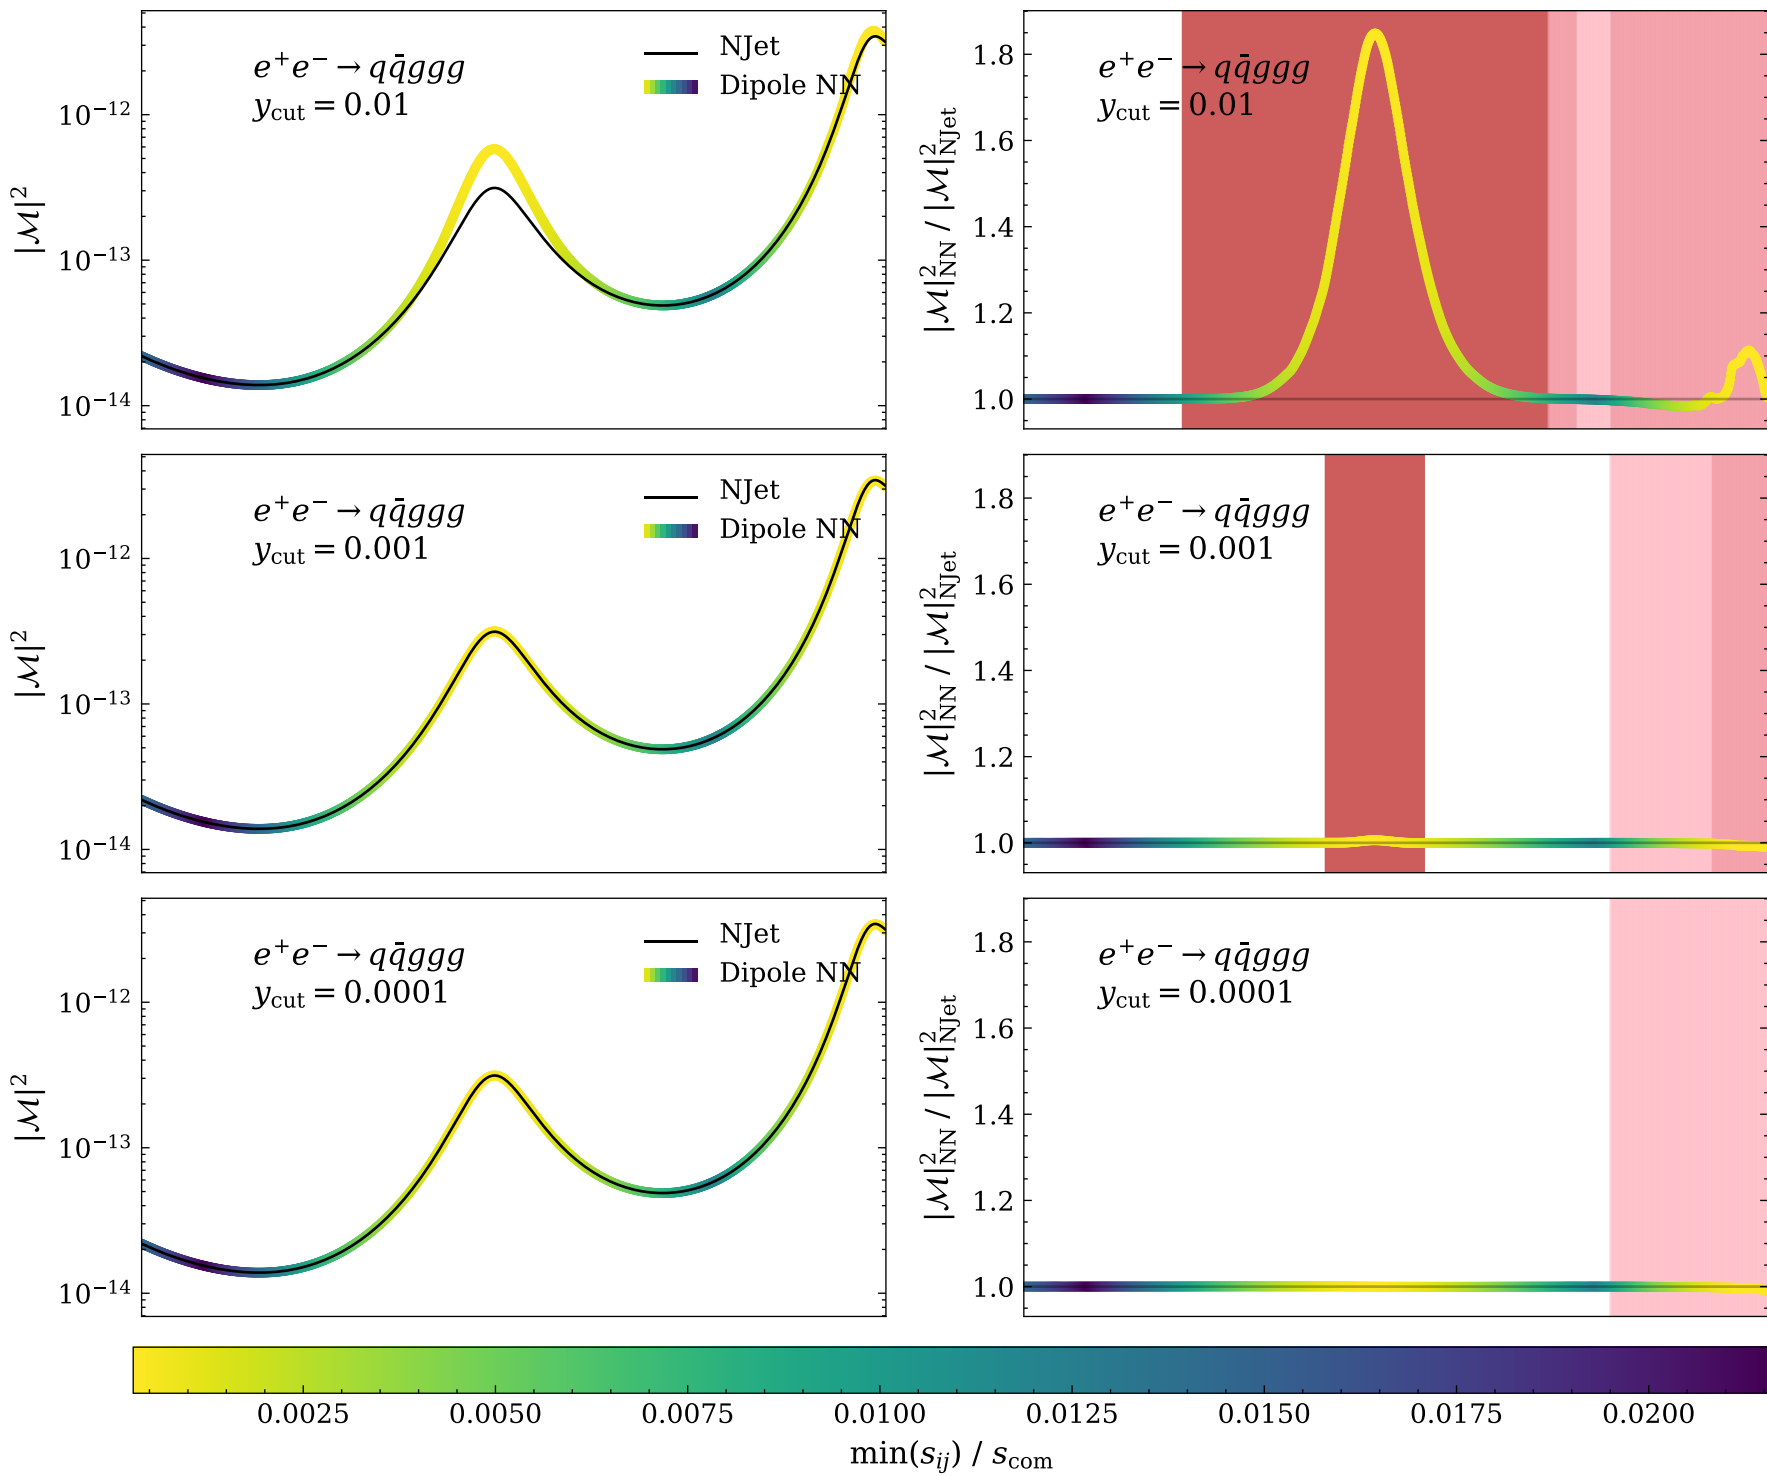

Trajectory 1270

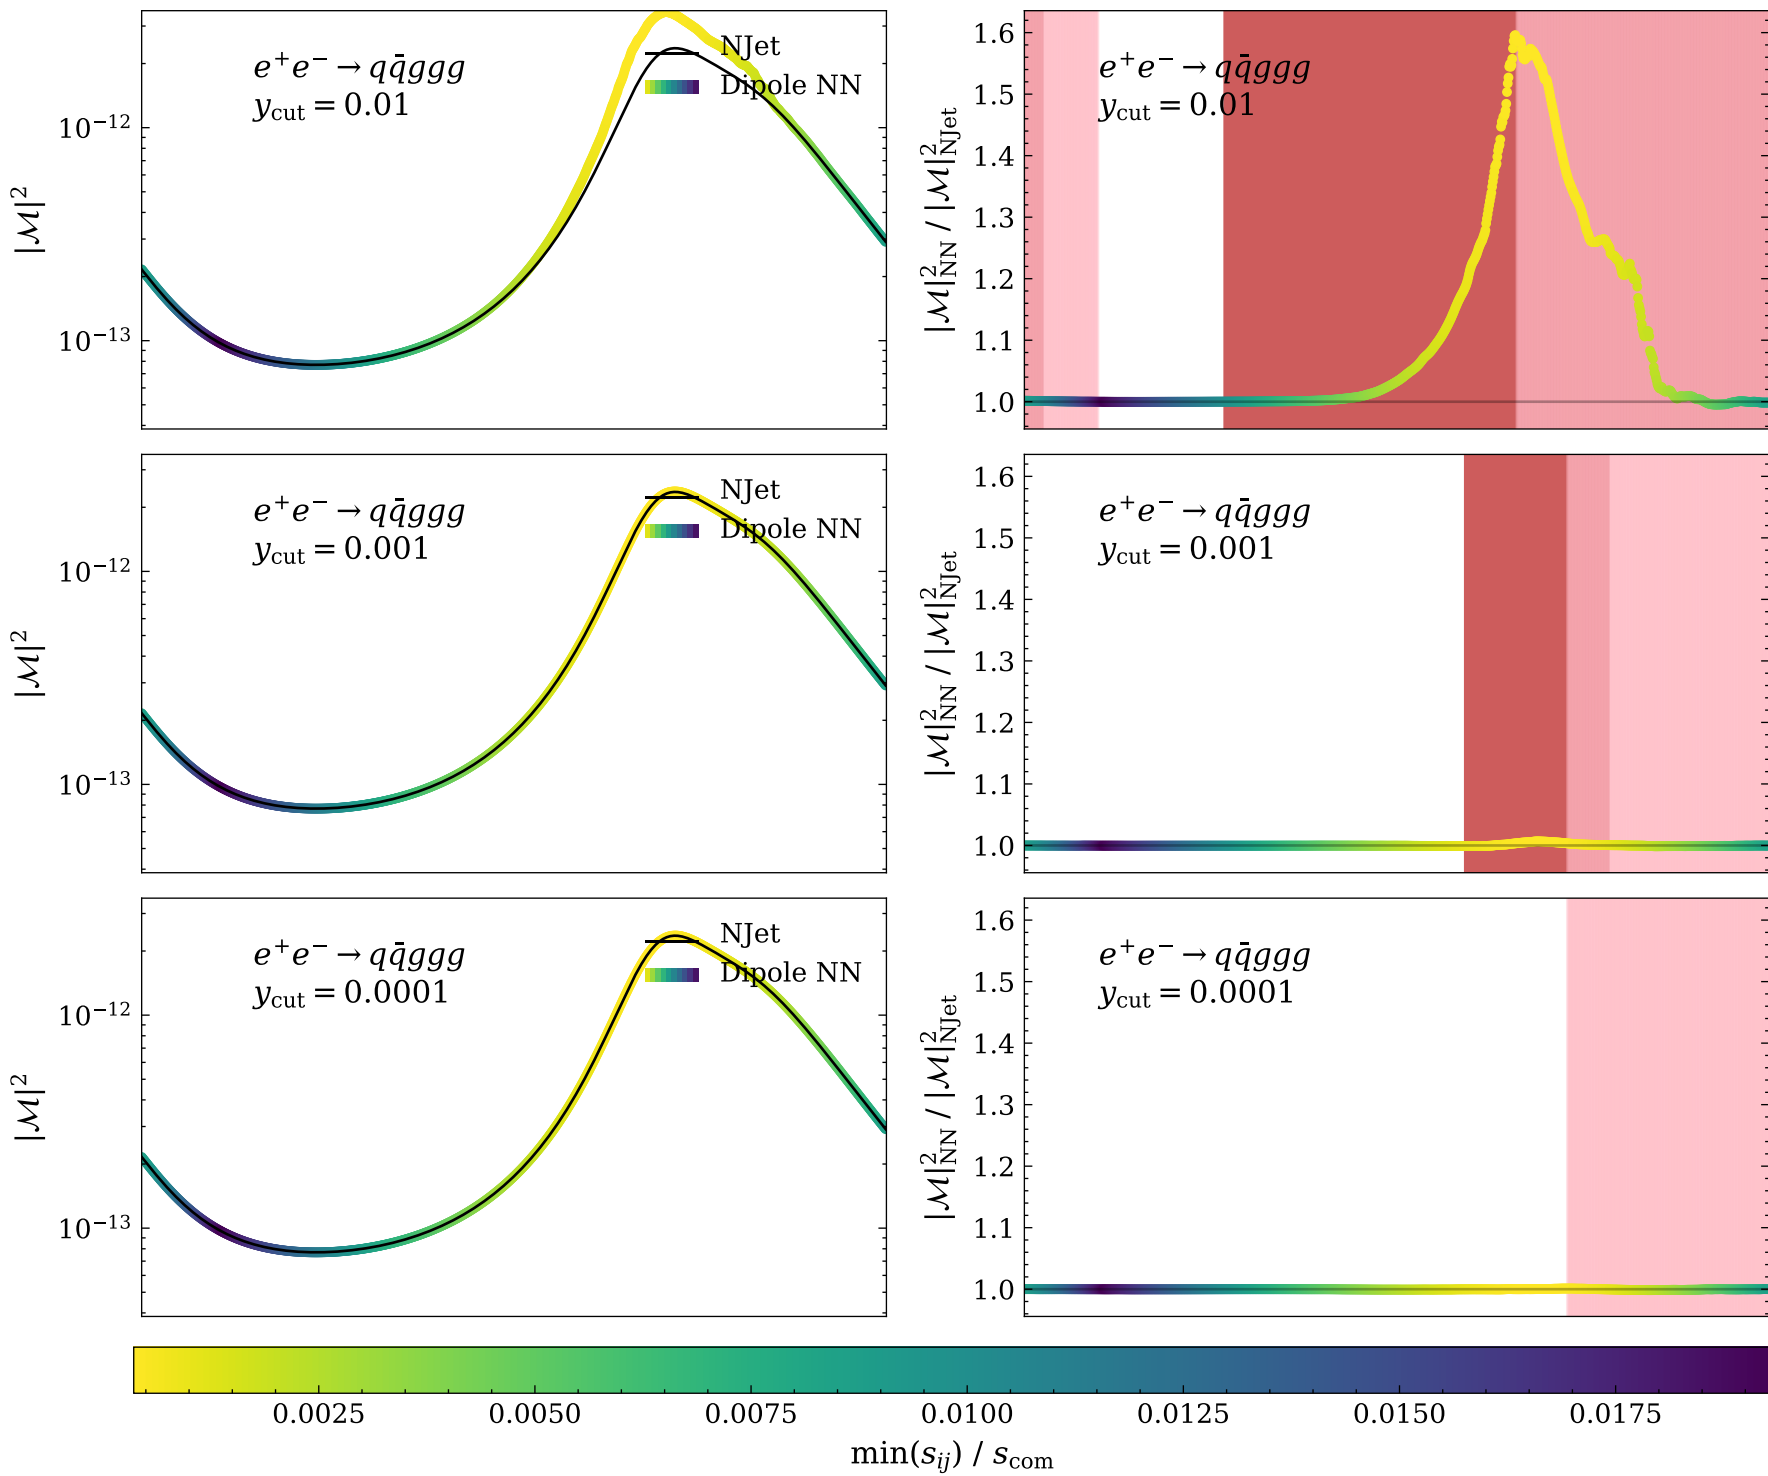

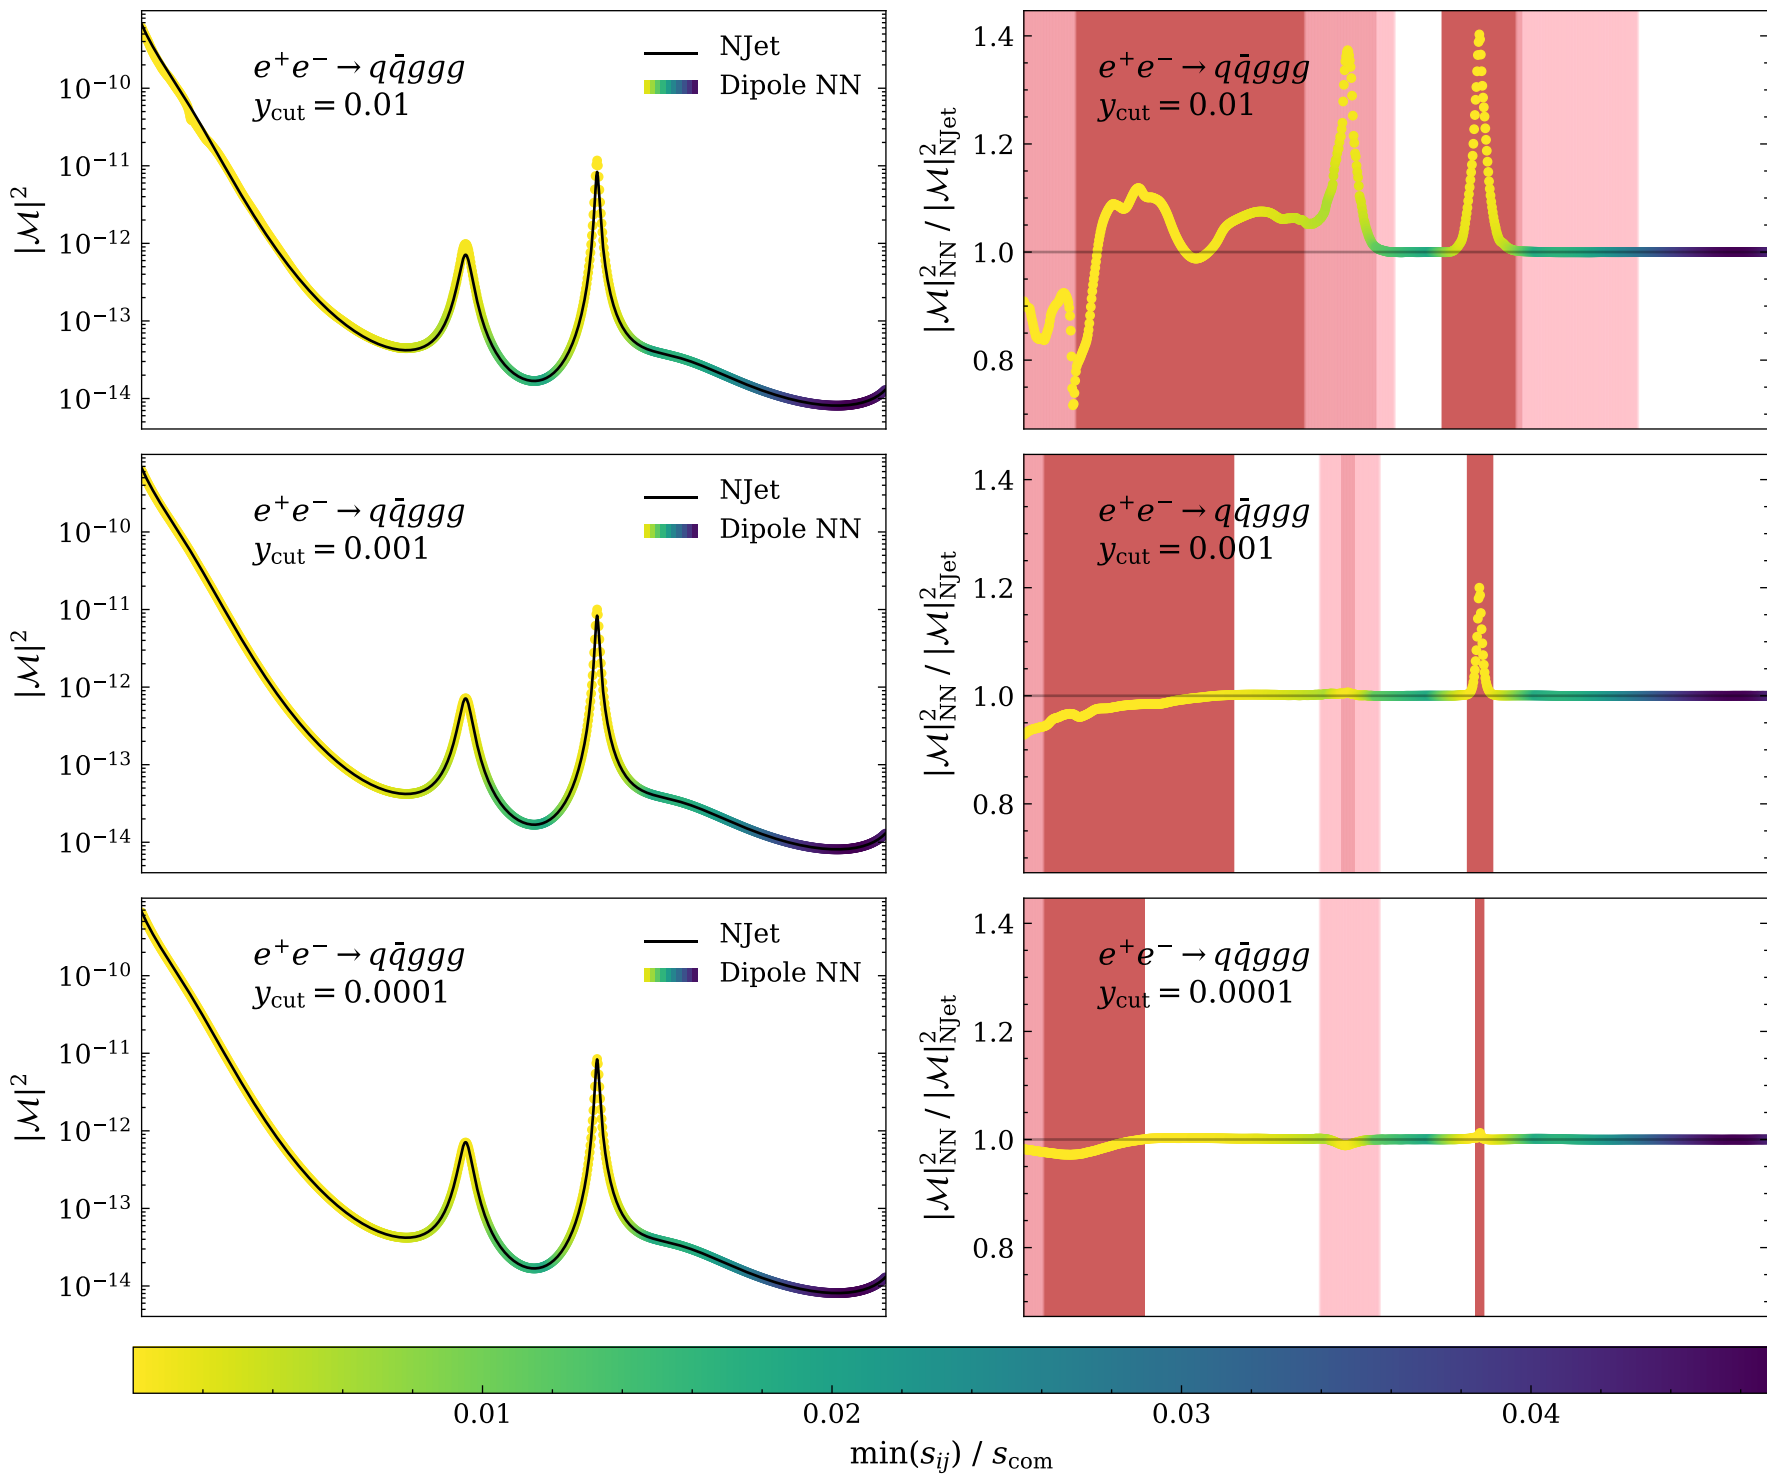

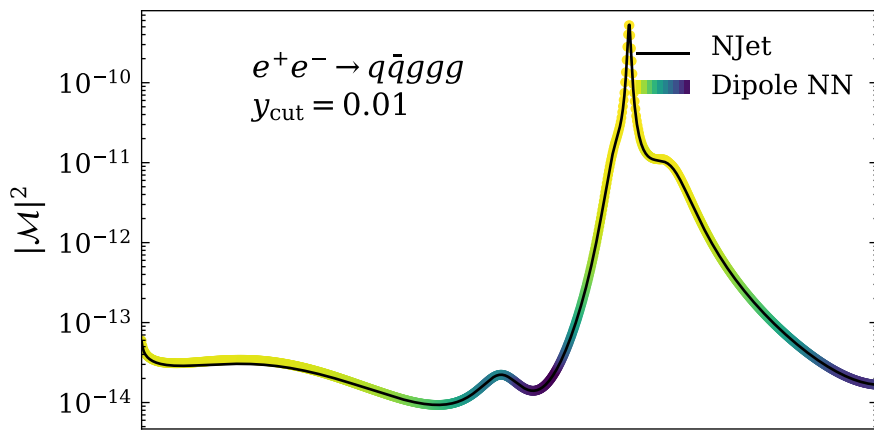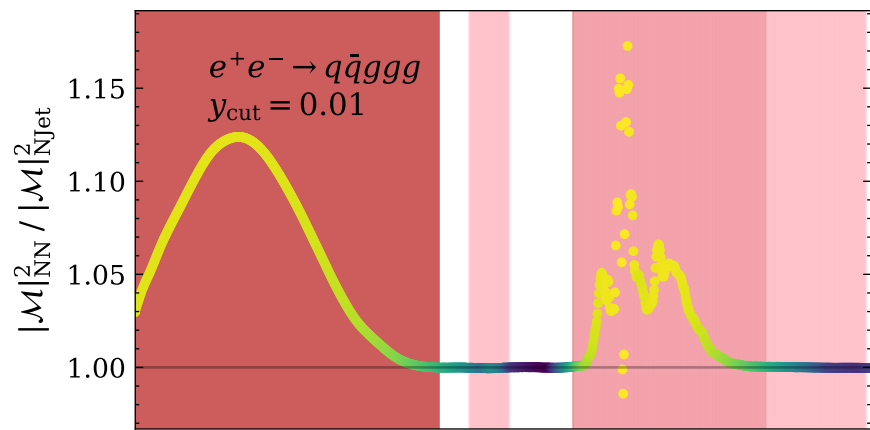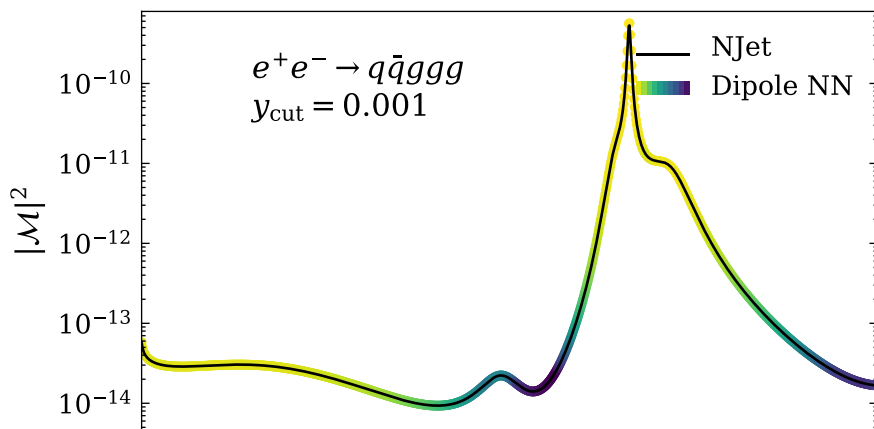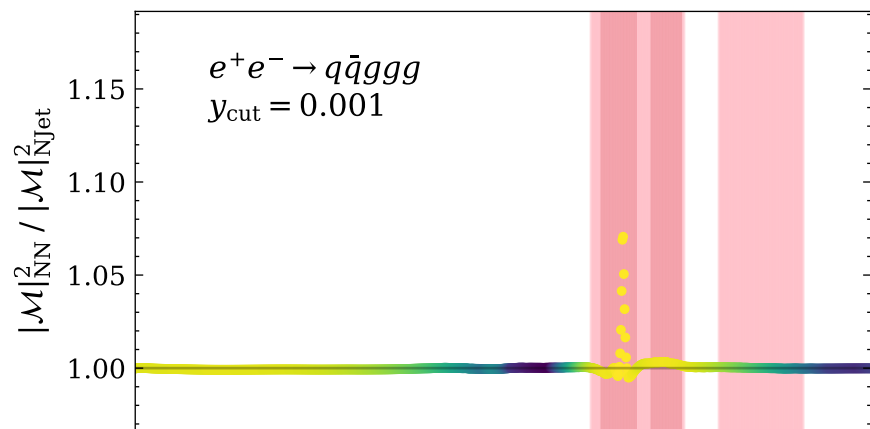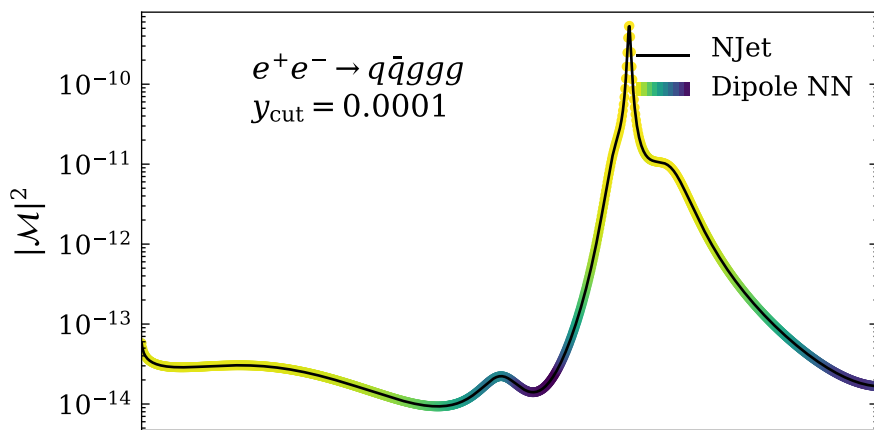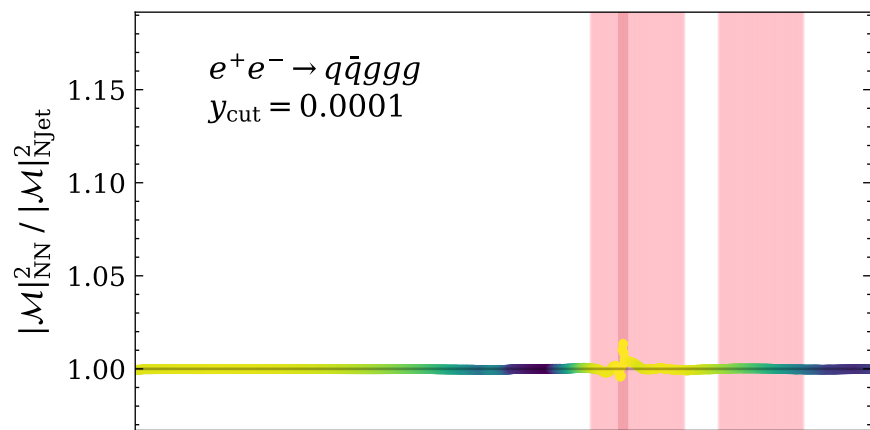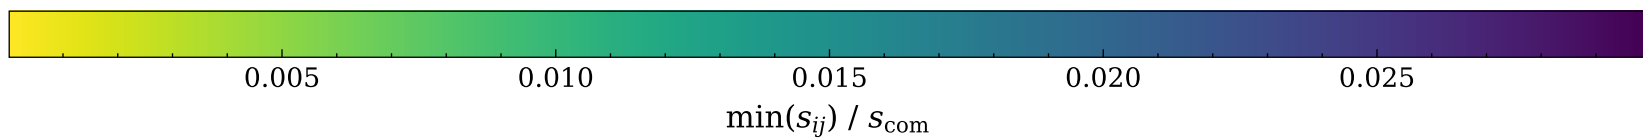

Trajectory 1273

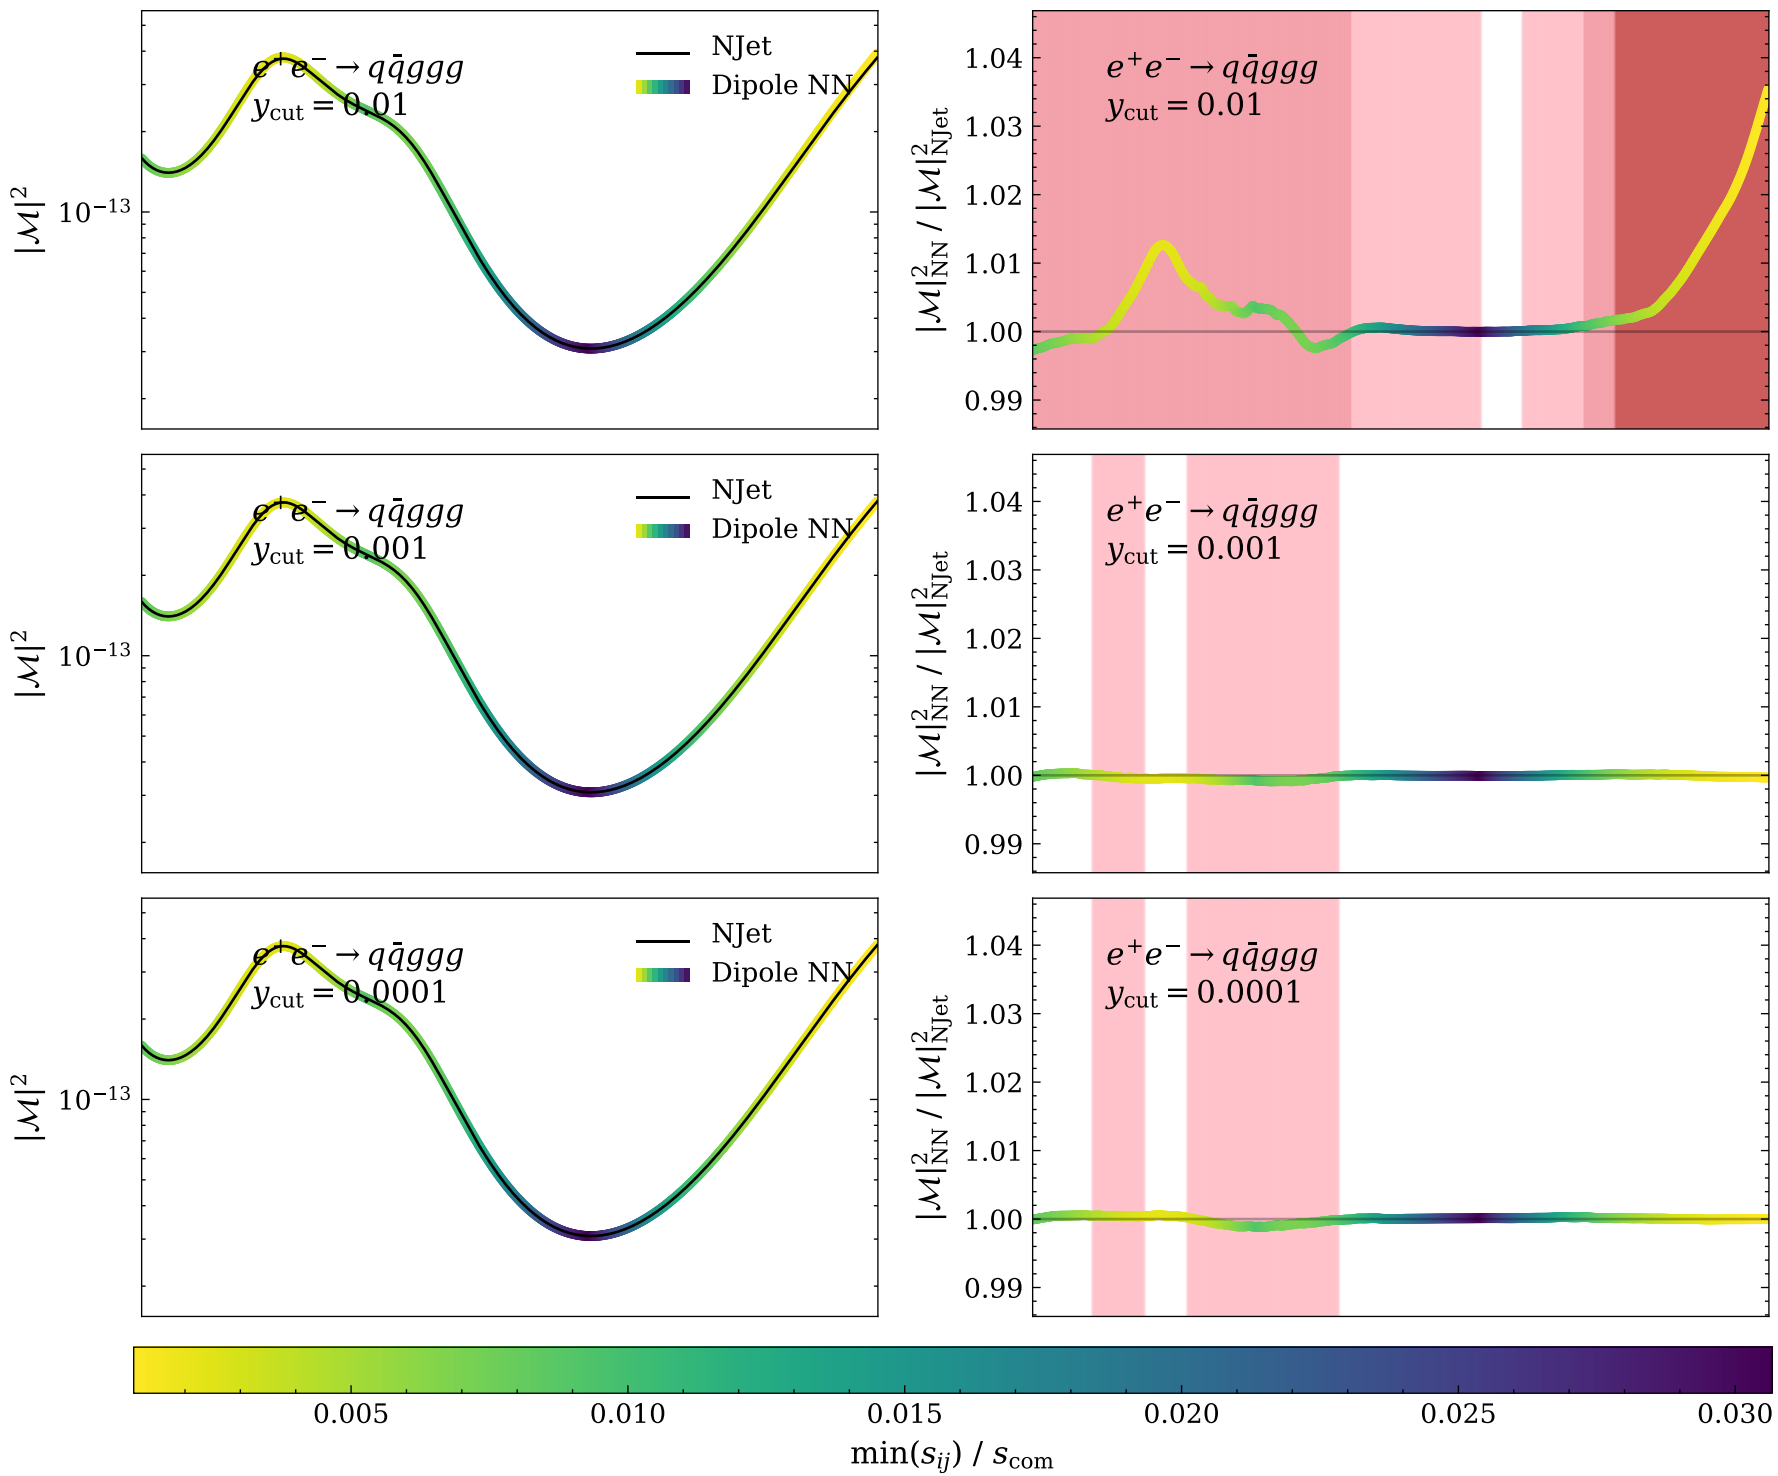

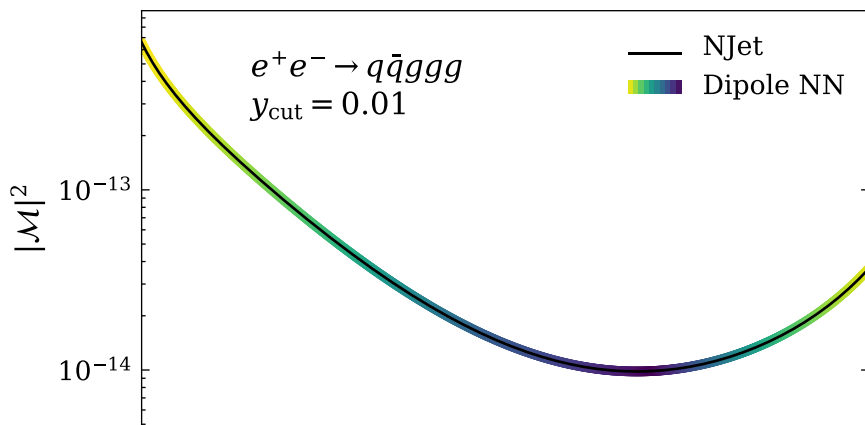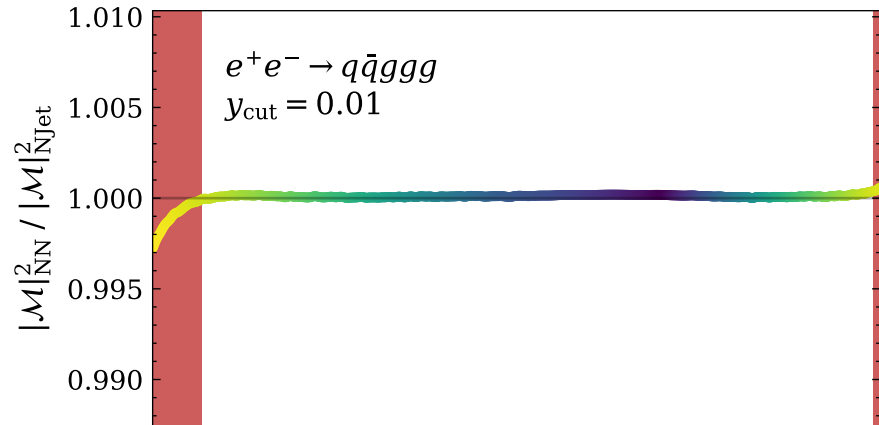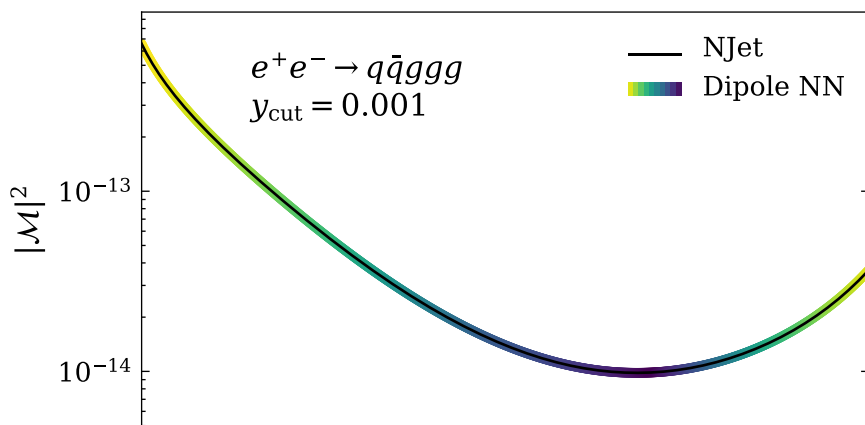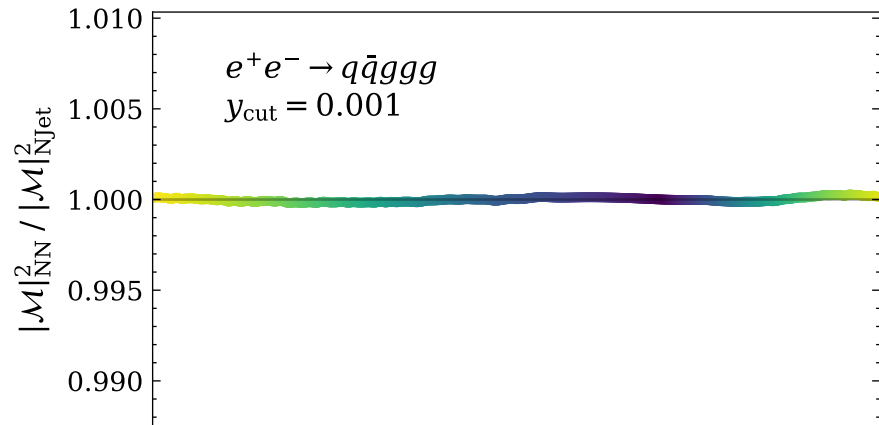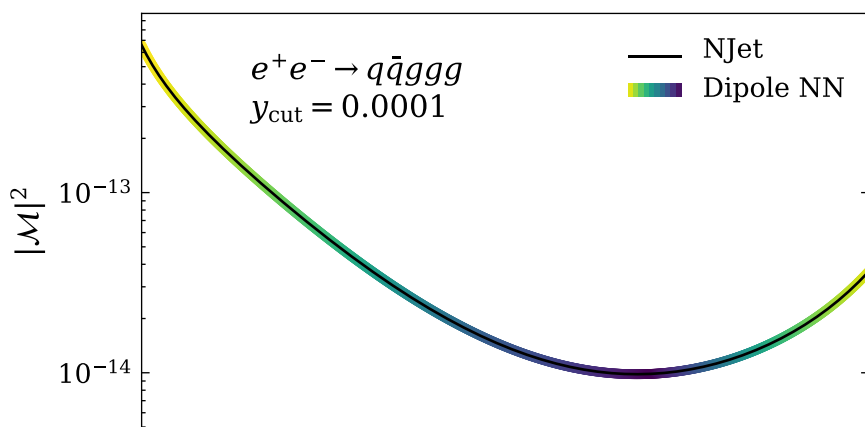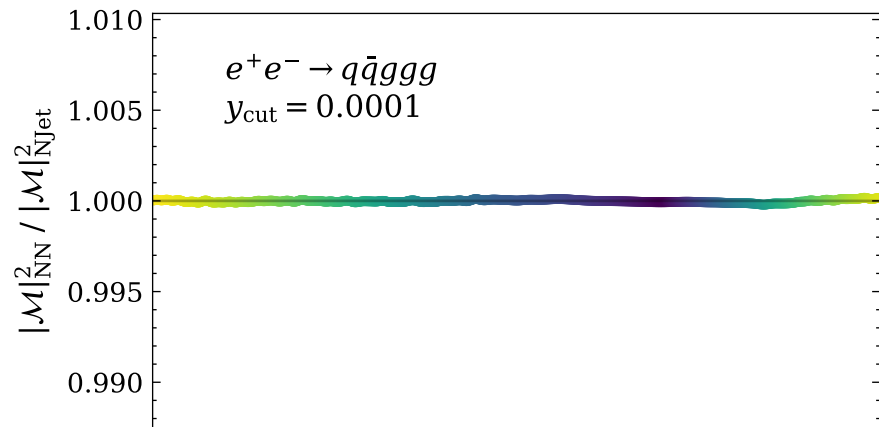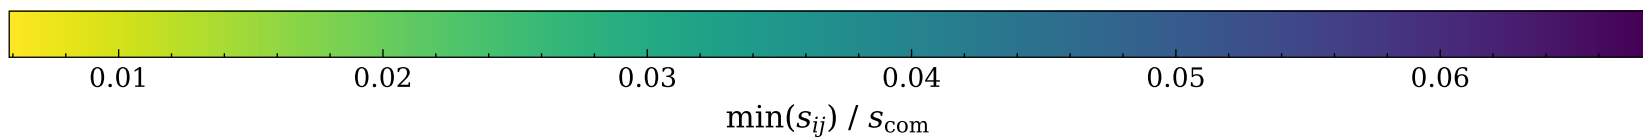

Trajectory 1275

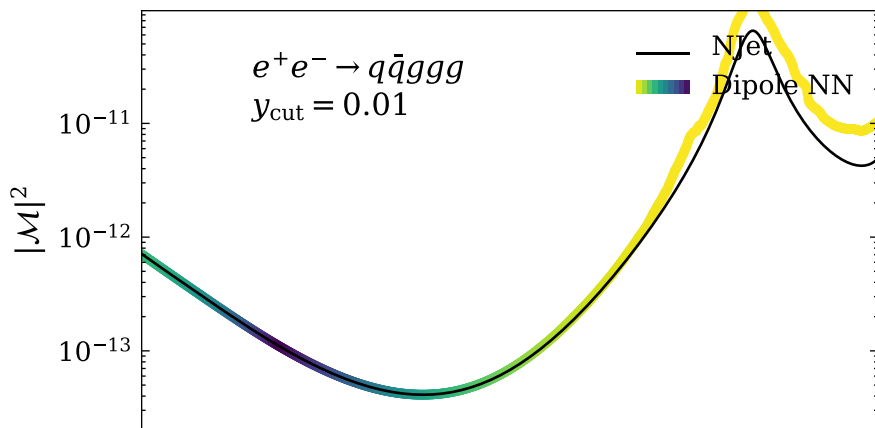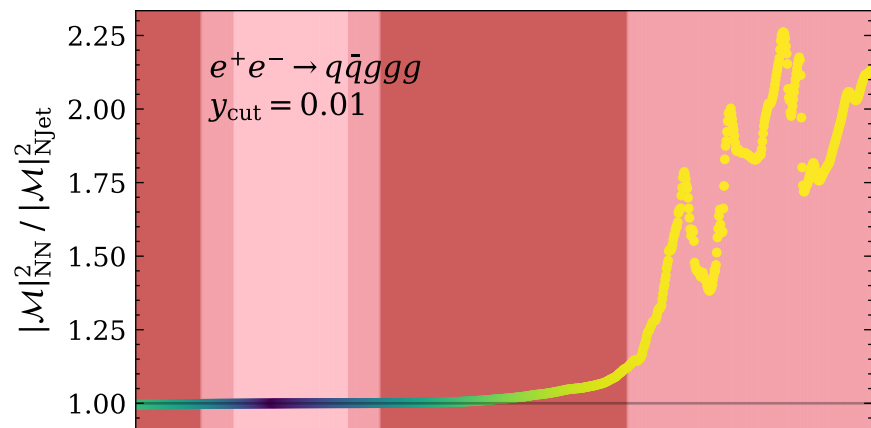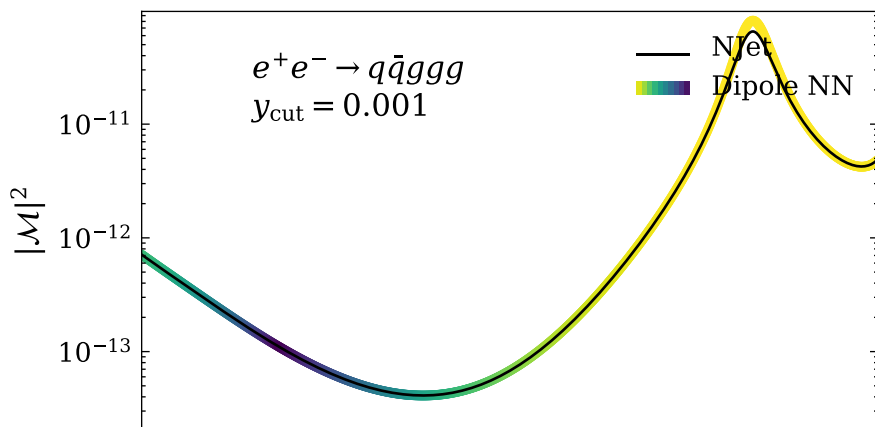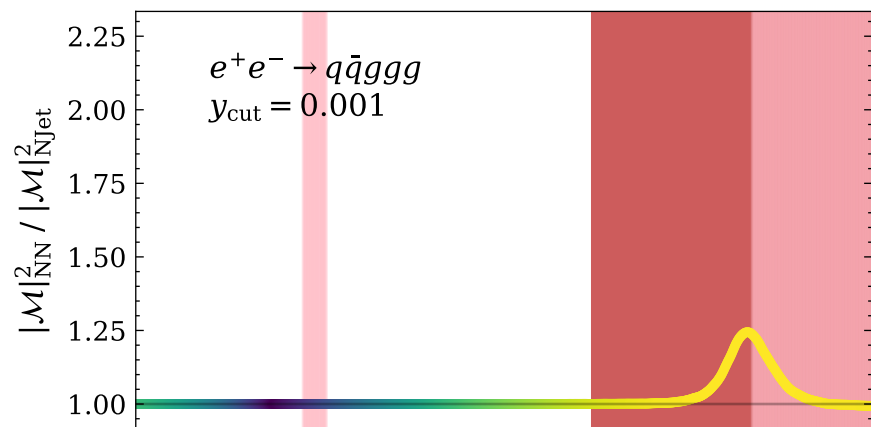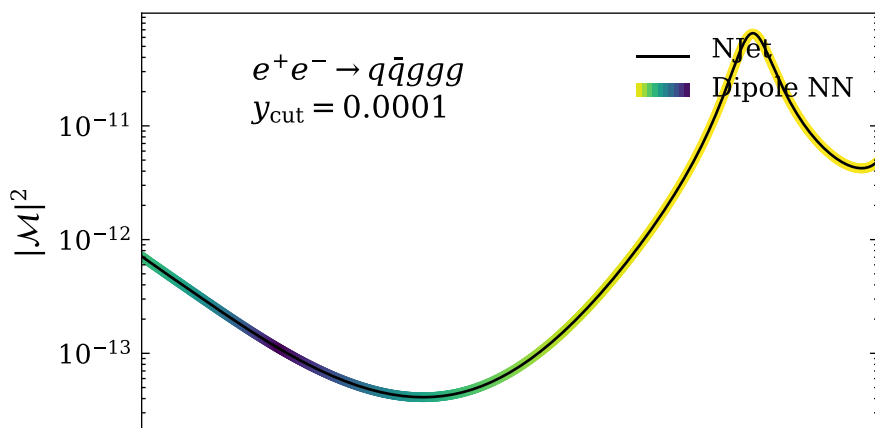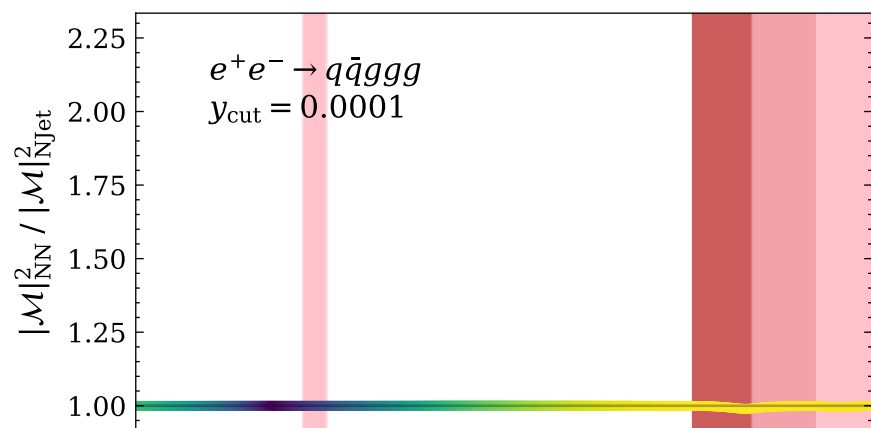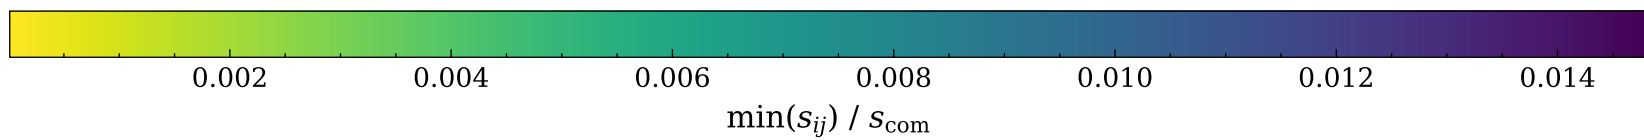

Trajectory 1276

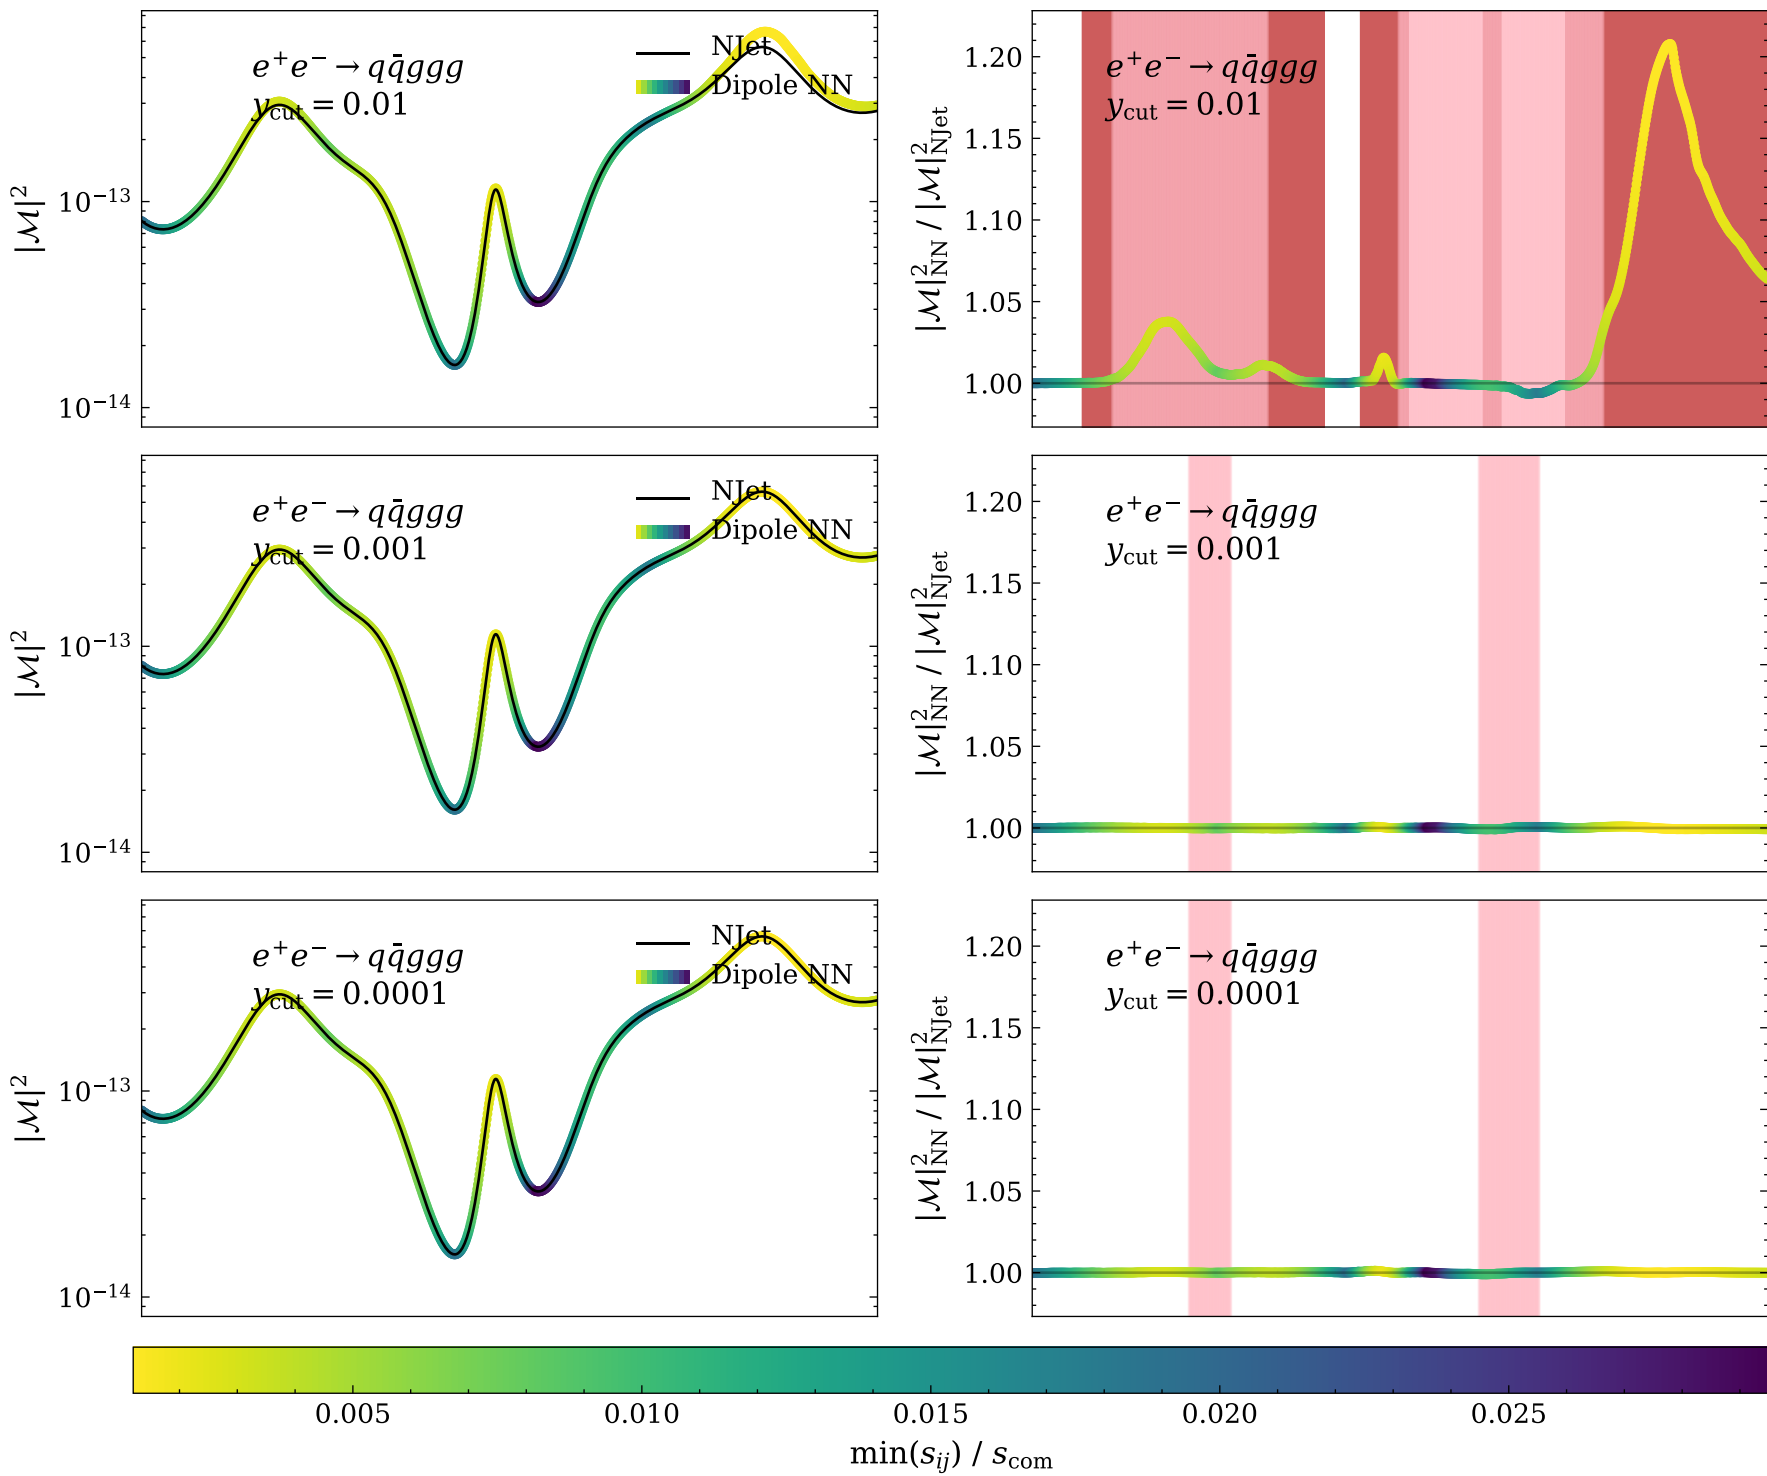

Trajectory 1277

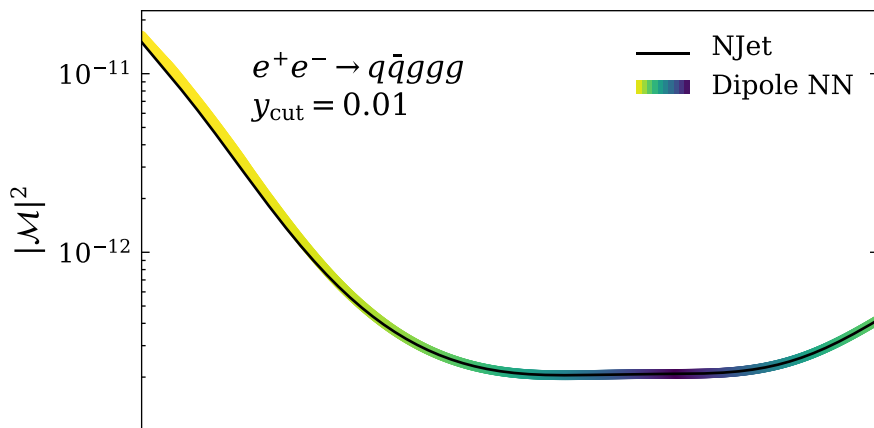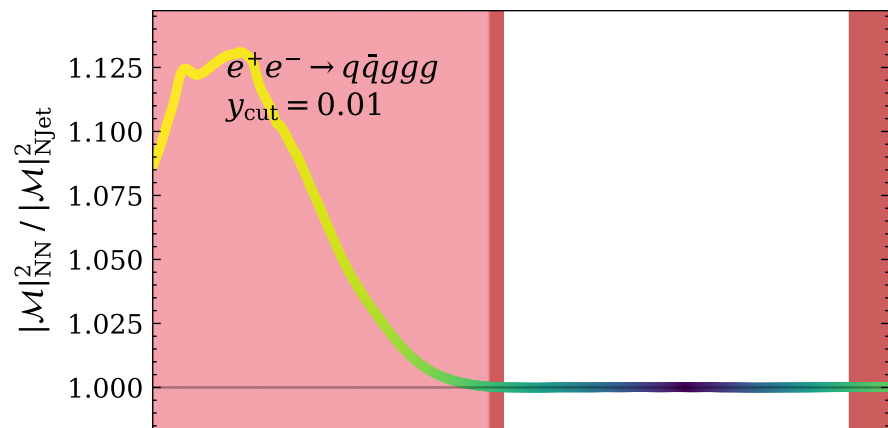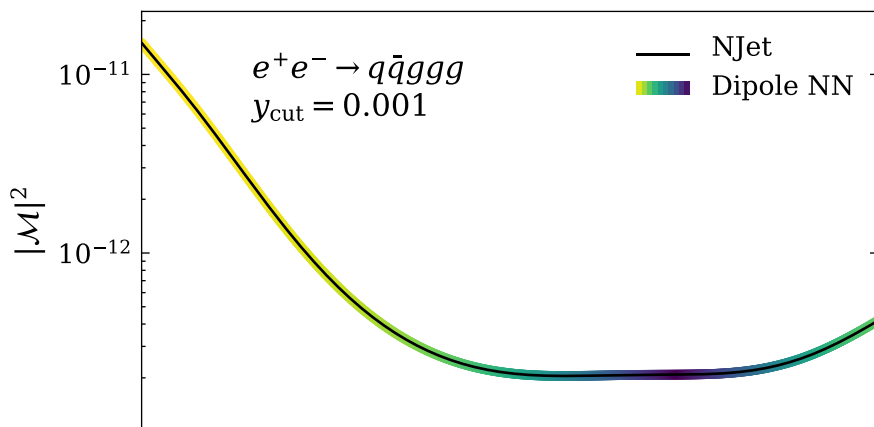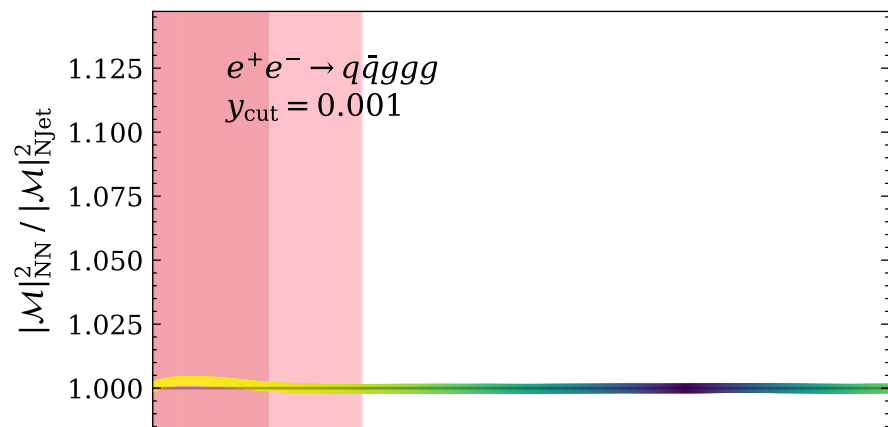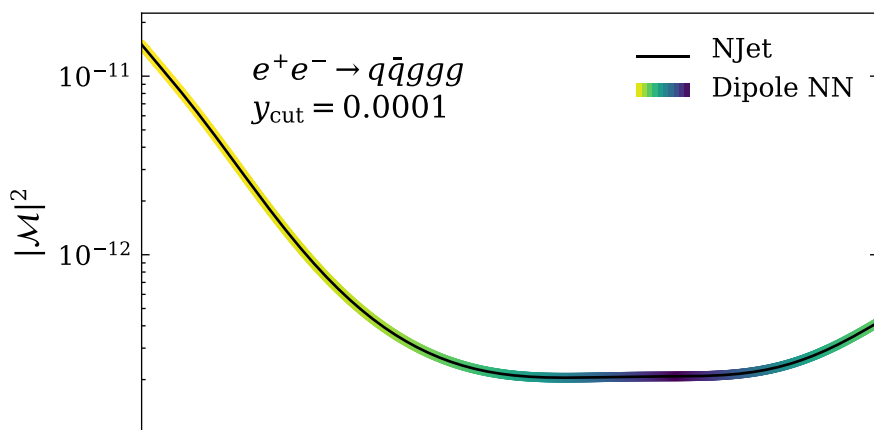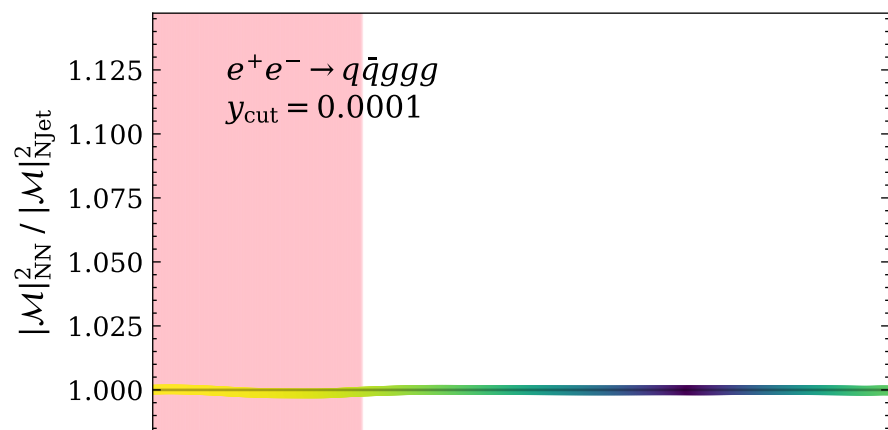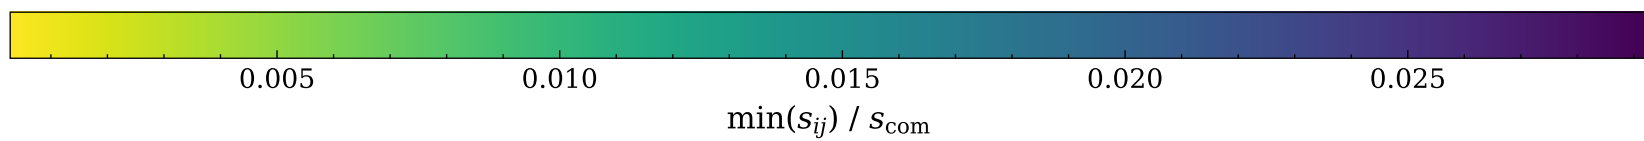

Trajectory 1278

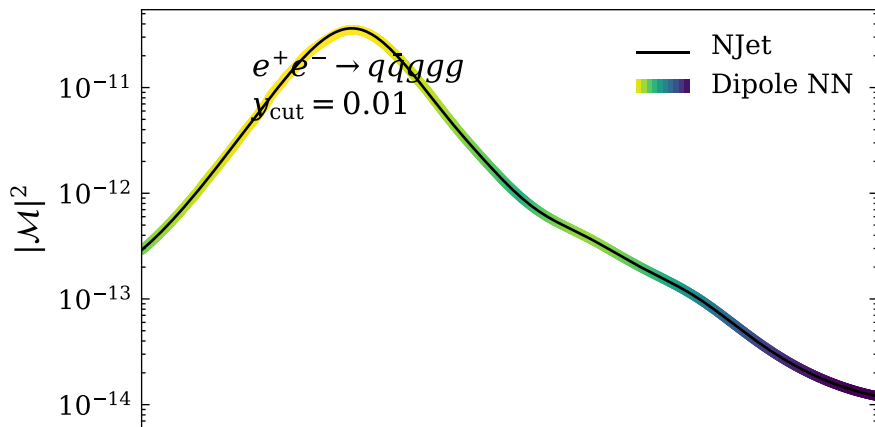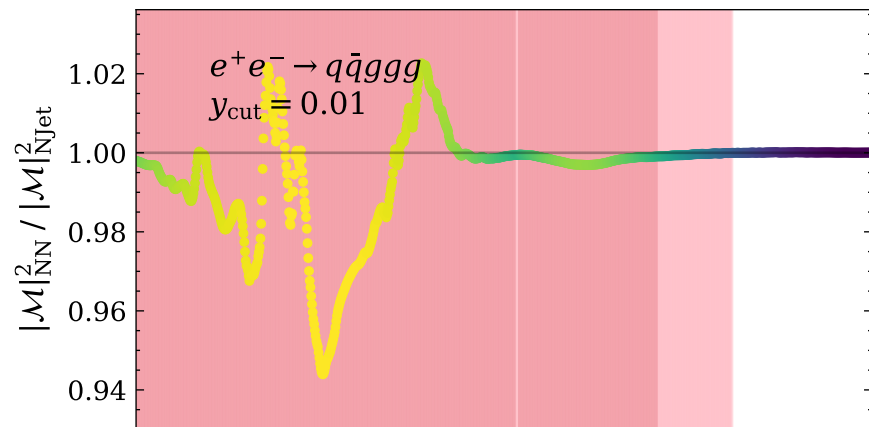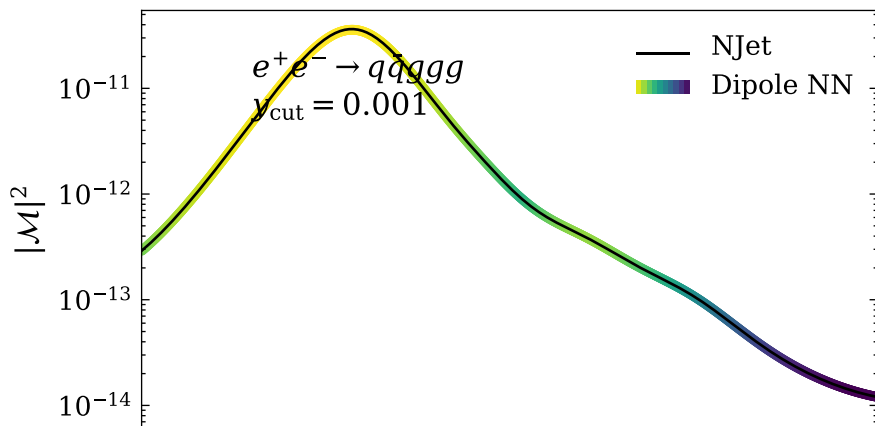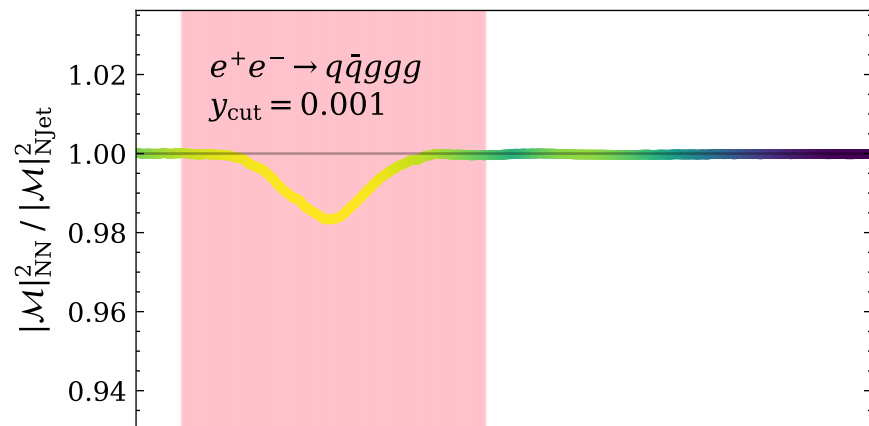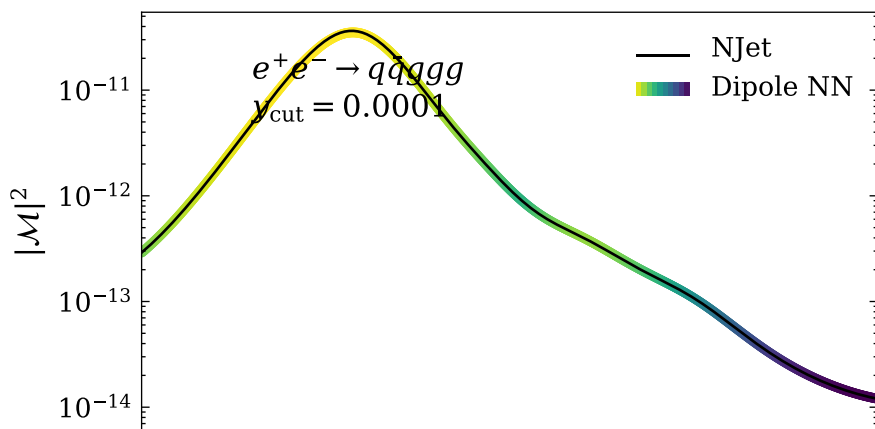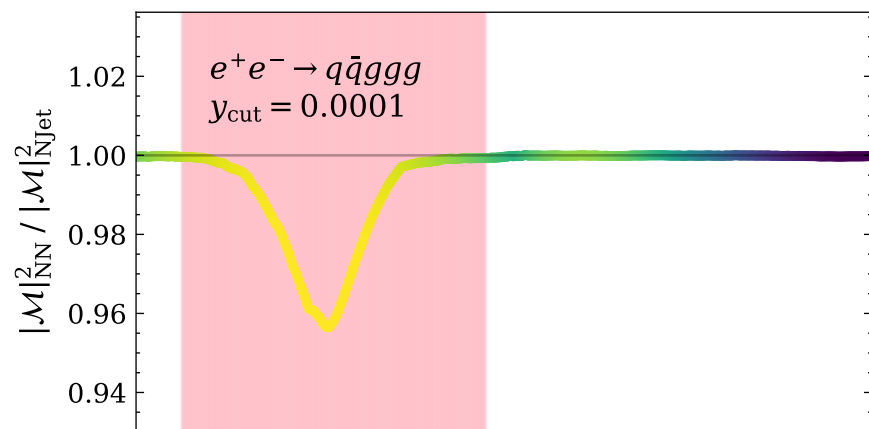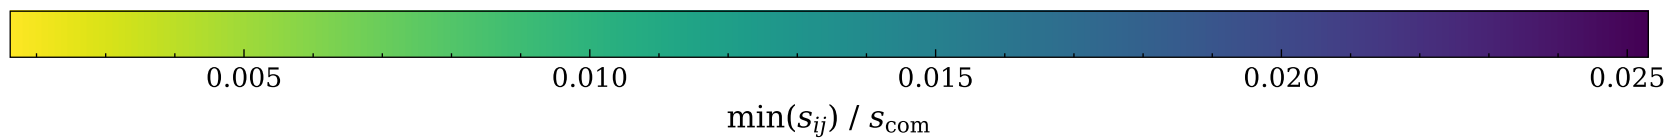

Trajectory 1279

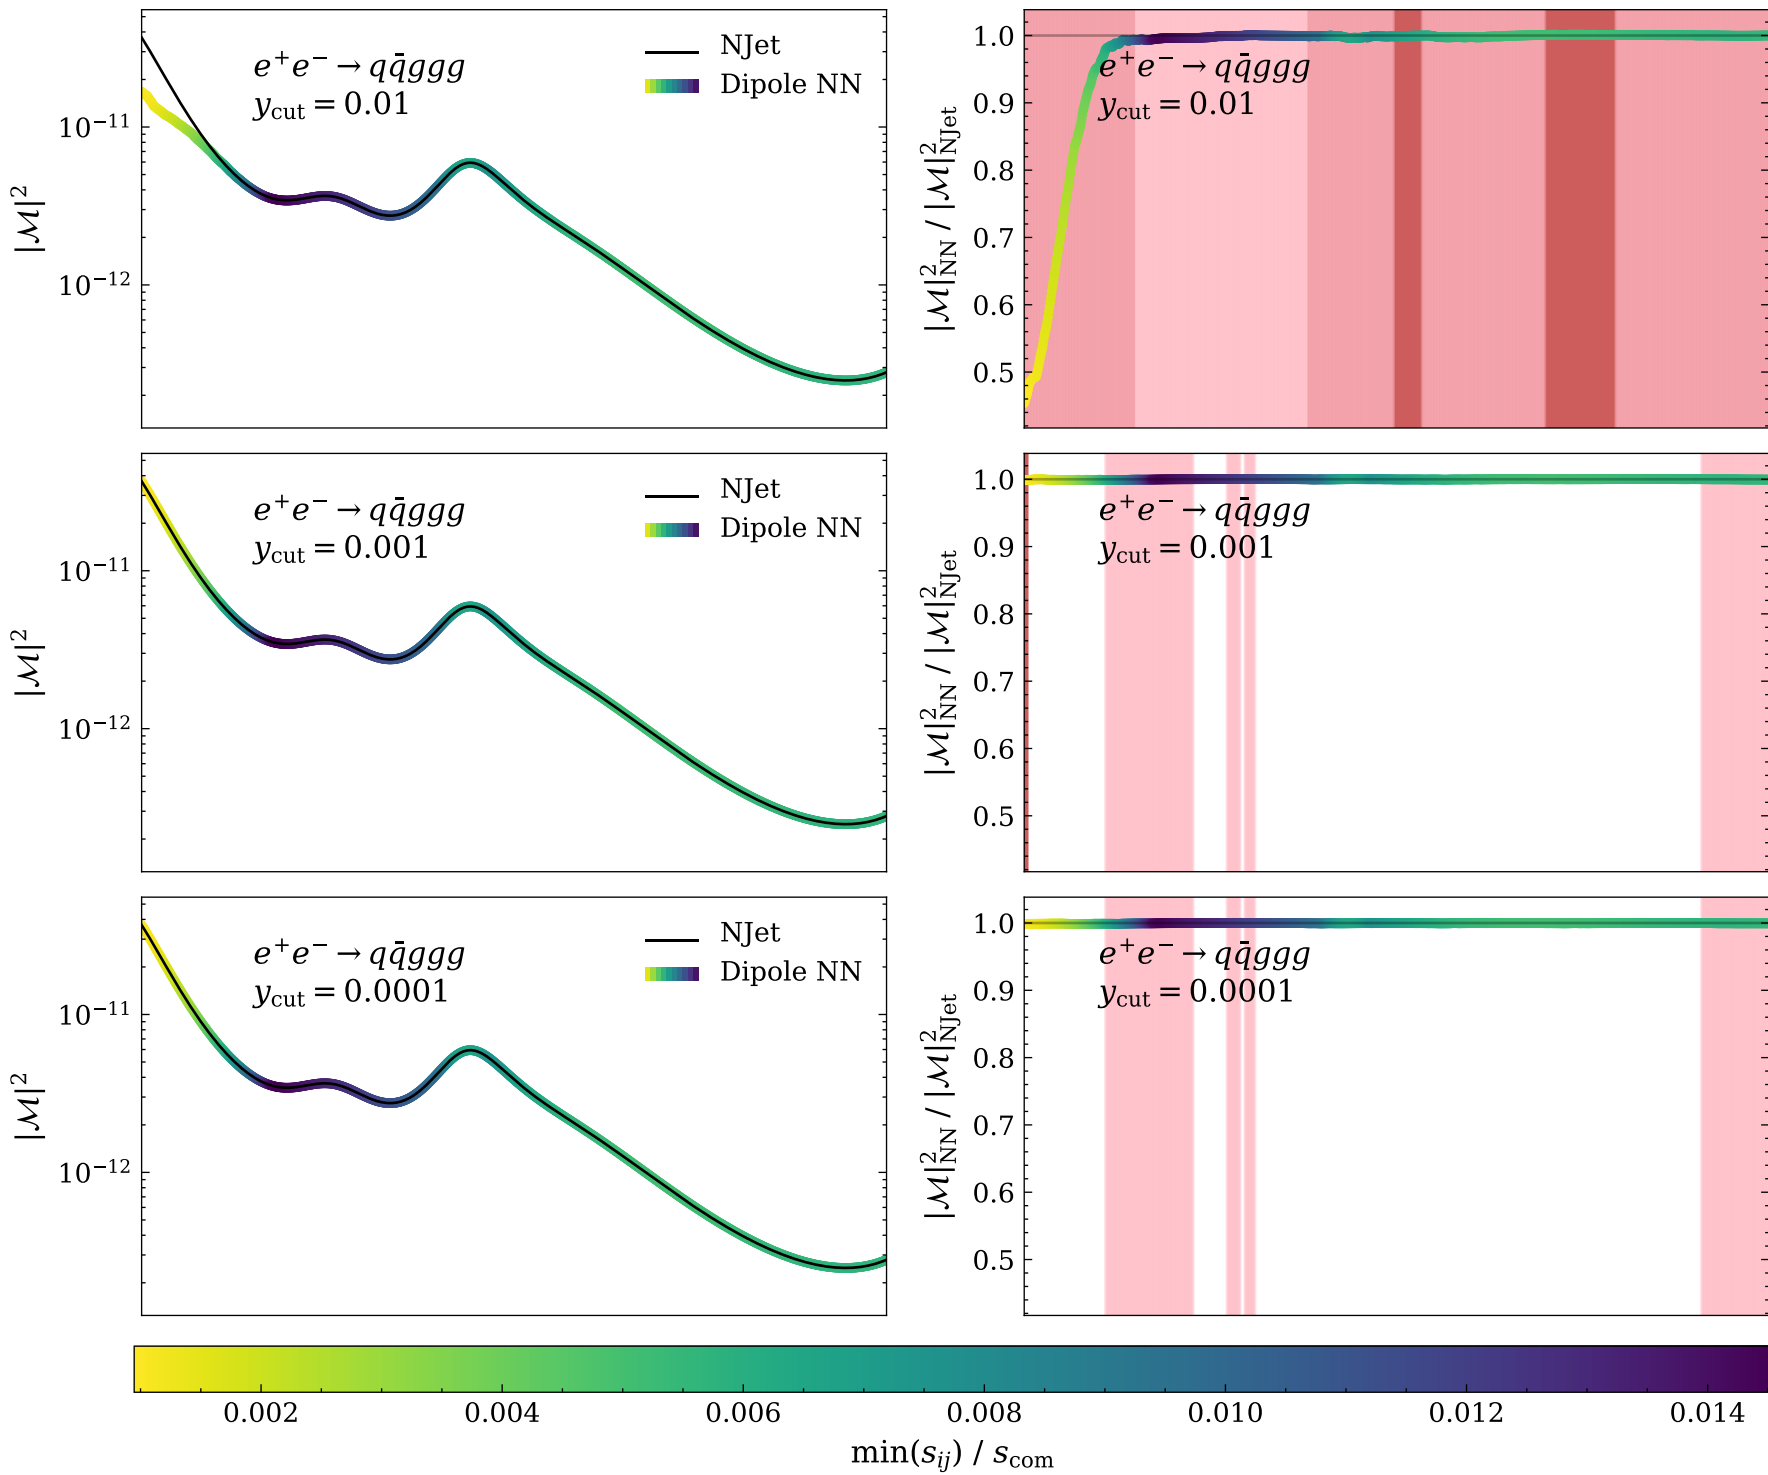

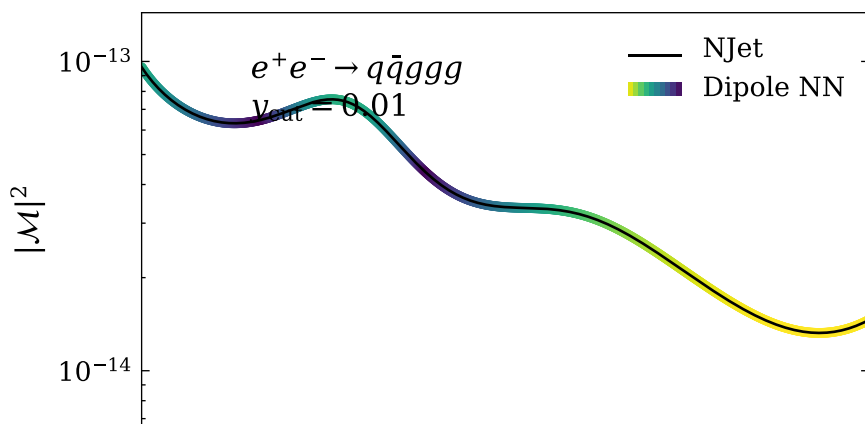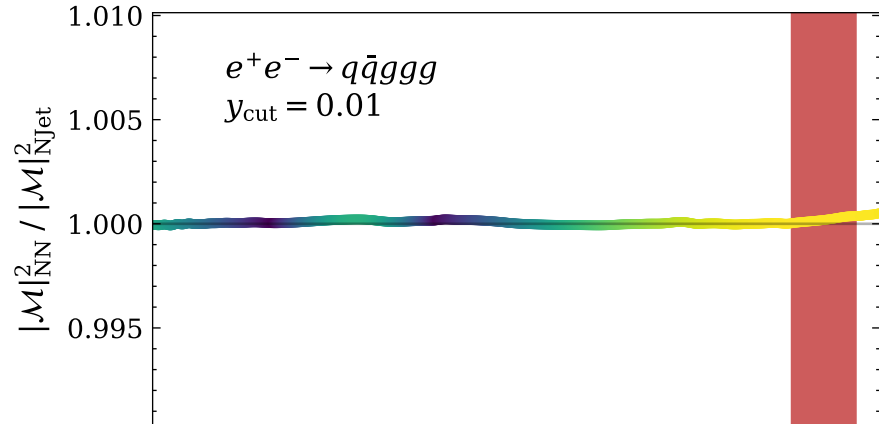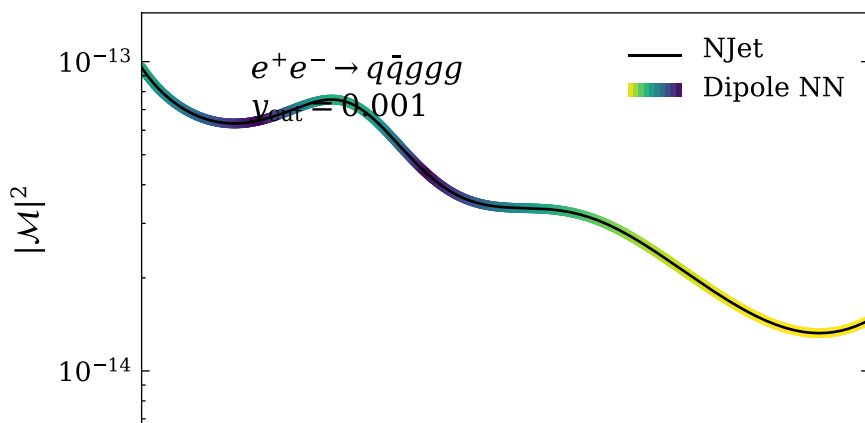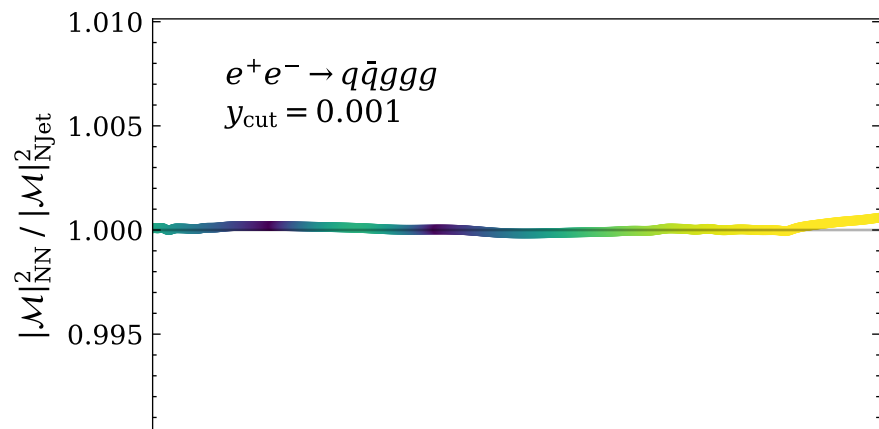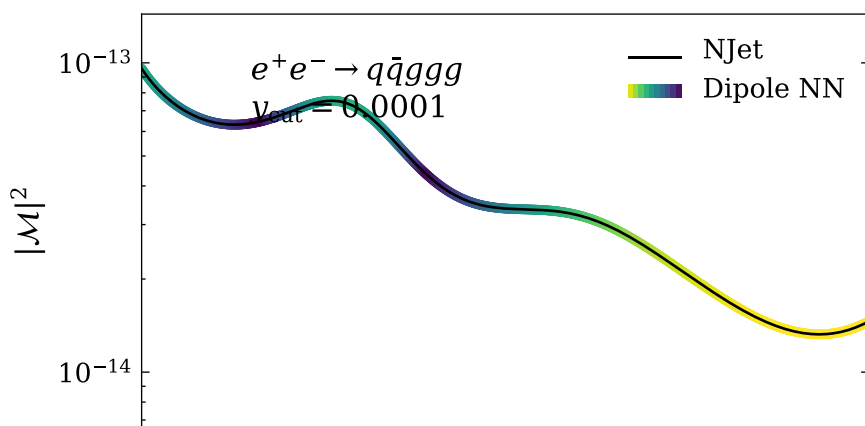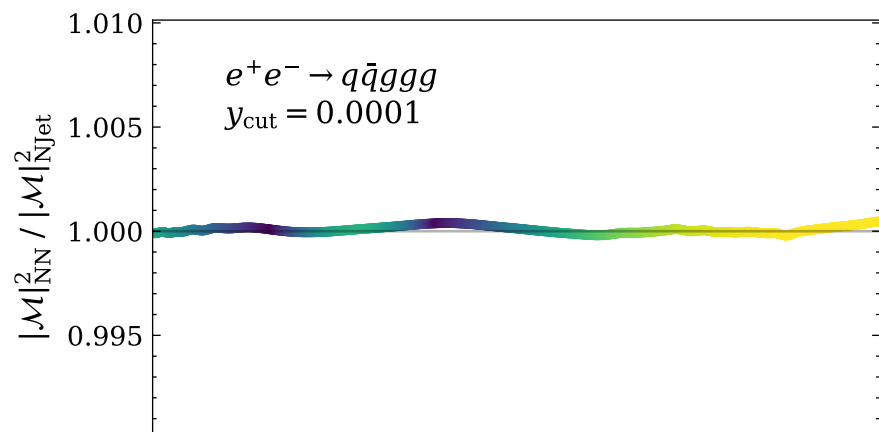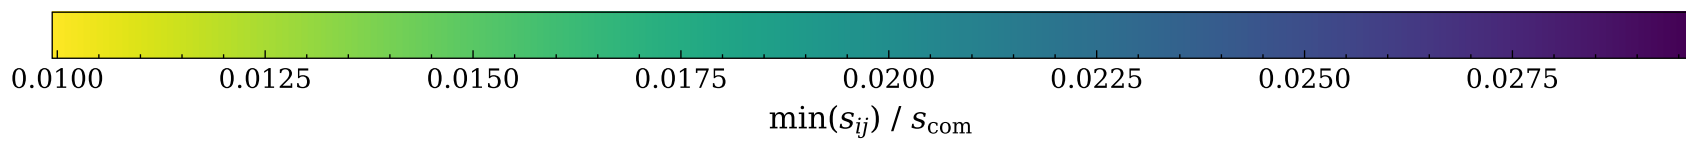

Trajectory 1281

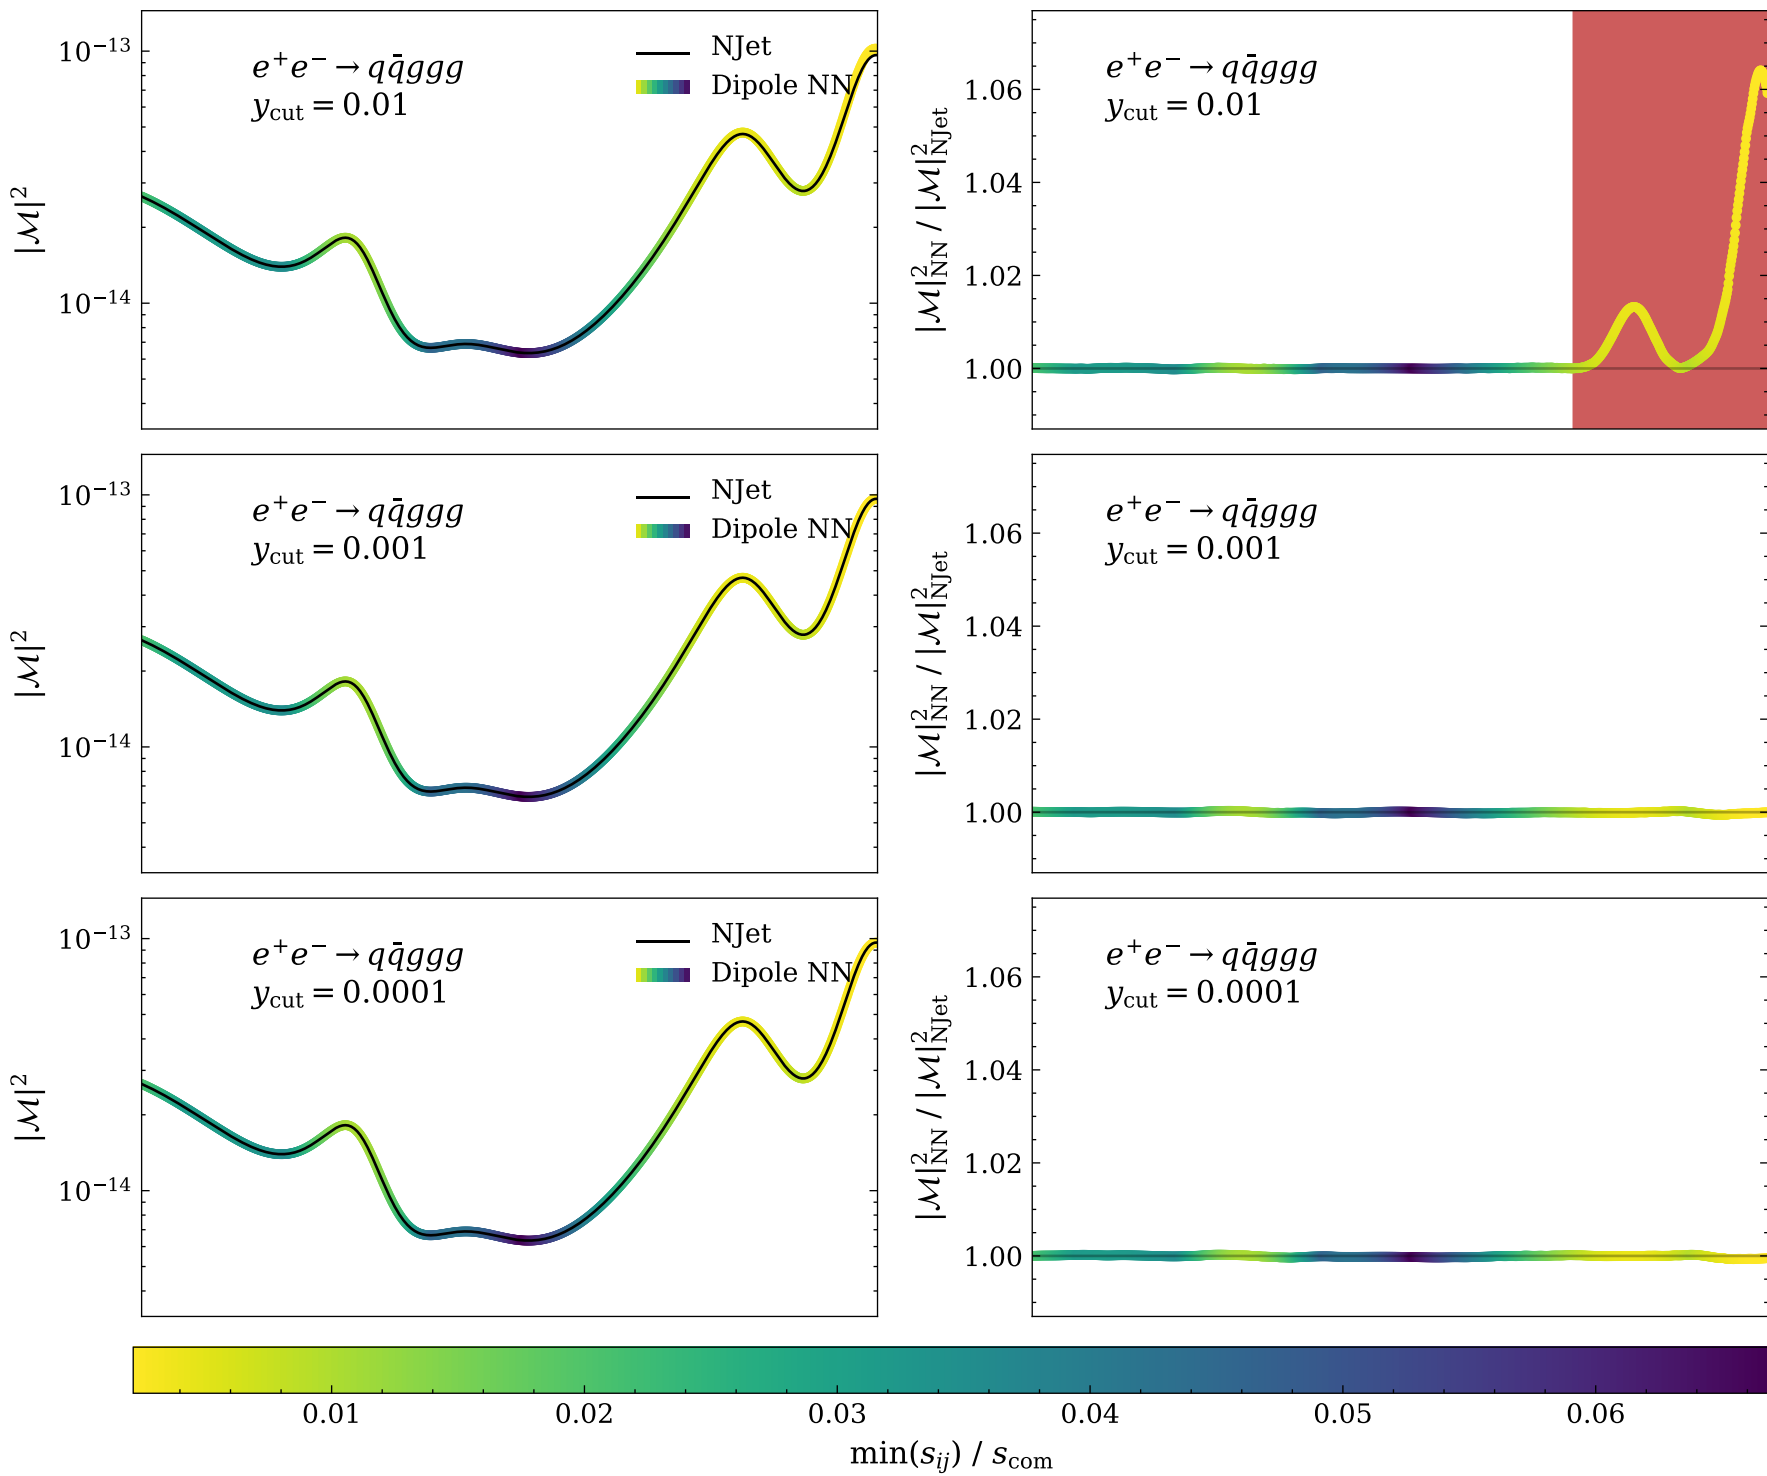

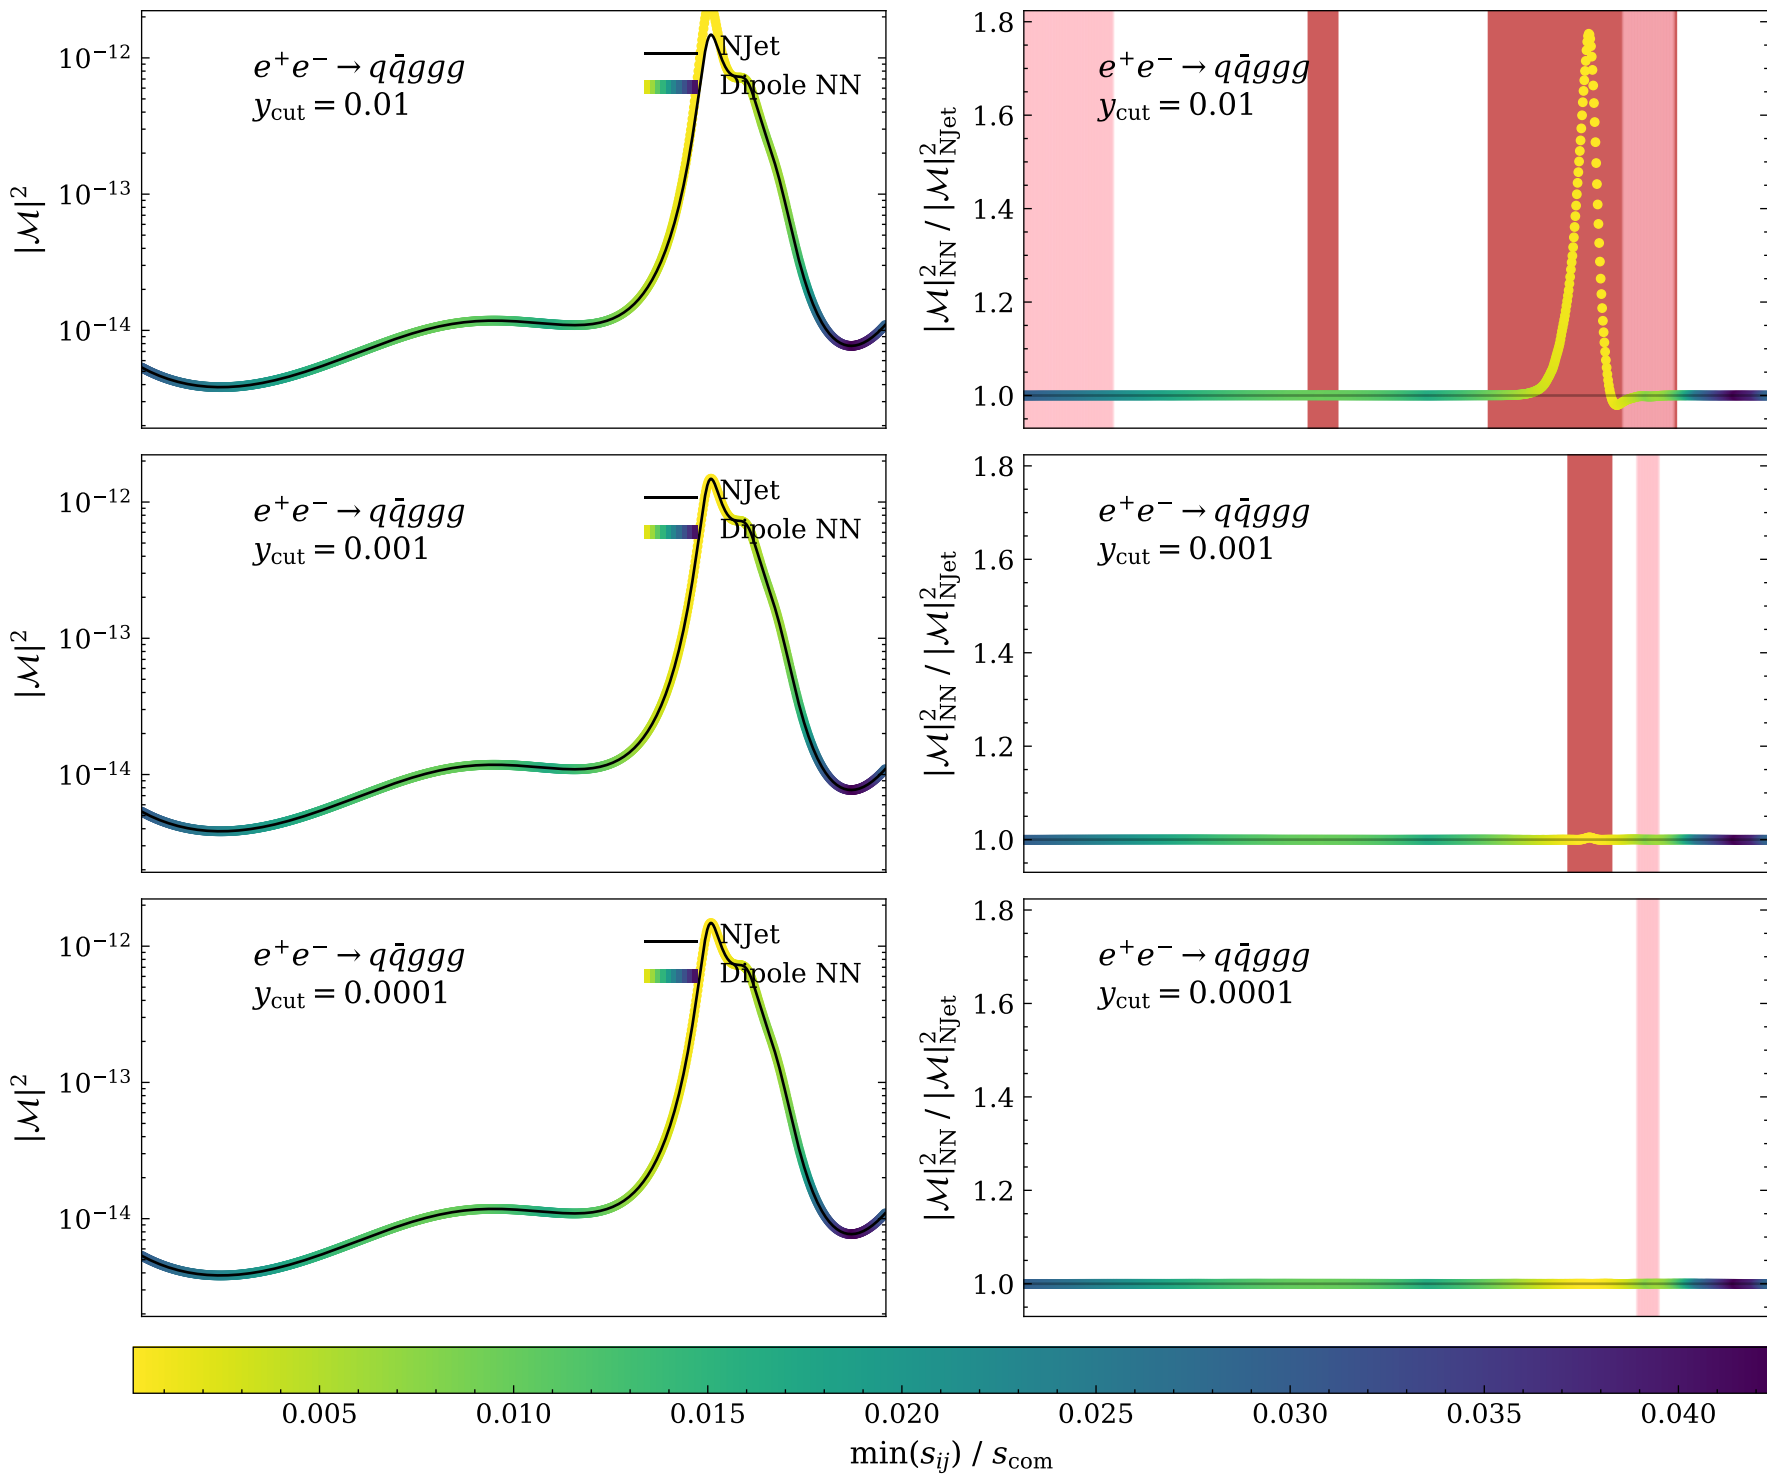

Trajectory 1283

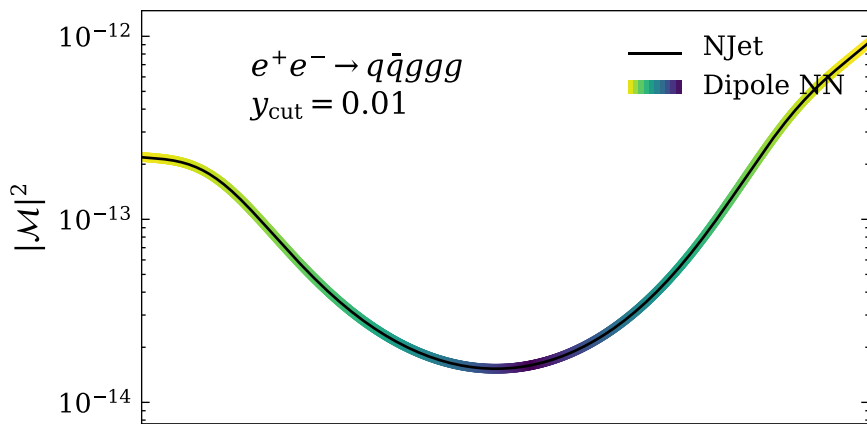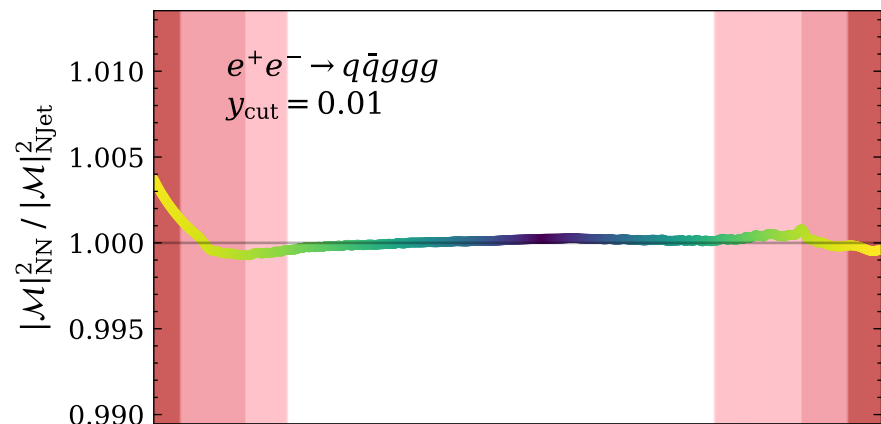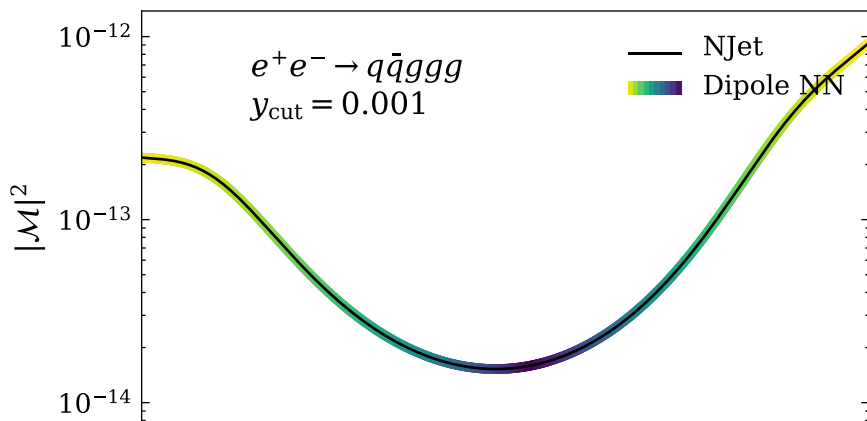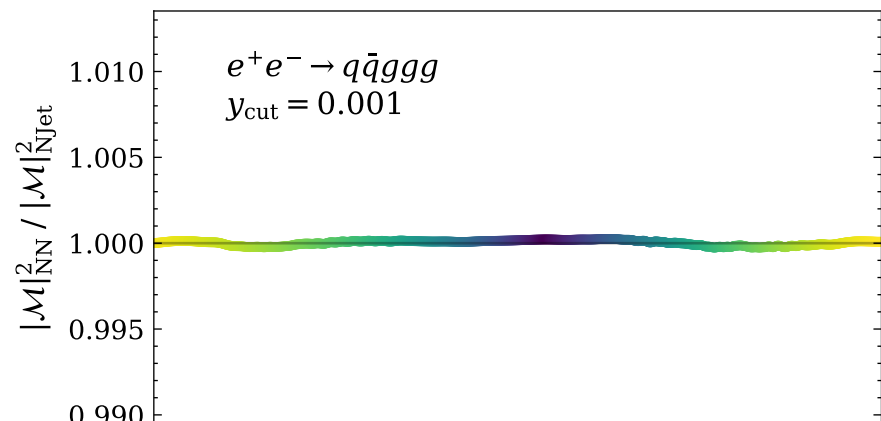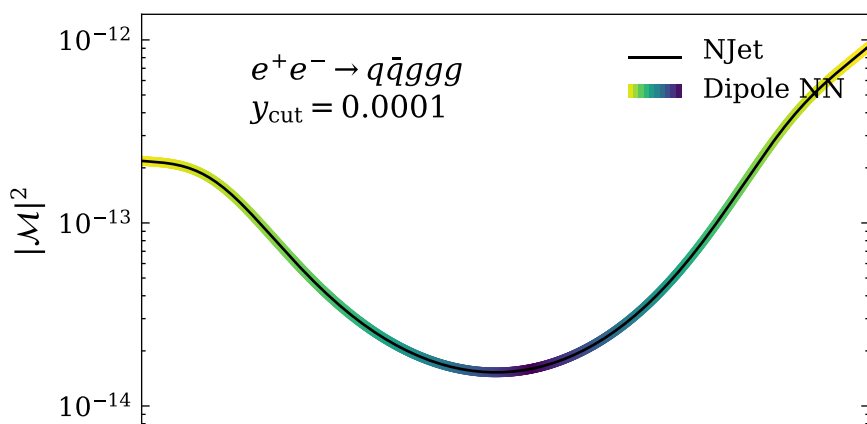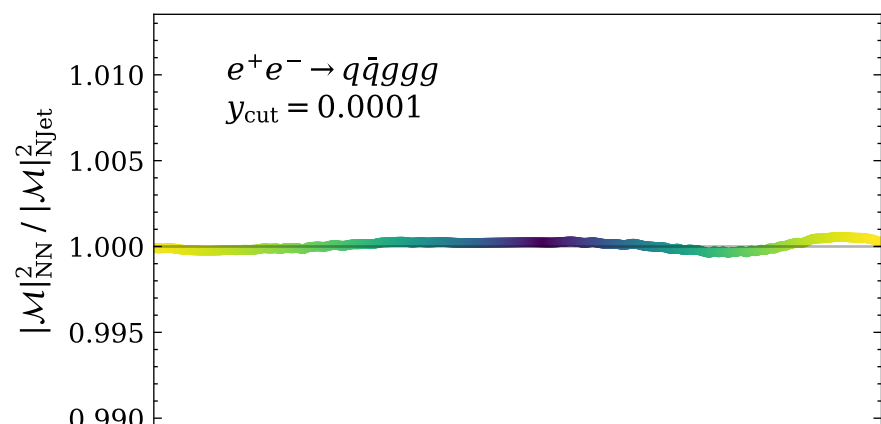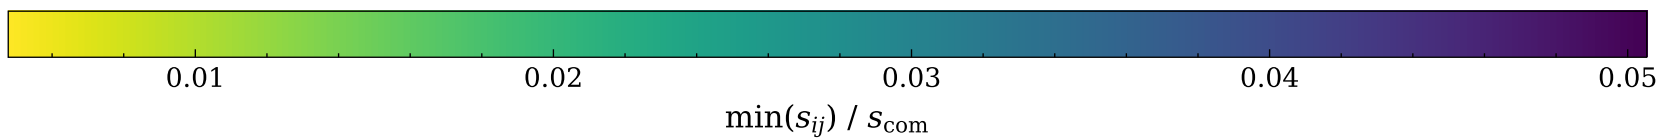

Supplement: Supplementary file 1 [file trajectories_panel.pdf]
